# Supplementary material for: Temporal stability in human interaction networks
Source: arXiv:1310.7769 ancillary file (2017-10-29)
Supplement: Supplementary file 1 [file supportingInformation.pdf]

# Temporal stability in human interaction networks: sector sizes, topological prominence and time activity (Supporting Information)

Renato Fabbri[1, a)]
*São Carlos Institute of Physics, University of São Paulo (IFSC/USP)*

(Dated: 21 August 2015)

## CONTENTS


I. Time activity in different scales 1
  A. Time circular measures 1
  B. Time histograms 3
    1. Histograms of activity along the hours of the day 3
    2. Histograms of activity along the days of the week 5
    3. Histograms of activity along the days of the month 5
    4. Histograms of activity along months of the year 7

II. PCA of measures along the timeline 7
  A. Betweenness, clustering and degree 7
  B. Betweenness, clustering, degrees and strengths 8
  C. Betweenness, clustering, degrees, strengths and symmetry measures 8

III. Fraction of participants in each Erdös Sector along the timeline 10
  A. CPP list 10
  B. LAD list 25

IV. Stability in other networks: Twitter, Facebook, Participa.br 40


The supporting information (this document) contains statistics for time activity (circular statistics and histograms) in Section I, the fraction of vertices in the peripheral, intermediary and hub sectors in Section III and the combination of basic topological measures into principal components with greater variance in Section II. There is a focus on email list interaction networks for benchmarking and Section IV reinforces the results with the analysis of networks from Facebook, Twitter and Participa.br. More context (e.g. methods, discussion, data and scripts) is given in the main document[1].

## I. TIME ACTIVITY IN DIFFERENT SCALES

Here we complement the theory presented in Section III A and results in Section IV A of the paper[1].

### A. Time circular measures

The measurements used were the rescaled circular mean $\theta'_\mu$, standard deviation $S(z)$, variance $Var(z)$, circular dispersion $\delta(z)$ and the relation of maximum and minimum incidence $\frac{max(incidence)}{min(incidence)}$ at each time unit. Also, $\mu_{\frac{max(incidence')}{min(incidence')}}$ and $\sigma_{\frac{max(incidence')}{min(incidence')}}$ are given for 1000 uniform distribution simulations within the same number of bins and with the same number of samples. Greater dispersion is found on seconds and minutes, followed by days of the month. Greater localization if found in the hours of the day, followed by weekdays and months.

a) http://ifsc.usp.br/~fabbri/; Electronic mail: fabbri@usp.br

TABLE S1. LAU circular measurements.

| scale | $\theta'_\mu$ | $S(z)$ | $Var(z)$ | $\delta(z)$ | $\frac{max(incidence)}{min(incidence)}$ | $\mu\,\frac{max(incidence')}{min(incidence')}$ | $\sigma\,\frac{max(incidence')}{min(incidence')}$ |
|---|---|---|---|---|---|---|---|
| seconds | $-//-$ | 3.31 | 1.00 | 29337.65 | 1.27 | 1.29 | 0.04 |
| minutes | $-//-$ | 3.13 | 0.99 | 8879.19 | 1.32 | 1.29 | 0.04 |
| hours | -8.76 | 1.56 | 0.71 | 4.92 | 8.38 | 1.14 | 0.03 |
| weekdays | -0.21 | 2.14 | 0.90 | 45.41 | 1.62 | 1.05 | 0.02 |
| month days | -0.64 | 2.76 | 0.98 | 1001.75 | 1.49 | 1.17 | 0.03 |
| months | 3.55 | 2.30 | 0.93 | 94.53 | 1.57 | 1.09 | 0.02 |

TABLE S2. LAD circular measurements.

| scale | $\theta'_\mu$ | $S(z)$ | $Var(z)$ | $\delta(z)$ | $\frac{max(incidence)}{min(incidence)}$ | $\mu\,\frac{max(incidence')}{min(incidence')}$ | $\sigma\,\frac{max(incidence')}{min(incidence')}$ |
|---|---|---|---|---|---|---|---|
| seconds | $-//-$ | 3.13 | 0.99 | 9070.17 | 1.28 | 1.29 | 0.05 |
| minutes | $-//-$ | 3.60 | 1.00 | 205489.40 | 1.22 | 1.29 | 0.05 |
| hours | -9.61 | 1.52 | 0.68 | 4.36 | 9.77 | 1.14 | 0.03 |
| weekdays | -0.03 | 2.03 | 0.87 | 29.28 | 1.72 | 1.05 | 0.02 |
| month days | -2.65 | 2.93 | 0.99 | 2657.77 | 1.50 | 1.17 | 0.03 |
| months | -0.56 | 2.14 | 0.90 | 44.00 | 2.25 | 1.09 | 0.02 |

TABLE S3. MET circular measurements.

| scale | $\theta'_\mu$ | $S(z)$ | $Var(z)$ | $\delta(z)$ | $\frac{max(incidence)}{min(incidence)}$ | $\mu\,\frac{max(incidence')}{min(incidence')}$ | $\sigma\,\frac{max(incidence')}{min(incidence')}$ |
|---|---|---|---|---|---|---|---|
| seconds | $-//-$ | 3.06 | 0.99 | 5910.47 | 1.27 | 1.29 | 0.04 |
| minutes | $-//-$ | 3.14 | 0.99 | 9696.29 | 1.34 | 1.29 | 0.04 |
| hours | -9.20 | 1.35 | 0.60 | 2.76 | 19.26 | 1.14 | 0.03 |
| weekdays | -0.27 | 1.86 | 0.82 | 13.82 | 2.89 | 1.05 | 0.02 |
| month days | 3.58 | 2.49 | 0.95 | 237.30 | 1.55 | 1.17 | 0.03 |
| months | -2.92 | 1.73 | 0.78 | 9.20 | 3.04 | 1.09 | 0.02 |

TABLE S4. CPP circular measurements.

| scale | $\theta'_\mu$ | $S(z)$ | $Var(z)$ | $\delta(z)$ | $\frac{max(incidence)}{min(incidence)}$ | $\mu\,\frac{max(incidence')}{min(incidence')}$ | $\sigma\,\frac{max(incidence')}{min(incidence')}$ |
|---|---|---|---|---|---|---|---|
| seconds | $-//-$ | 3.31 | 1.00 | 28205.46 | 1.26 | 1.29 | 0.04 |
| minutes | $-//-$ | 3.18 | 0.99 | 12275.59 | 1.27 | 1.29 | 0.04 |
| hours | -9.39 | 1.48 | 0.67 | 3.91 | 11.18 | 1.15 | 0.03 |
| weekdays | -0.17 | 1.83 | 0.81 | 12.66 | 2.59 | 1.05 | 0.02 |
| month days | -10.12 | 3.16 | 0.99 | 10789.17 | 1.54 | 1.17 | 0.03 |
| months | 0.15 | 2.34 | 0.93 | 115.49 | 1.50 | 1.08 | 0.02 |

## B. Time histograms

### 1. Histograms of activity along the hours of the day

Higher activity was observed between noon and 6pm, followed by the time period between 6pm and midnight. Around 2/3 of the whole activity takes place from noon to midnight. The activity peak occurs around midday, with a slight skew toward one hour before noon.

TABLE S5. LAU activity along the hours of the day.

| | 1h | 2h | 3h | 4h | 6h | 12h |
|---|---|---|---|---|---|---|
| 0h | 3.58 | 5.80 | 7.43 | 8.49 | 10.14 | 36.88 |
| 1h | 2.22 | | | | | |
| 2h | 1.63 | 2.69 | | | | |
| 3h | 1.06 | | 2.72 | | | |
| 4h | 0.84 | 1.66 | | 5.20 | | |
| 5h | 0.82 | | | | | |
| 6h | 1.17 | 3.54 | 7.07 | | 26.74 | |
| 7h | 2.37 | | | | | |
| 8h | 3.53 | 9.57 | | 23.20 | | |
| 9h | 6.04 | | 19.67 | | | |
| 10h | 6.83 | 13.62 | | | | |
| 11h | 6.79 | | | | | |
| 12h | 6.11 | 12.36 | 18.75 | 24.68 | 35.66 | 63.12 |
| 13h | 6.26 | | | | | |
| 14h | 6.38 | 12.31 | | | | |
| 15h | 5.93 | | 16.91 | | | |
| 16h | 5.52 | 10.98 | | 20.73 | | |
| 17h | 5.46 | | | | | |
| 18h | 5.23 | 9.75 | 14.30 | | 27.46 | |
| 19h | 4.52 | | | | | |
| 20h | 4.55 | 8.97 | | 17.71 | | |
| 21h | 4.42 | | 13.16 | | | |
| 22h | 4.51 | 8.74 | | | | |
| 23h | 4.23 | | | | | |

TABLE S6. LAD activity along the hours of the day.

| | 1h | 2h | 3h | 4h | 6h | 12h |
|---|---|---|---|---|---|---|
| 0h | 4.01 | 6.53 | 8.32 | 9.37 | 10.78 | 33.11 |
| 1h | 2.52 | | | | | |
| 2h | 1.79 | 2.84 | | | | |
| 3h | 1.06 | | 2.46 | | | |
| 4h | 0.75 | 1.40 | | 3.81 | | |
| 5h | 0.66 | | | | | |
| 6h | 0.85 | 2.41 | 5.36 | | 22.33 | |
| 7h | 1.56 | | | | | |
| 8h | 2.95 | 7.61 | | 19.93 | | |
| 9h | 4.66 | | 16.98 | | | |
| 10h | 5.92 | 12.32 | | | | |
| 11h | 6.40 | | | | | |
| 12h | 6.41 | 12.53 | 18.85 | 24.82 | 37.24 | 66.89 |
| 13h | 6.12 | | | | | |
| 14h | 6.32 | 12.29 | | | | |
| 15h | 5.97 | | 18.39 | | | |
| 16h | 6.40 | 12.42 | | 23.44 | | |
| 17h | 6.02 | | | | | |
| 18h | 5.99 | 11.02 | 15.65 | | 29.65 | |
| 19h | 5.03 | | | | | |
| 20h | 4.63 | 9.22 | | 18.63 | | |
| 21h | 4.59 | | 14.00 | | | |
| 22h | 4.88 | 9.41 | | | | |
| 23h | 4.53 | | | | | |

TABLE S7. MET activity along the hours of the day.

| | 1h | 2h | 3h | 4h | 6h | 12h |
|---|---|---|---|---|---|---|
| 0h | 2.87 | 4.64 | 5.67 | 6.31 | 7.15 | 29.33 |
| 1h | 1.77 | | | | | |
| 2h | 1.04 | 1.67 | | | | |
| 3h | 0.64 | | 1.48 | | | |
| 4h | 0.47 | 0.85 | | 2.89 | | |
| 5h | 0.38 | | | | | |
| 6h | 0.72 | 2.04 | 4.71 | | 22.18 | |
| 7h | 1.33 | | | | | |
| 8h | 2.67 | 7.07 | | 20.14 | | |
| 9h | 4.40 | | 17.47 | | | |
| 10h | 6.29 | 13.07 | | | | |
| 11h | 6.78 | | | | | |
| 12h | 7.33 | 14.41 | 21.50 | 28.65 | 42.22 | 70.67 |
| 13h | 7.08 | | | | | |
| 14h | 7.09 | 14.24 | | | | |
| 15h | 7.14 | | 20.72 | | | |
| 16h | 6.68 | 13.58 | | 24.79 | | |
| 17h | 6.89 | | | | | |
| 18h | 5.99 | 11.22 | 16.19 | | 28.44 | |
| 19h | 5.23 | | | | | |
| 20h | 4.98 | 9.34 | | 17.22 | | |
| 21h | 4.37 | | 12.25 | | | |
| 22h | 4.24 | 7.88 | | | | |
| 23h | 3.64 | | | | | |

TABLE S8. CPP activity along the hours of the day.

| | 1h | 2h | 3h | 4h | 6h | 12h |
|---|---|---|---|---|---|---|
| 0h | 3.66 | 6.42 | 8.20 | 9.30 | 10.67 | 33.76 |
| 1h | 2.76 | | | | | |
| 2h | 1.79 | 2.88 | | | | |
| 3h | 1.10 | | 2.47 | | | |
| 4h | 0.68 | 1.37 | | 3.44 | | |
| 5h | 0.69 | | | | | |
| 6h | 0.83 | 2.07 | 4.35 | | 23.09 | |
| 7h | 1.24 | | | | | |
| 8h | 2.28 | 6.80 | | 21.03 | | |
| 9h | 4.52 | | 18.75 | | | |
| 10h | 6.62 | 14.23 | | | | |
| 11h | 7.61 | | | | | |
| 12h | 6.44 | 12.48 | 18.95 | 25.05 | 37.63 | 66.24 |
| 13h | 6.04 | | | | | |
| 14h | 6.47 | 12.57 | | | | |
| 15h | 6.10 | | 18.68 | | | |
| 16h | 6.22 | 12.58 | | 23.60 | | |
| 17h | 6.36 | | | | | |
| 18h | 6.01 | 11.02 | 15.88 | | 28.61 | |
| 19h | 5.02 | | | | | |
| 20h | 4.85 | 9.23 | | 17.59 | | |
| 21h | 4.38 | | 12.73 | | | |
| 22h | 4.06 | 8.36 | | | | |
| 23h | 4.30 | | | | | |

### 2. Histograms of activity along the days of the week

Most notably, a decrease of activity on weekends of at least one third and at most two thirds.

| | Mon | Tue | Wed | Thu | Fri | Sat | Sun |
|---|---|---|---|---|---|---|---|
| LAU | 15.71 | 15.81 | 15.88 | 16.43 | 15.14 | 10.13 | 10.91 |
| LAD | 14.92 | 17.75 | 17.01 | 15.41 | 14.21 | 10.40 | 10.31 |
| MET | 17.53 | 17.54 | 16.43 | 17.06 | 17.46 | 7.92 | 6.06 |
| CPP | 17.06 | 17.43 | 17.61 | 17.13 | 16.30 | 6.81 | 7.67 |

### 3. Histograms of activity along the days of the month

The most important feature seems to be the homogeneity made explicit by the high circular dispersion in the tables of Section I A. Slightly higher activity rates are found in the beginning of the month, although not statistically significant.

TABLE S9. LAU activity along the days of the month.

<table>
<tr><th></th><th>1 day</th><th>5</th><th>10</th><th>15 days</th></tr>
<tr><td>1</td><td>3.36</td><td rowspan="5">16.21</td><td rowspan="10">33.71</td><td rowspan="15">50.82</td></tr>
<tr><td>2</td><td>3.43</td></tr>
<tr><td>3</td><td>3.31</td></tr>
<tr><td>4</td><td>3.37</td></tr>
<tr><td>5</td><td>2.75</td></tr>
<tr><td>6</td><td>3.03</td><td rowspan="5">17.50</td></tr>
<tr><td>7</td><td>3.93</td></tr>
<tr><td>8</td><td>3.62</td></tr>
<tr><td>9</td><td>3.84</td></tr>
<tr><td>10</td><td>3.09</td></tr>
<tr><td>11</td><td>3.20</td><td rowspan="5">17.11</td><td rowspan="10">34.02</td></tr>
<tr><td>12</td><td>3.40</td></tr>
<tr><td>13</td><td>3.67</td></tr>
<tr><td>14</td><td>3.71</td></tr>
<tr><td>15</td><td>3.14</td></tr>
<tr><td>16</td><td>3.08</td><td rowspan="5">16.91</td><td rowspan="15">49.18</td></tr>
<tr><td>17</td><td>3.13</td></tr>
<tr><td>18</td><td>3.43</td></tr>
<tr><td>19</td><td>3.61</td></tr>
<tr><td>20</td><td>3.67</td></tr>
<tr><td>21</td><td>3.60</td><td rowspan="5">15.43</td><td rowspan="10">32.27</td></tr>
<tr><td>22</td><td>3.42</td></tr>
<tr><td>23</td><td>2.80</td></tr>
<tr><td>24</td><td>2.64</td></tr>
<tr><td>25</td><td>2.97</td></tr>
<tr><td>26</td><td>3.06</td><td rowspan="5">16.85</td></tr>
<tr><td>27</td><td>2.69</td></tr>
<tr><td>28</td><td>3.79</td></tr>
<tr><td>29</td><td>3.75</td></tr>
<tr><td>30</td><td>3.57</td></tr>
</table>

TABLE S10. LAD activity along the days of the month.

<table>
<tr><th></th><th>1 day</th><th>5</th><th>10</th><th>15 days</th></tr>
<tr><td>1</td><td>3.29</td><td rowspan="5">15.77</td><td rowspan="10">33.63</td><td rowspan="15">50.50</td></tr>
<tr><td>2</td><td>3.38</td></tr>
<tr><td>3</td><td>2.85</td></tr>
<tr><td>4</td><td>2.94</td></tr>
<tr><td>5</td><td>3.31</td></tr>
<tr><td>6</td><td>3.60</td><td rowspan="5">17.85</td></tr>
<tr><td>7</td><td>2.68</td></tr>
<tr><td>8</td><td>3.78</td></tr>
<tr><td>9</td><td>3.88</td></tr>
<tr><td>10</td><td>3.91</td></tr>
<tr><td>11</td><td>3.22</td><td rowspan="5">16.87</td><td rowspan="10">33.41</td></tr>
<tr><td>12</td><td>2.79</td></tr>
<tr><td>13</td><td>3.50</td></tr>
<tr><td>14</td><td>3.95</td></tr>
<tr><td>15</td><td>3.40</td></tr>
<tr><td>16</td><td>3.32</td><td rowspan="5">16.54</td><td rowspan="15">49.50</td></tr>
<tr><td>17</td><td>2.95</td></tr>
<tr><td>18</td><td>3.50</td></tr>
<tr><td>19</td><td>3.69</td></tr>
<tr><td>20</td><td>3.07</td></tr>
<tr><td>21</td><td>2.76</td><td rowspan="5">15.71</td><td rowspan="10">32.96</td></tr>
<tr><td>22</td><td>3.35</td></tr>
<tr><td>23</td><td>3.32</td></tr>
<tr><td>24</td><td>3.15</td></tr>
<tr><td>25</td><td>3.13</td></tr>
<tr><td>26</td><td>3.68</td><td rowspan="5">17.25</td></tr>
<tr><td>27</td><td>4.02</td></tr>
<tr><td>28</td><td>3.49</td></tr>
<tr><td>29</td><td>3.34</td></tr>
<tr><td>30</td><td>2.72</td></tr>
</table>

TABLE S11. MET activity along the days of the month.

| | 1 day | 5 | 10 | 15 days |
|---|---|---|---|---|
| 1 | 3.05 | | | |
| 2 | 3.38 | | | |
| 3 | 3.62 | 18.25 | | |
| 4 | 4.25 | | | |
| 5 | 3.94 | | 35.24 | |
| 6 | 3.73 | | | |
| 7 | 3.17 | | | |
| 8 | 3.26 | 16.98 | | 50.96 |
| 9 | 3.56 | | | |
| 10 | 3.26 | | | |
| 11 | 3.81 | | | |
| 12 | 2.91 | | | |
| 13 | 3.30 | 15.73 | | |
| 14 | 2.75 | | | |
| 15 | 2.95 | | 31.98 | |
| 16 | 3.36 | | | |
| 17 | 3.16 | | | |
| 18 | 3.44 | 16.25 | | |
| 19 | 3.36 | | | |
| 20 | 2.93 | | | |
| 21 | 3.20 | | | |
| 22 | 3.11 | | | |
| 23 | 3.60 | 15.79 | | 49.04 |
| 24 | 2.74 | | | |
| 25 | 3.13 | | 32.78 | |
| 26 | 3.13 | | | |
| 27 | 3.07 | | | |
| 28 | 3.61 | 16.99 | | |
| 29 | 3.60 | | | |
| 30 | 3.57 | | | |

TABLE S12. CPP activity along the days of the month.

| | 1 day | 5 | 10 | 15 days |
|---|---|---|---|---|
| 1 | 3.22 | | | |
| 2 | 3.08 | | | |
| 3 | 3.19 | 15.98 | | |
| 4 | 3.65 | | | |
| 5 | 2.84 | | 31.82 | |
| 6 | 3.65 | | | |
| 7 | 3.53 | | | |
| 8 | 3.10 | 15.84 | | 49.62 |
| 9 | 2.49 | | | |
| 10 | 3.07 | | | |
| 11 | 3.47 | | | |
| 12 | 3.26 | | | |
| 13 | 3.55 | 17.80 | | |
| 14 | 3.84 | | | |
| 15 | 3.68 | | 34.22 | |
| 16 | 3.74 | | | |
| 17 | 3.40 | | | |
| 18 | 3.41 | 16.42 | | |
| 19 | 2.95 | | | |
| 20 | 2.93 | | | |
| 21 | 3.15 | | | |
| 22 | 3.64 | | | |
| 23 | 3.51 | 17.13 | | 50.38 |
| 24 | 3.32 | | | |
| 25 | 3.51 | | 33.96 | |
| 26 | 3.54 | | | |
| 27 | 3.21 | | | |
| 28 | 3.40 | 16.84 | | |
| 29 | 3.83 | | | |
| 30 | 2.86 | | | |

### 4. Histograms of activity along months of the year

Activity is concentrated in Jun-Aug and/or in Dec-Mar. These observations mostly fit academic calendars, vacations and end-of-year holidays.

TABLE S13. LAU activity along the months of the year.

| | m. | b. | t. | q. | s. |
|---|---|---|---|---|---|
| Jan | 10.22 | 19.56 | 28.24 | 35.09 | 49.16 |
| Fev | 9.34 | | | | |
| Mar | 8.67 | 15.53 | | | |
| Apr | 6.86 | | 20.93 | | |
| Mai | 7.28 | 14.07 | | 30.36 | |
| Jun | 6.80 | | | | |
| Jul | 8.97 | 16.29 | 24.47 | | 50.84 |
| Ago | 7.32 | | | | |
| Set | 8.18 | 16.25 | | 34.55 | |
| Out | 8.06 | | 26.36 | | |
| Nov | 7.64 | 18.30 | | | |
| Dez | 10.66 | | | | |

TABLE S14. LAD activity along the months of the year.

| | m. | b. | t. | q. | s. |
|---|---|---|---|---|---|
| Jan | 11.24 | 18.51 | 26.46 | 36.07 | 57.96 |
| Fev | 7.26 | | | | |
| Mar | 7.95 | 17.56 | | | |
| Apr | 9.61 | | 31.50 | | |
| Mai | 8.94 | 21.89 | | 37.56 | |
| Jun | 12.95 | | | | |
| Jul | 9.03 | 15.67 | 22.30 | | 42.04 |
| Ago | 6.64 | | | | |
| Set | 6.63 | 12.38 | | 26.37 | |
| Out | 5.75 | | 19.74 | | |
| Nov | 7.61 | 13.99 | | | |
| Dez | 6.38 | | | | |

TABLE S15. MET activity along the months of the year.

| | m. | b. | t. | q. | s. |
|---|---|---|---|---|---|
| Jan | 4.87 | 11.00 | 16.89 | 23.30 | 47.70 |
| Fev | 6.13 | | | | |
| Mar | 5.89 | 12.30 | | | |
| Apr | 6.41 | | 30.81 | | |
| Mai | 10.45 | 24.40 | | 47.87 | |
| Jun | 13.95 | | | | |
| Jul | 13.24 | 23.47 | 31.21 | | 52.30 |
| Ago | 10.22 | | | | |
| Set | 7.75 | 16.79 | | 28.83 | |
| Out | 9.04 | | 21.09 | | |
| Nov | 7.45 | 12.05 | | | |
| Dez | 4.59 | | | | |

TABLE S16. CPP activity along the months of the year.

| | m. | b. | t. | q. | s. |
|---|---|---|---|---|---|
| Jan | 8.70 | 17.00 | 27.23 | 36.49 | 54.27 |
| Fev | 8.29 | | | | |
| Mar | 10.23 | 19.49 | | | |
| Apr | 9.26 | | 27.03 | | |
| Mai | 9.41 | 17.78 | | 33.46 | |
| Jun | 8.37 | | | | |
| Jul | 8.70 | 15.68 | 22.94 | | 45.73 |
| Ago | 6.98 | | | | |
| Set | 7.26 | 15.36 | | 30.06 | |
| Out | 8.10 | | 22.80 | | |
| Nov | 7.89 | 14.69 | | | |
| Dez | 6.81 | | | | |

## II. PCA OF MEASURES ALONG THE TIMELINE

Loadings for the 14 metrics into the principal components are given for all LAD, LAU, MET, CPP, lists, $ws = 1000$ messages in 20 disjoint positioning. The clustering coefficient (cc) appears as the first metric in the tables, followed by 7 centrality metrics and 6 symmetry-related metrics. The centrality metrics, including degrees, strength and betweenness centrality, are the most important contributors for the first principal component, while the second component is dominated by symmetry metrics. The clustering coefficient is only relevant for the third principal component, coupled with standard deviations of strengths and degrees. The three components have in average 80.36% of the variance. Further details are given in Sections III C 1 and IV B of the main document[1].

### A. Betweenness, clustering and degree

TABLE S17. LAU principal components formation and concentration of dispersion.

| | PC1 | | PC2 | | PC3 | |
|---|---|---|---|---|---|---|
| | $\mu$ | $\sigma$ | $\mu$ | $\sigma$ | $\mu$ | $\sigma$ |
| $cc$ | 6.03 | 3.73 | 87.60 | 5.25 | 4.52 | 0.93 |
| $k$ | 47.13 | 1.76 | 3.01 | 1.98 | 47.90 | 0.38 |
| $bt$ | 46.84 | 1.97 | 9.39 | 4.31 | 47.58 | 0.57 |
| $\lambda$ | 64.99 | 0.60 | 33.08 | 0.41 | 1.93 | 0.36 |

TABLE S18. LAD principal components formation and concentration of dispersion.

| | PC1 | | PC2 | | PC3 | |
|---|---|---|---|---|---|---|
| | $\mu$ | $\sigma$ | $\mu$ | $\sigma$ | $\mu$ | $\sigma$ |
| $cc$ | 6.42 | 4.05 | 86.60 | 5.50 | 5.19 | 1.45 |
| $k$ | 46.98 | 1.86 | 2.95 | 1.65 | 47.61 | 0.57 |
| $bt$ | 46.59 | 2.18 | 10.45 | 4.72 | 47.20 | 0.90 |
| $\lambda$ | 64.96 | 0.71 | 33.08 | 0.41 | 1.96 | 0.52 |

TABLE S19. MET principal components formation and concentration of dispersion.

| | PC1 | | PC2 | | PC3 | |
|---|---|---|---|---|---|---|
| | $\mu$ | $\sigma$ | $\mu$ | $\sigma$ | $\mu$ | $\sigma$ |
| $cc$ | 5.82 | 3.76 | 87.26 | 5.12 | 4.93 | 1.19 |
| $k$ | 47.18 | 1.82 | 4.35 | 4.01 | 47.63 | 0.57 |
| $bt$ | 47.01 | 1.96 | 8.40 | 4.22 | 47.44 | 0.67 |
| $\lambda$ | 64.94 | 0.76 | 33.13 | 0.45 | 1.93 | 0.62 |

TABLE S20. CPP principal components formation and concentration of dispersion.

| | PC1 | | PC2 | | PC3 | |
|---|---|---|---|---|---|---|
| | $\mu$ | $\sigma$ | $\mu$ | $\sigma$ | $\mu$ | $\sigma$ |
| $cc$ | 3.61 | 2.13 | 91.86 | 3.24 | 3.59 | 0.98 |
| $k$ | 48.24 | 0.99 | 2.96 | 2.25 | 48.25 | 0.43 |
| $bt$ | 48.15 | 1.14 | 5.18 | 3.89 | 48.16 | 0.56 |
| $\lambda$ | 65.24 | 0.51 | 33.30 | 0.17 | 1.46 | 0.49 |

### B. Betweenness, clustering, degrees and strengths

TABLE S21. LAU principal components formation and concentration of dispersion.

| | PC1 | | PC2 | | PC3 | |
|---|---|---|---|---|---|---|
| | $\mu$ | $\sigma$ | $\mu$ | $\sigma$ | $\mu$ | $\sigma$ |
| $cc$ | 1.59 | 0.81 | 80.37 | 5.18 | 3.09 | 1.89 |
| $s$ | 14.40 | 0.15 | 0.81 | 0.68 | 4.75 | 4.43 |
| $s^{in}$ | 14.00 | 0.14 | 2.32 | 1.49 | 18.98 | 4.93 |
| $s^{out}$ | 13.96 | 0.14 | 2.72 | 1.44 | 18.25 | 6.36 |
| $k$ | 14.49 | 0.15 | 0.54 | 0.35 | 1.37 | 0.98 |
| $k^{in}$ | 14.01 | 0.13 | 2.72 | 1.35 | 18.69 | 5.01 |
| $k^{out}$ | 13.85 | 0.13 | 2.37 | 1.73 | 22.63 | 3.79 |
| $bt$ | 13.69 | 0.22 | 8.16 | 1.62 | 12.23 | 8.33 |
| $\lambda$ | 81.87 | 0.88 | 12.48 | 0.15 | 3.33 | 0.70 |

TABLE S22. LAD principal components formation and concentration of dispersion.

| | PC1 | | PC2 | | PC3 | |
|---|---|---|---|---|---|---|
| | $\mu$ | $\sigma$ | $\mu$ | $\sigma$ | $\mu$ | $\sigma$ |
| $cc$ | 1.83 | 1.11 | 80.38 | 11.45 | 3.78 | 4.43 |
| $s$ | 14.25 | 0.17 | 1.34 | 1.81 | 9.88 | 5.76 |
| $s^{in}$ | 13.99 | 0.19 | 2.06 | 1.70 | 17.62 | 6.15 |
| $s^{out}$ | 14.03 | 0.22 | 1.81 | 1.98 | 15.44 | 6.68 |
| $k$ | 14.38 | 0.13 | 0.95 | 1.64 | 3.45 | 3.15 |
| $k^{in}$ | 14.05 | 0.14 | 2.26 | 1.66 | 13.44 | 7.26 |
| $k^{out}$ | 13.96 | 0.15 | 1.72 | 1.53 | 16.14 | 6.37 |
| $bt$ | 13.51 | 0.35 | 9.48 | 2.86 | 20.26 | 9.87 |
| $\lambda$ | 82.32 | 1.61 | 12.52 | 0.26 | 2.97 | 1.21 |

TABLE S23. MET principal components formation and concentration of dispersion.

| | PC1 | | PC2 | | PC3 | |
|---|---|---|---|---|---|---|
| | $\mu$ | $\sigma$ | $\mu$ | $\sigma$ | $\mu$ | $\sigma$ |
| $cc$ | 1.16 | 0.76 | 81.72 | 3.00 | 1.61 | 1.78 |
| $s$ | 14.32 | 0.16 | 1.76 | 1.12 | 11.39 | 5.50 |
| $s^{in}$ | 14.17 | 0.11 | 2.29 | 1.29 | 14.46 | 3.72 |
| $s^{out}$ | 14.09 | 0.17 | 1.72 | 1.18 | 17.54 | 5.37 |
| $k$ | 14.39 | 0.16 | 1.73 | 0.63 | 4.76 | 2.82 |
| $k^{in}$ | 14.12 | 0.13 | 1.02 | 0.71 | 11.69 | 6.93 |
| $k^{out}$ | 14.06 | 0.13 | 3.11 | 1.58 | 12.18 | 9.24 |
| $bt$ | 13.69 | 0.26 | 6.64 | 2.01 | 26.37 | 12.37 |
| $\lambda$ | 83.41 | 1.53 | 12.53 | 0.11 | 2.34 | 1.16 |

TABLE S24. CPP principal components formation and concentration of dispersion.

| | PC1 | | PC2 | | PC3 | |
|---|---|---|---|---|---|---|
| | $\mu$ | $\sigma$ | $\mu$ | $\sigma$ | $\mu$ | $\sigma$ |
| $cc$ | 0.84 | 0.61 | 80.59 | 6.89 | 2.30 | 2.19 |
| $s$ | 14.28 | 0.07 | 0.97 | 1.03 | 15.89 | 1.15 |
| $s^{in}$ | 14.18 | 0.12 | 2.89 | 1.71 | 13.50 | 5.19 |
| $s^{out}$ | 14.07 | 0.23 | 2.83 | 1.63 | 18.80 | 4.94 |
| $k$ | 14.42 | 0.08 | 0.78 | 0.67 | 7.48 | 2.71 |
| $k^{in}$ | 14.29 | 0.10 | 2.36 | 1.41 | 7.21 | 4.49 |
| $k^{out}$ | 14.16 | 0.12 | 3.62 | 1.83 | 8.79 | 4.58 |
| $bt$ | 13.76 | 0.22 | 5.96 | 1.88 | 26.03 | 7.94 |
| $\lambda$ | 83.32 | 1.42 | 12.60 | 0.08 | 2.61 | 1.15 |

### C. Betweenness, clustering, degrees, strengths and symmetry measures

TABLE S25. LAU principal components formation and concentration of dispersion.

| | PC1 | | PC2 | | PC3 | |
|---|---|---|---|---|---|---|
| | $\mu$ | $\sigma$ | $\mu$ | $\sigma$ | $\mu$ | $\sigma$ |
| $cc$ | 1.64 | 0.77 | 2.42 | 1.71 | 19.20 | 3.96 |
| $s$ | 12.80 | 0.46 | 0.89 | 0.82 | 2.53 | 0.63 |
| $s^{in}$ | 12.47 | 0.42 | 2.30 | 0.97 | 2.29 | 0.81 |
| $s^{out}$ | 12.37 | 0.46 | 2.89 | 1.24 | 2.64 | 0.58 |
| $k$ | 12.93 | 0.44 | 0.82 | 0.73 | 1.32 | 0.45 |
| $k^{in}$ | 12.54 | 0.37 | 2.88 | 1.13 | 1.02 | 0.56 |
| $k^{out}$ | 12.32 | 0.46 | 3.82 | 1.14 | 1.57 | 0.68 |
| $bt$ | 12.19 | 0.46 | 1.06 | 0.62 | 2.64 | 0.89 |
| $asy$ | 0.93 | 0.81 | 20.38 | 0.82 | 1.66 | 1.09 |
| $\mu_{asy}$ | 0.96 | 0.83 | 20.26 | 0.82 | 1.66 | 1.04 |
| $\sigma_{asy}$ | 6.18 | 0.71 | 1.24 | 0.92 | 27.98 | 1.74 |
| $dis$ | 0.90 | 0.79 | 20.36 | 0.82 | 1.54 | 1.07 |
| $\mu_{dis}$ | 0.92 | 0.61 | 19.02 | 0.84 | 1.45 | 1.12 |
| $\sigma_{dis}$ | 0.86 | 0.51 | 1.64 | 1.10 | 32.51 | 1.90 |
| $\lambda$ | 48.41 | 0.52 | 27.95 | 0.36 | 12.81 | 0.79 |

TABLE S26. LAD principal components formation and concentration of dispersion.

| | PC1 | | PC2 | | PC3 | |
|---|---|---|---|---|---|---|
| | $\mu$ | $\sigma$ | $\mu$ | $\sigma$ | $\mu$ | $\sigma$ |
| $cc$ | 1.96 | 0.95 | 3.07 | 1.46 | 17.94 | 5.38 |
| $s$ | 12.34 | 0.57 | 1.72 | 0.99 | 2.43 | 0.93 |
| $s^{in}$ | 12.06 | 0.64 | 3.18 | 0.98 | 1.98 | 1.09 |
| $s^{out}$ | 12.22 | 0.48 | 1.14 | 0.78 | 2.83 | 0.79 |
| $k$ | 12.54 | 0.56 | 1.43 | 0.87 | 0.92 | 0.44 |
| $k^{in}$ | 12.15 | 0.61 | 3.81 | 0.79 | 0.61 | 0.42 |
| $k^{out}$ | 12.27 | 0.45 | 1.51 | 1.08 | 1.56 | 0.39 |
| $bt$ | 11.73 | 0.64 | 1.80 | 0.88 | 2.28 | 1.00 |
| $asy$ | 1.51 | 0.97 | 19.66 | 1.63 | 3.02 | 1.66 |
| $\mu_{asy}$ | 1.41 | 0.99 | 19.53 | 1.62 | 3.00 | 1.69 |
| $\sigma_{asy}$ | 5.62 | 0.68 | 2.01 | 1.23 | 27.46 | 3.31 |
| $dis$ | 1.58 | 0.98 | 19.57 | 1.65 | 3.21 | 1.71 |
| $\mu_{dis}$ | 1.84 | 1.00 | 18.62 | 1.52 | 2.08 | 1.13 |
| $\sigma_{dis}$ | 0.77 | 0.59 | 2.94 | 1.60 | 30.68 | 3.34 |
| $\lambda$ | 48.65 | 1.03 | 27.84 | 0.31 | 13.00 | 0.77 |

TABLE S27. MET principal components formation and concentration of dispersion.

| | PC1 | | PC2 | | PC3 | |
|---|---|---|---|---|---|---|
| | $\mu$ | $\sigma$ | $\mu$ | $\sigma$ | $\mu$ | $\sigma$ |
| $cc$ | 1.18 | 0.71 | 3.00 | 2.35 | 22.39 | 2.71 |
| $s$ | 12.34 | 0.66 | 1.74 | 1.17 | 1.55 | 0.75 |
| $s^{in}$ | 12.25 | 0.62 | 1.74 | 0.96 | 1.45 | 0.77 |
| $s^{out}$ | 12.11 | 0.72 | 2.42 | 1.35 | 1.78 | 0.78 |
| $k$ | 12.48 | 0.63 | 1.46 | 0.91 | 0.54 | 0.48 |
| $k^{in}$ | 12.32 | 0.56 | 1.54 | 1.22 | 0.65 | 0.62 |
| $k^{out}$ | 12.12 | 0.67 | 3.10 | 1.15 | 0.87 | 0.74 |
| $bt$ | 11.85 | 0.62 | 1.46 | 0.87 | 1.16 | 0.70 |
| $asy$ | 1.79 | 1.22 | 19.35 | 2.15 | 3.29 | 2.15 |
| $\mu_{asy}$ | 1.84 | 1.22 | 19.17 | 2.16 | 3.31 | 2.23 |
| $\sigma_{asy}$ | 4.17 | 0.79 | 3.91 | 2.35 | 27.79 | 3.96 |
| $dis$ | 1.78 | 1.18 | 19.26 | 2.15 | 3.38 | 2.29 |
| $\mu_{dis}$ | 1.53 | 1.10 | 18.23 | 2.12 | 3.32 | 1.71 |
| $\sigma_{dis}$ | 2.23 | 0.93 | 3.61 | 2.38 | 28.54 | 3.23 |
| $\lambda$ | 49.05 | 1.01 | 27.79 | 0.30 | 13.30 | 1.35 |

TABLE S28. CPP principal components formation and concentration of dispersion.

| | PC1 | | PC2 | | PC3 | |
|---|---|---|---|---|---|---|
| | $\mu$ | $\sigma$ | $\mu$ | $\sigma$ | $\mu$ | $\sigma$ |
| $cc$ | 0.89 | 0.59 | 1.93 | 1.33 | 21.22 | 2.97 |
| $s$ | 11.71 | 0.57 | 2.97 | 0.82 | 2.45 | 0.72 |
| $s^{in}$ | 11.68 | 0.58 | 2.37 | 0.91 | 3.08 | 0.78 |
| $s^{out}$ | 11.49 | 0.61 | 3.63 | 0.79 | 1.61 | 0.88 |
| $k$ | 11.93 | 0.54 | 2.58 | 0.70 | 0.52 | 0.44 |
| $k^{in}$ | 11.93 | 0.52 | 1.19 | 0.88 | 1.41 | 0.71 |
| $k^{out}$ | 11.57 | 0.61 | 4.34 | 0.70 | 0.98 | 0.66 |
| $bt$ | 11.37 | 0.55 | 2.44 | 0.84 | 1.37 | 0.77 |
| $asy$ | 3.14 | 0.98 | 18.52 | 1.97 | 2.46 | 1.69 |
| $\mu_{asy}$ | 3.32 | 0.99 | 18.23 | 2.01 | 2.80 | 1.82 |
| $\sigma_{asy}$ | 4.91 | 0.59 | 2.44 | 1.47 | 26.84 | 3.06 |
| $dis$ | 2.94 | 0.88 | 18.50 | 1.92 | 3.06 | 1.98 |
| $\mu_{dis}$ | 2.55 | 0.89 | 18.12 | 1.85 | 1.57 | 1.32 |
| $\sigma_{dis}$ | 0.57 | 0.33 | 2.74 | 1.63 | 30.61 | 2.66 |
| $\lambda$ | 49.56 | 1.16 | 27.14 | 0.54 | 13.25 | 0.95 |

## III. FRACTION OF PARTICIPANTS IN EACH ERDÖS SECTOR ALONG THE TIMELINE

Here we present the fraction of participants in each Erdös sector with respect to each criterion defined in Section III D of the main document[1]. Step sizes of 50, 100, 250, 500, 1000 and 5000 are shown below, first for CPP, then for LAD list.

Each step size takes two pages of plot. On the first page, the criterion is based on each centrality metric observed separately: in, out and total degrees and strengths. In the first six plots, the code for the colors is as follows: red for hubs, green for the fraction of intermediary vertices and blue for the peripheral fraction. On the last plot, red is the center (maximum distance to another vertex is equal to radius), blue is periphery (maximum distance equals to diameter) of the greatest component. On the same graph, green represents the disconnected vertices.

On the second page we show the fractions of participants with respect to each compound criterion for the Erdös sectioning. In the first plot, the fraction of vertices with unique classification is plotted in black: $\frac{\text{number of nodes uniquely classified}}{\text{number of nodes}}$. On the second plot, black represents the exceeding classifications for the given vertices: $\frac{\text{number of classifications}-\text{number of nodes}}{\text{number of nodes}}$.

### A. CPP list

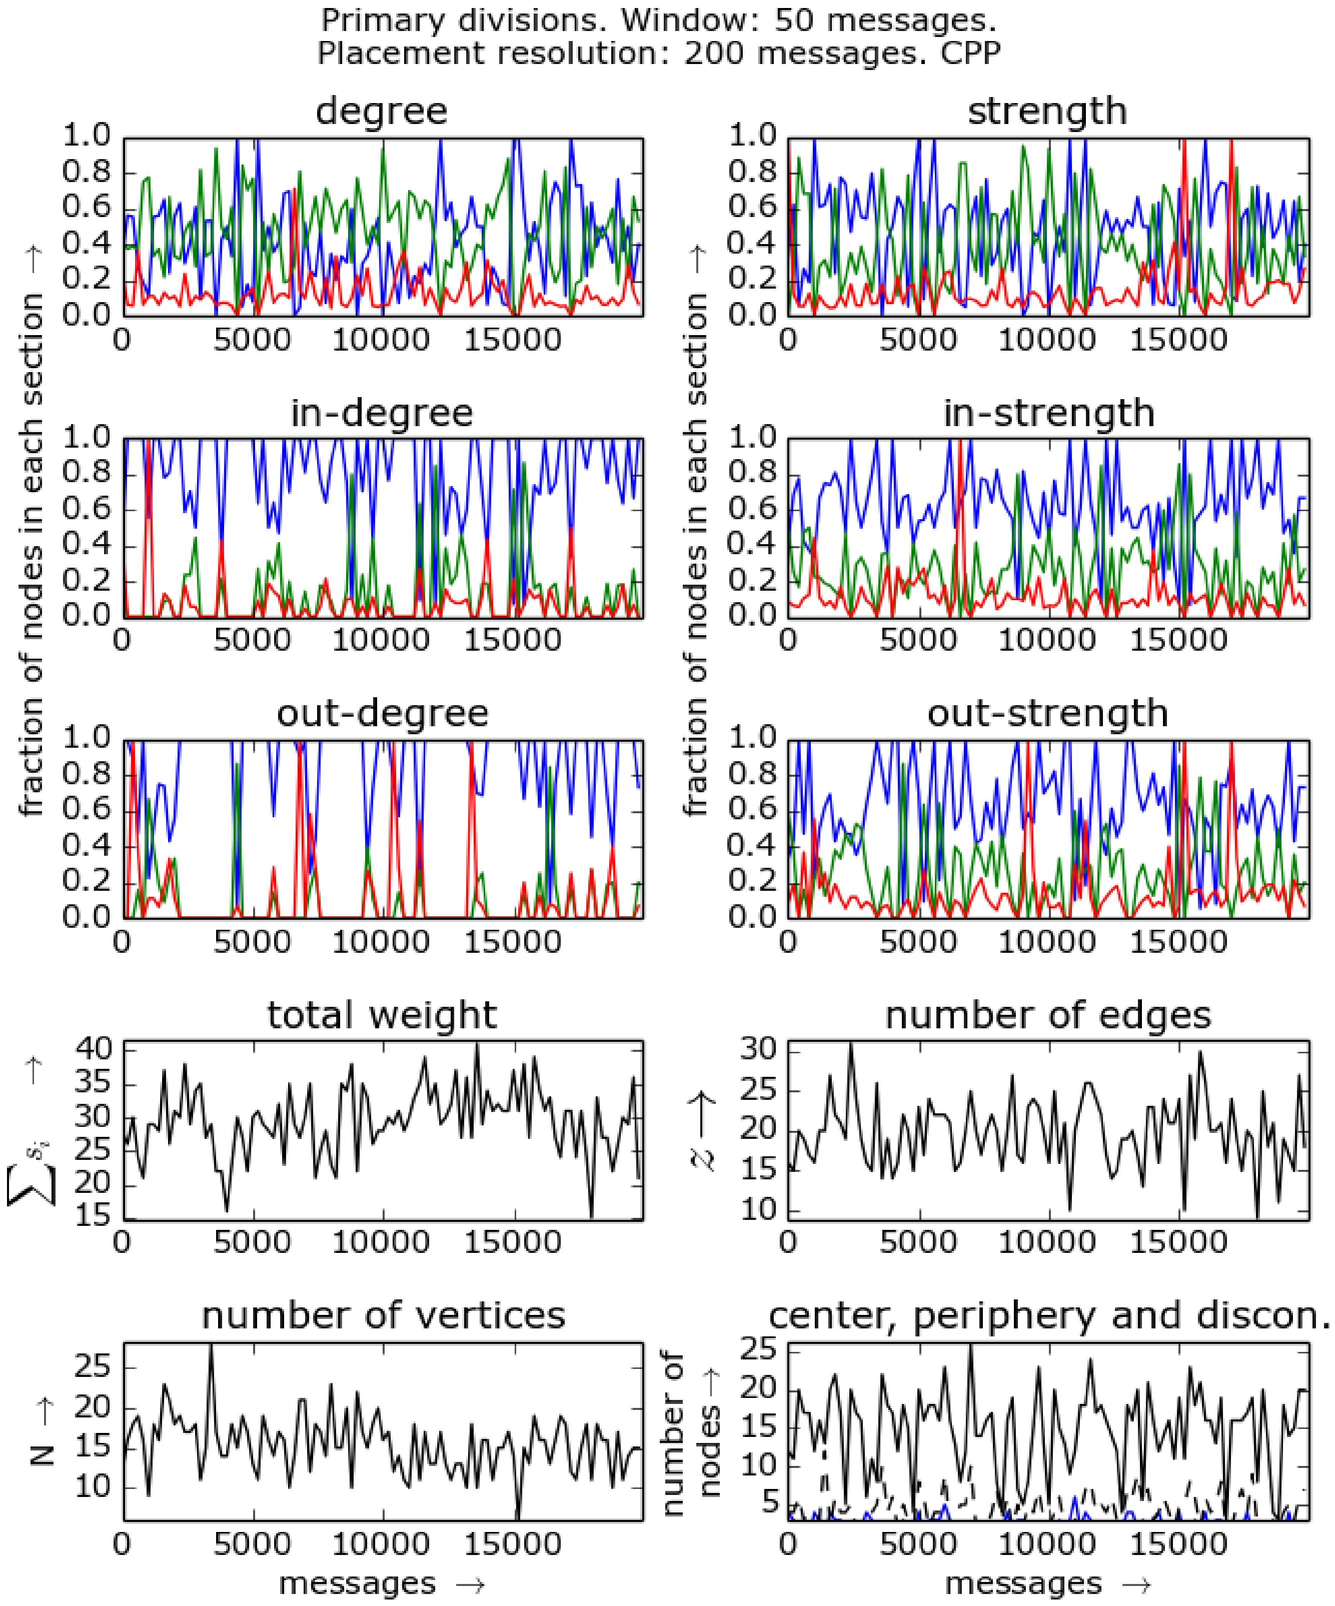

Primary divisions. Window: 50 messages.
Placement resolution: 200 messages. CPP
degree
strength
in-degree
in-strength
out-degree
out-strength
fraction of nodes in each section →
total weight
number of edges
number of vertices
center, periphery and discon.
messages →
number of nodes →
N →

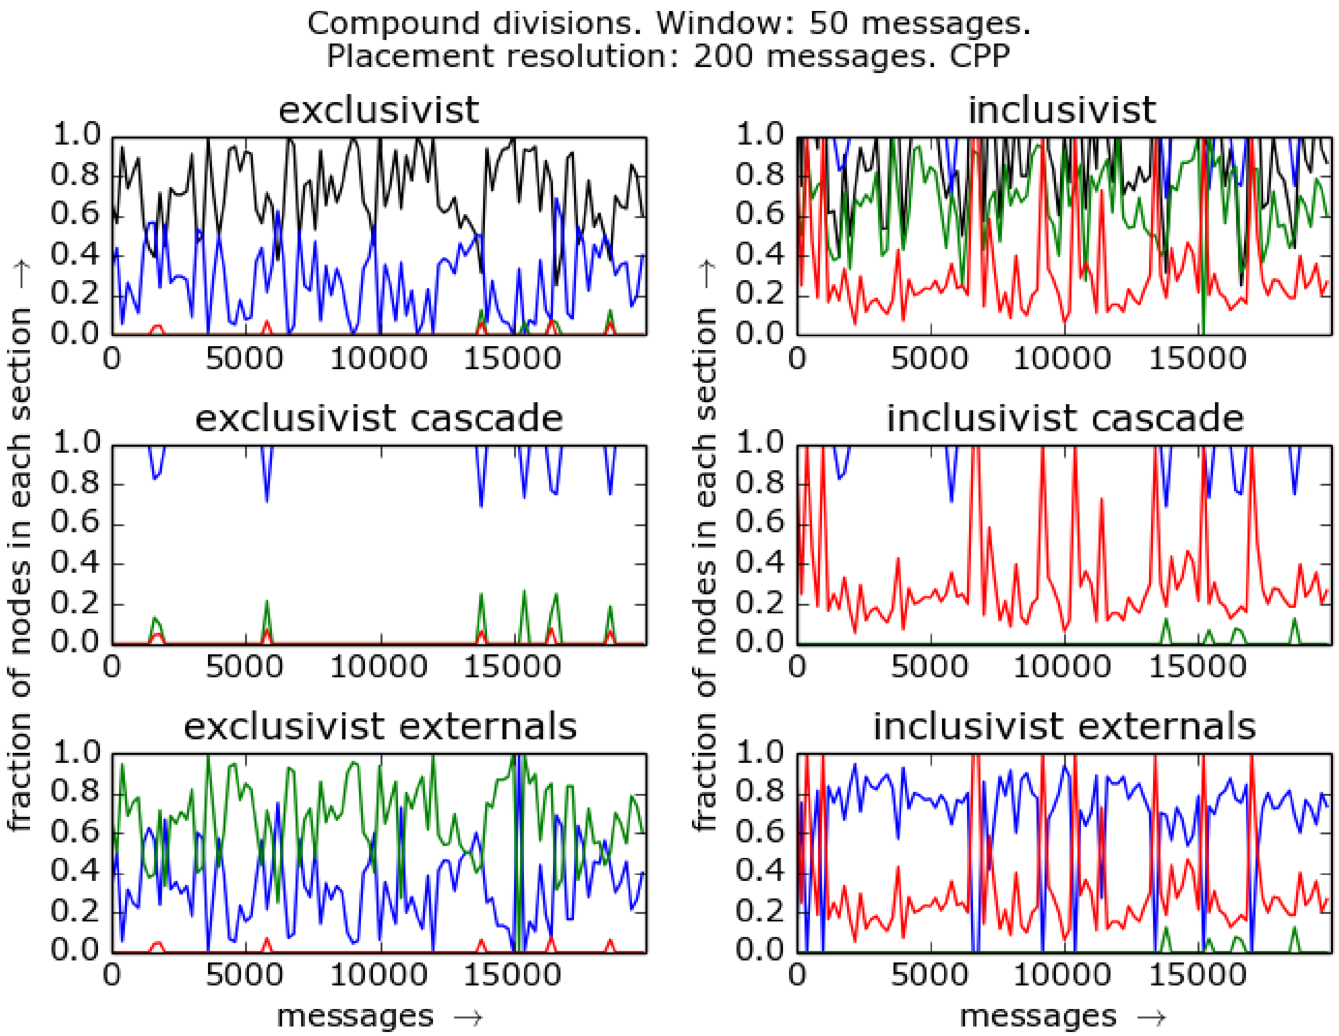

Compound divisions. Window: 50 messages.
Placement resolution: 200 messages. CPP
exclusivist
inclusivist
exclusivist cascade
inclusivist cascade
exclusivist externals
inclusivist externals
fraction of nodes in each section →
messages →
0.0
0.2
0.4
0.6
0.8
1.0
0
5000
10000
15000

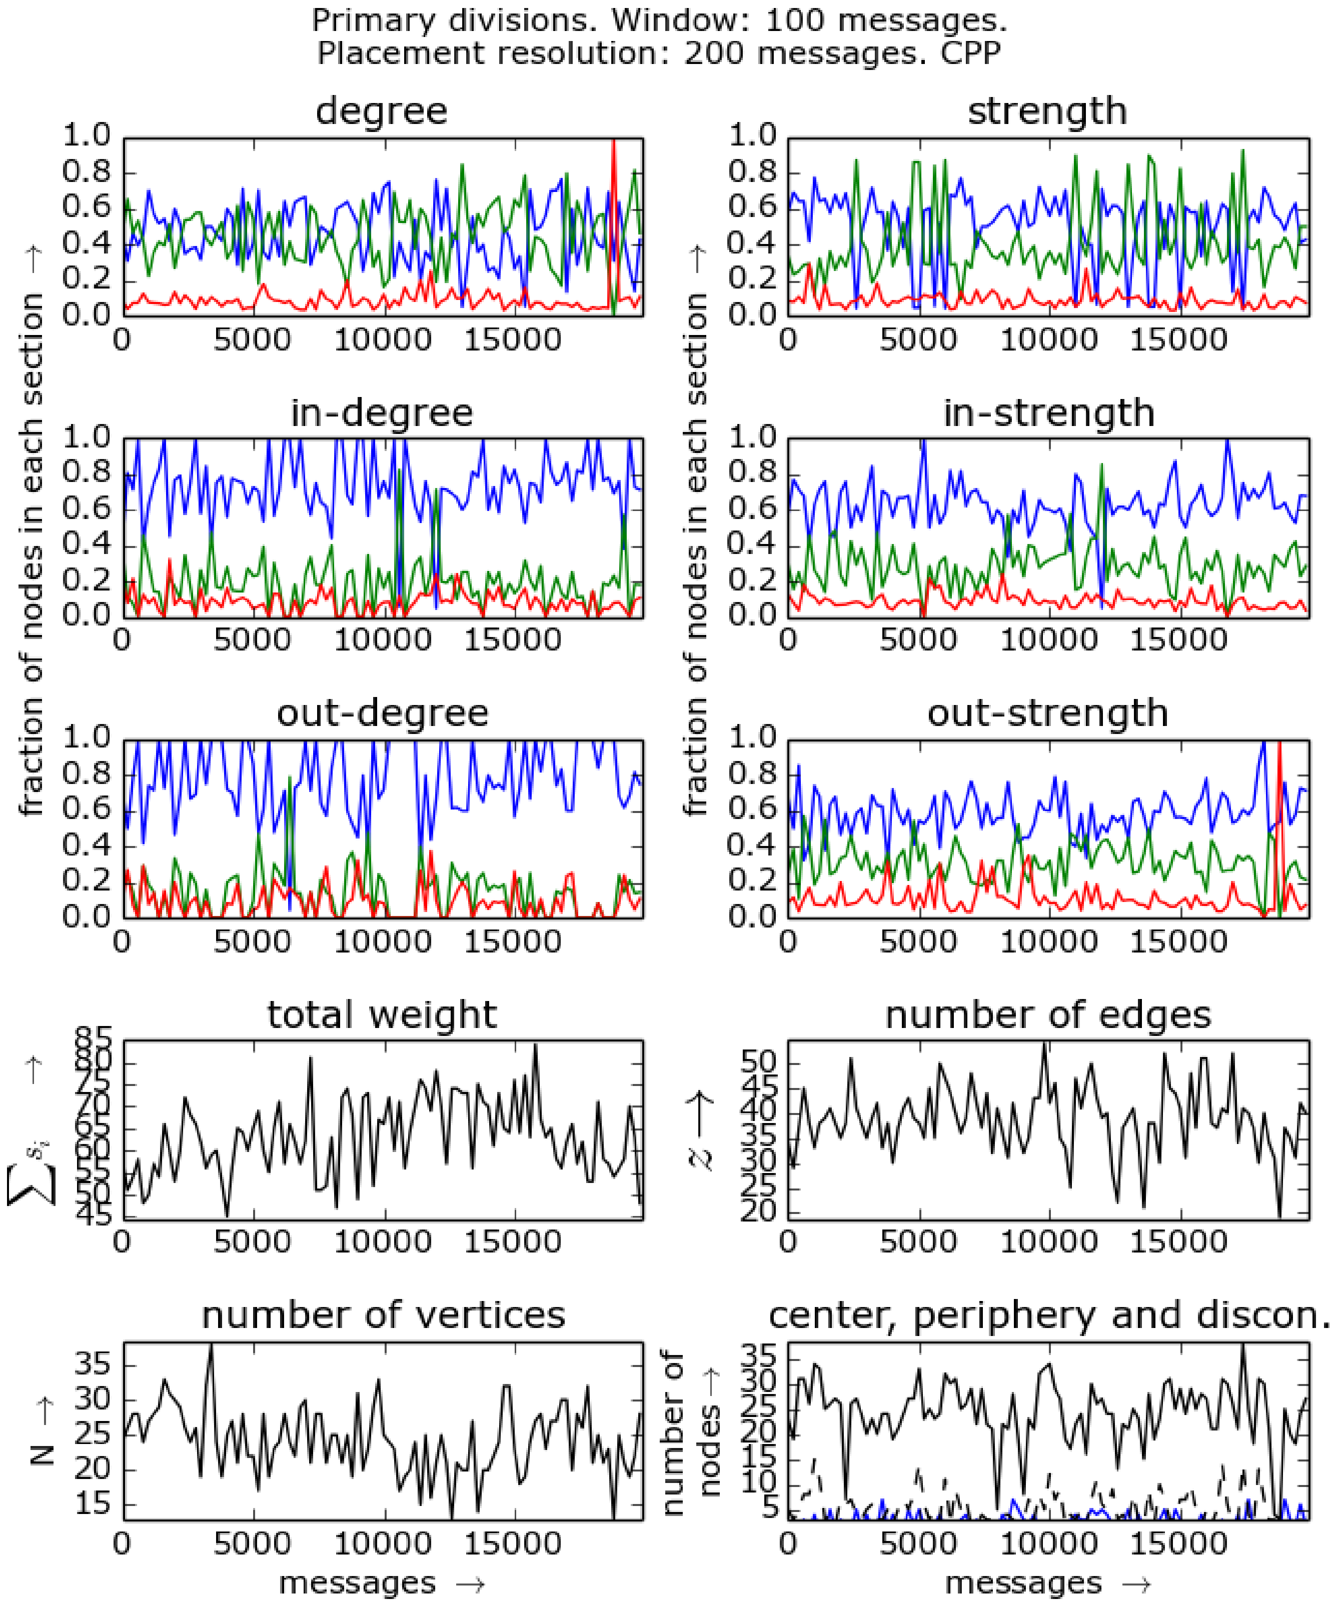
Primary divisions. Window: 100 messages.
Placement resolution: 200 messages. CPP
degree
strength
in-degree
in-strength
out-degree
out-strength
fraction of nodes in each section →
total weight
number of edges
number of vertices
center, periphery and discon.
$\sum s_i$ →
$z$ →
N →
number of nodes →
messages →

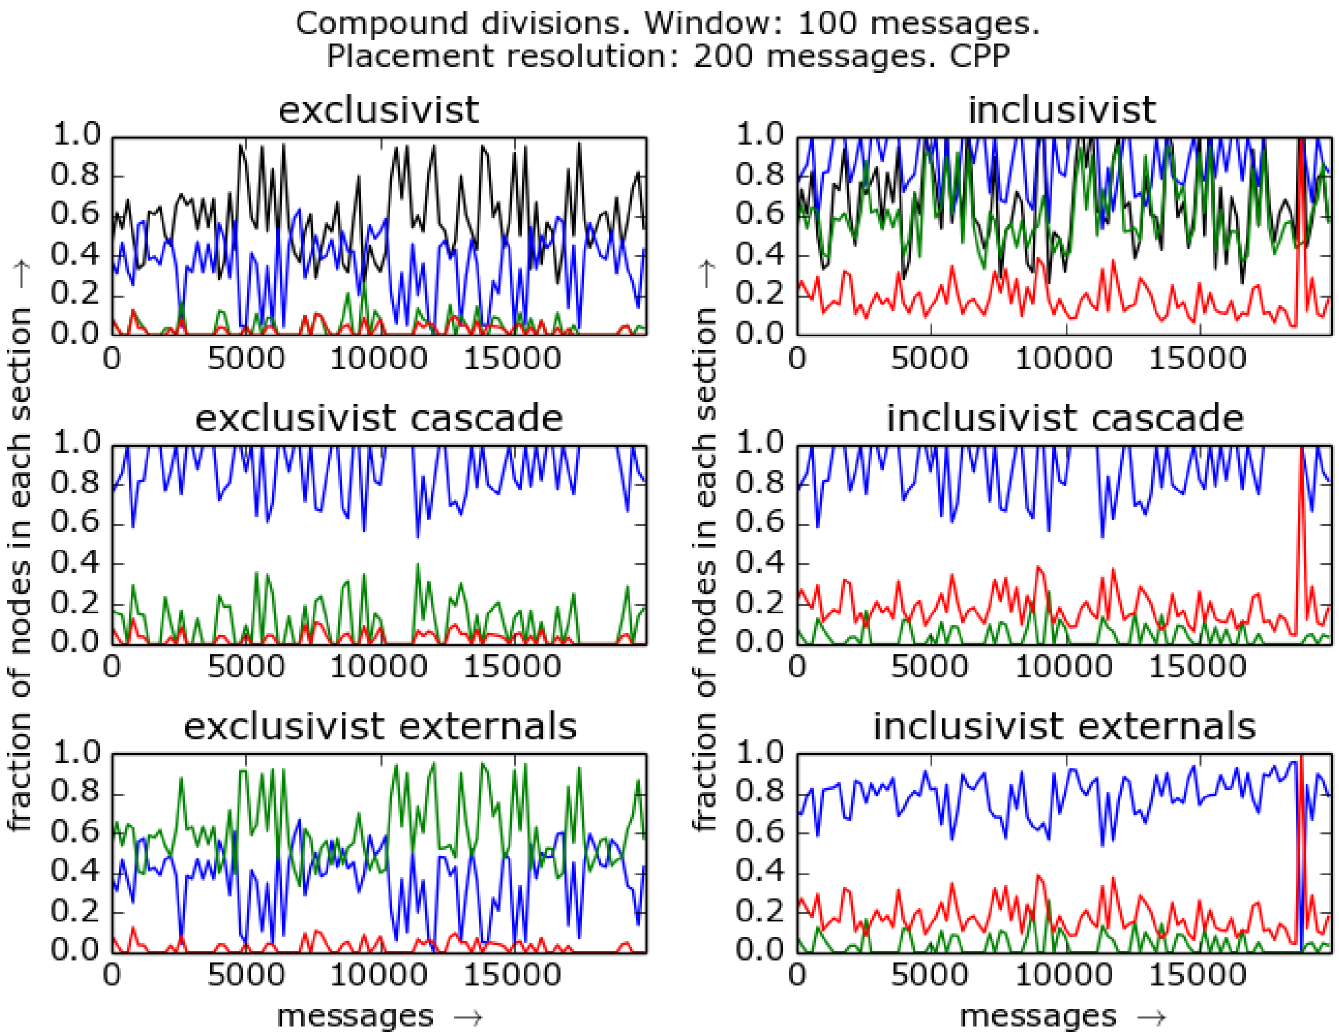
Compound divisions. Window: 100 messages.
Placement resolution: 200 messages. CPP
exclusivist
inclusivist
exclusivist cascade
inclusivist cascade
exclusivist externals
inclusivist externals
fraction of nodes in each section →
messages →
1.0
0.8
0.6
0.4
0.2
0.0
0
5000
10000
15000

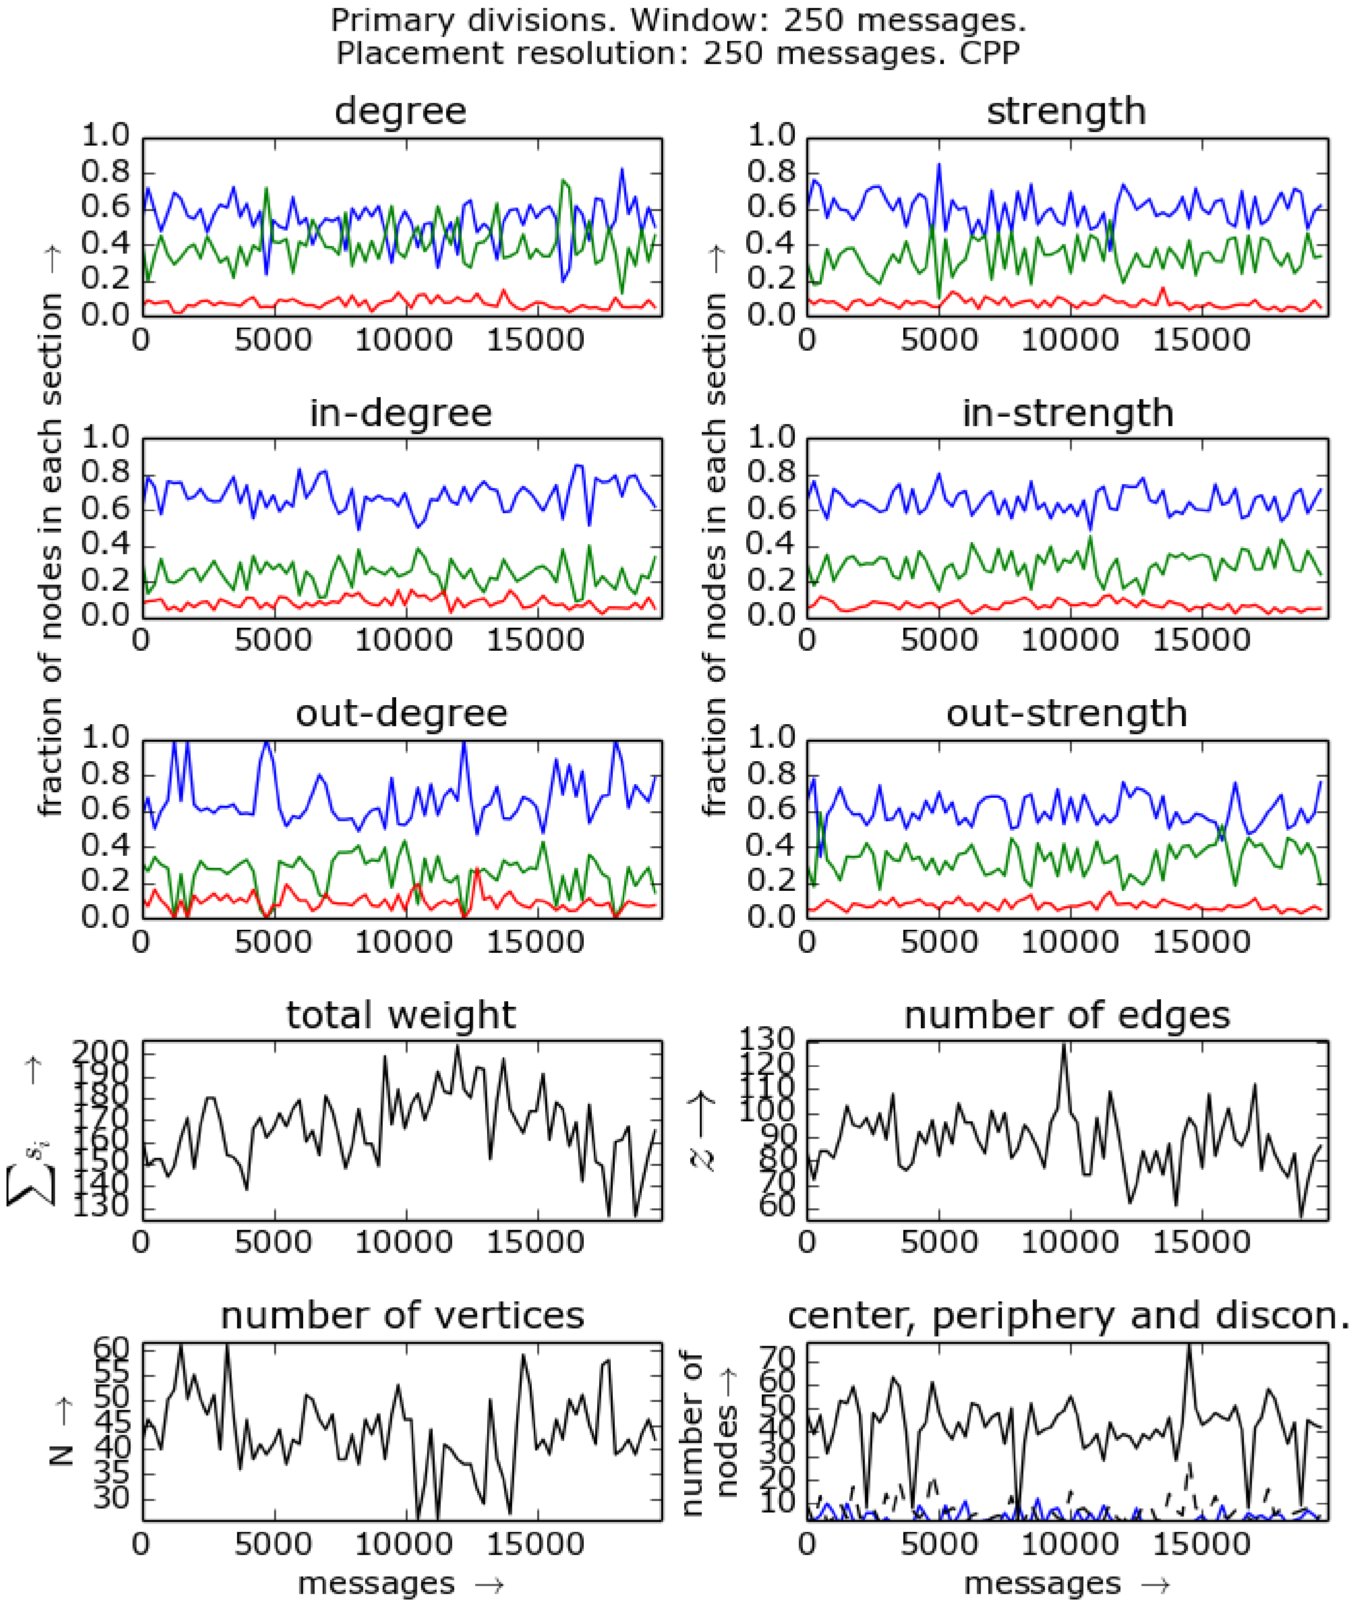
Primary divisions. Window: 250 messages.
Placement resolution: 250 messages. CPP
degree
strength
in-degree
in-strength
out-degree
out-strength
fraction of nodes in each section →
total weight
number of edges
number of vertices
center, periphery and discon.
messages →
N →
number of nodes →

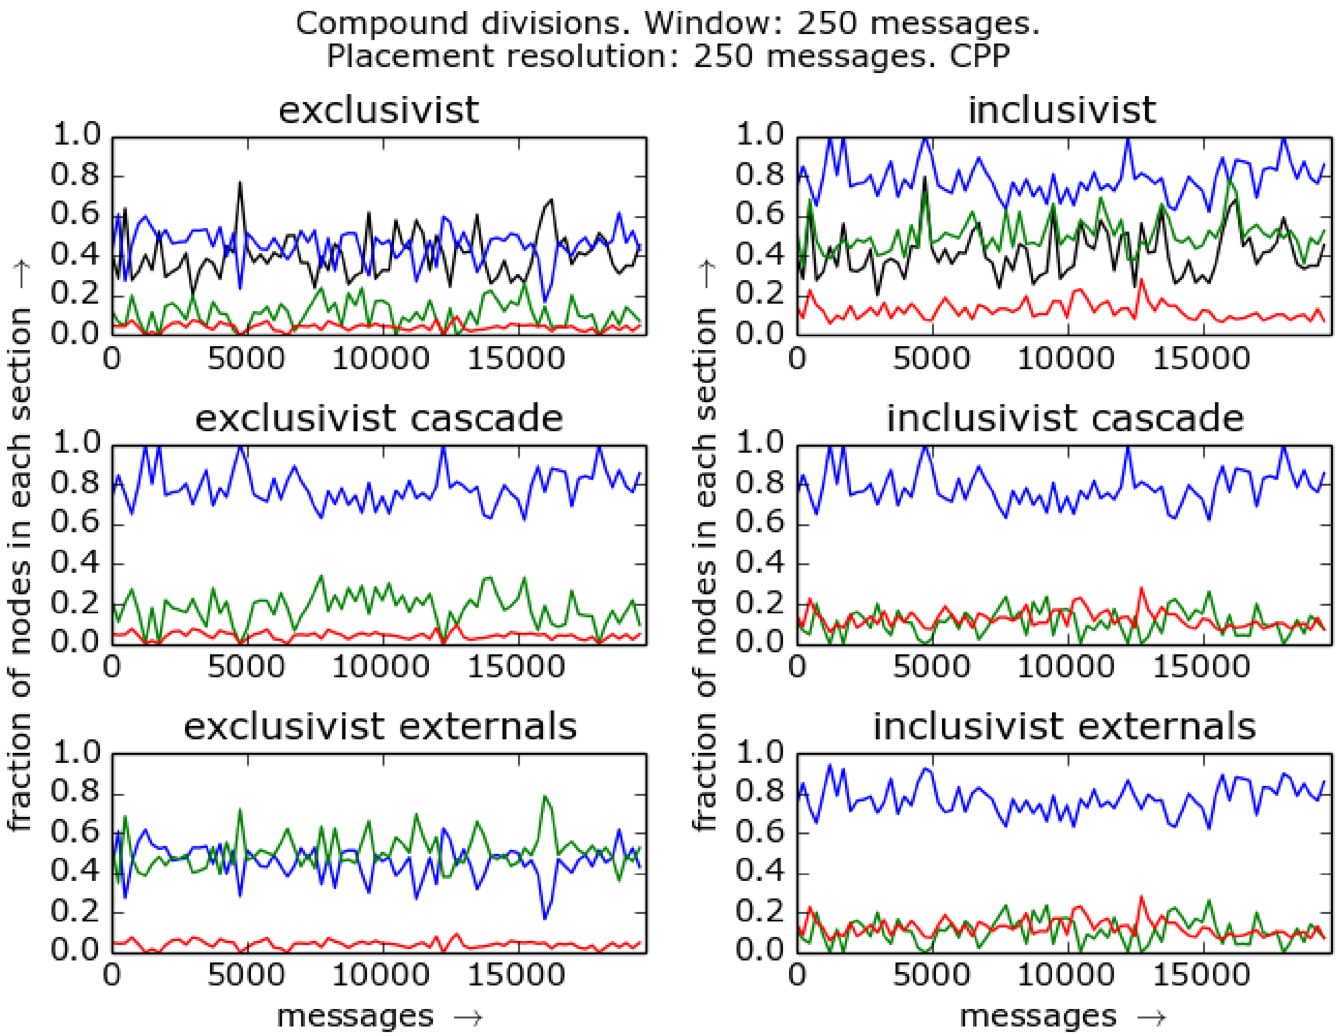
Compound divisions. Window: 250 messages.
Placement resolution: 250 messages. CPP
exclusivist
inclusivist
exclusivist cascade
inclusivist cascade
exclusivist externals
inclusivist externals
fraction of nodes in each section →
messages →
1.0
0.8
0.6
0.4
0.2
0.0
0
5000
10000
15000

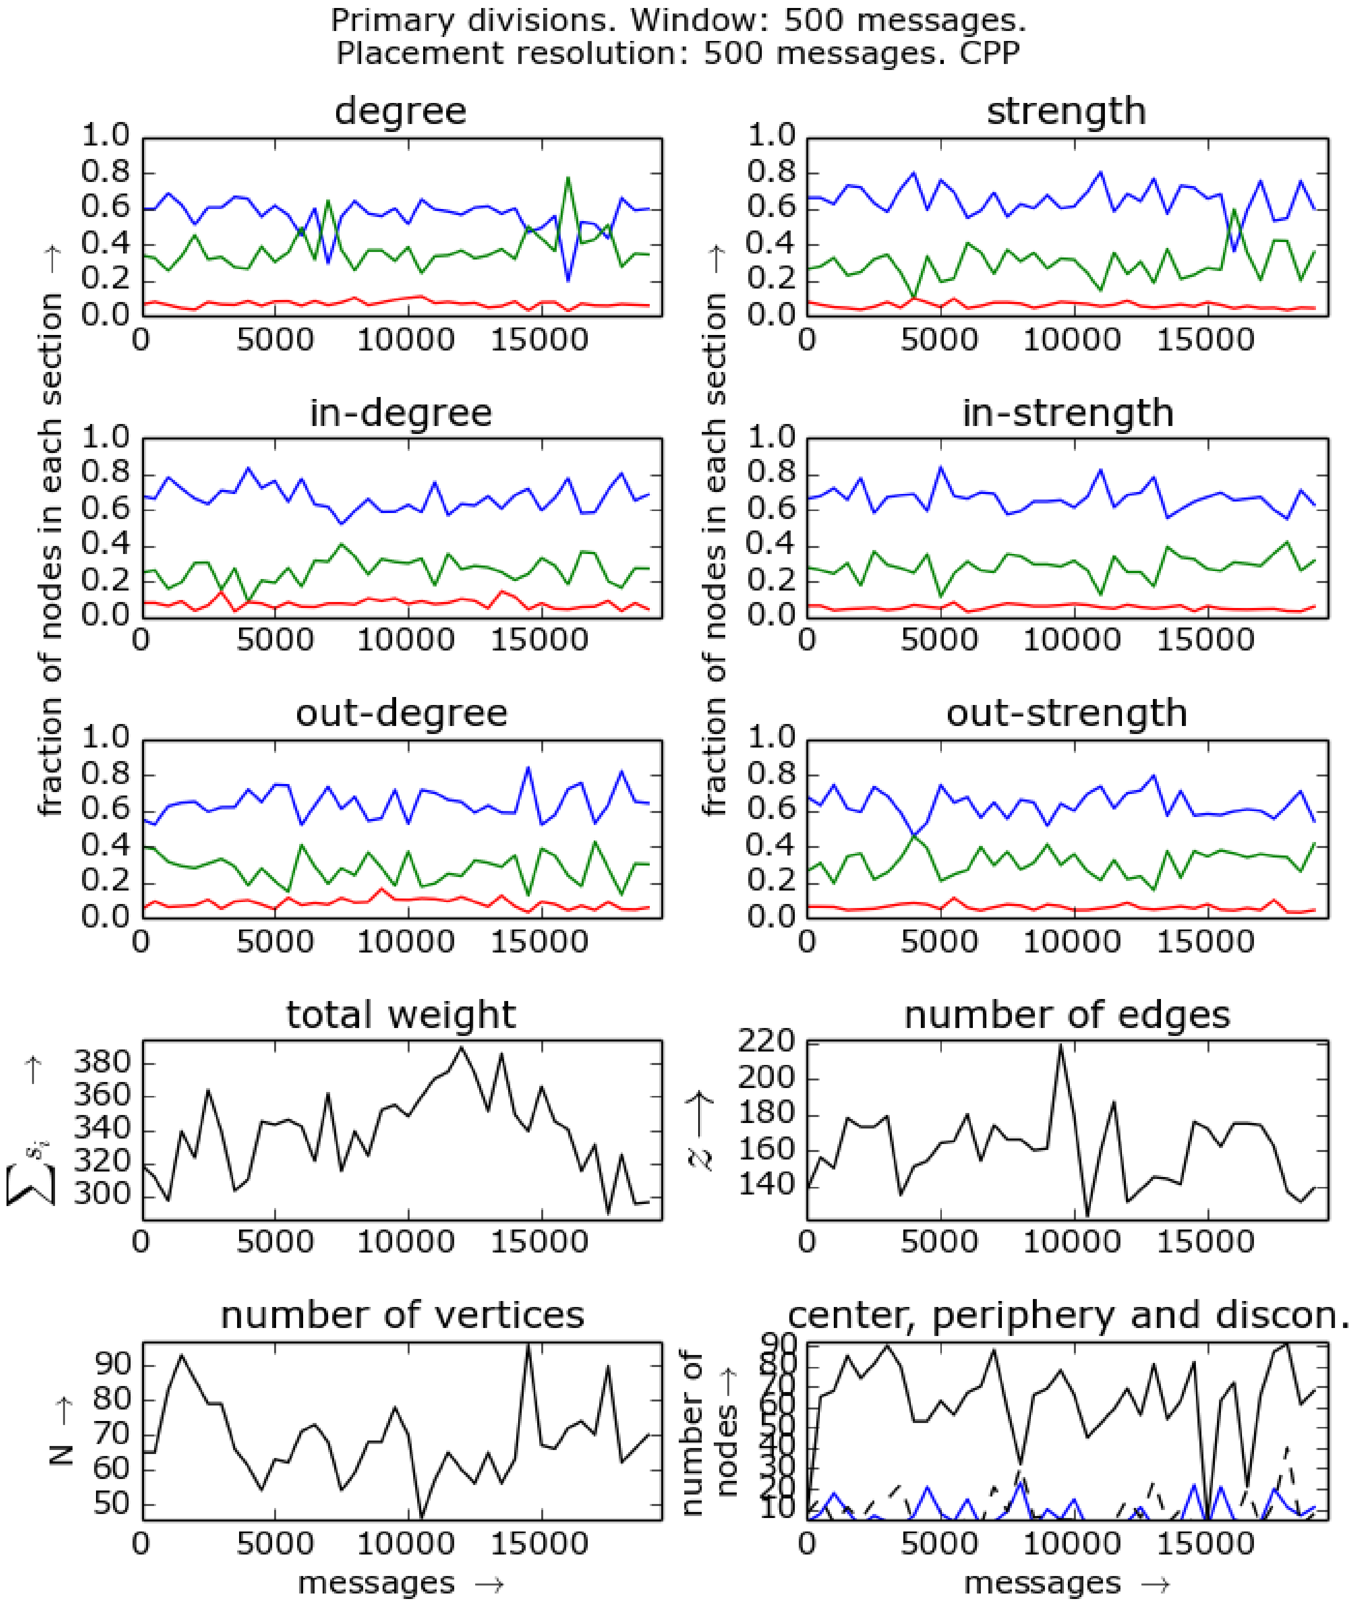
Primary divisions. Window: 500 messages.
Placement resolution: 500 messages. CPP
degree
strength
in-degree
in-strength
out-degree
out-strength
fraction of nodes in each section →
total weight
number of edges
number of vertices
center, periphery and discon.
messages →
number of nodes →
N →

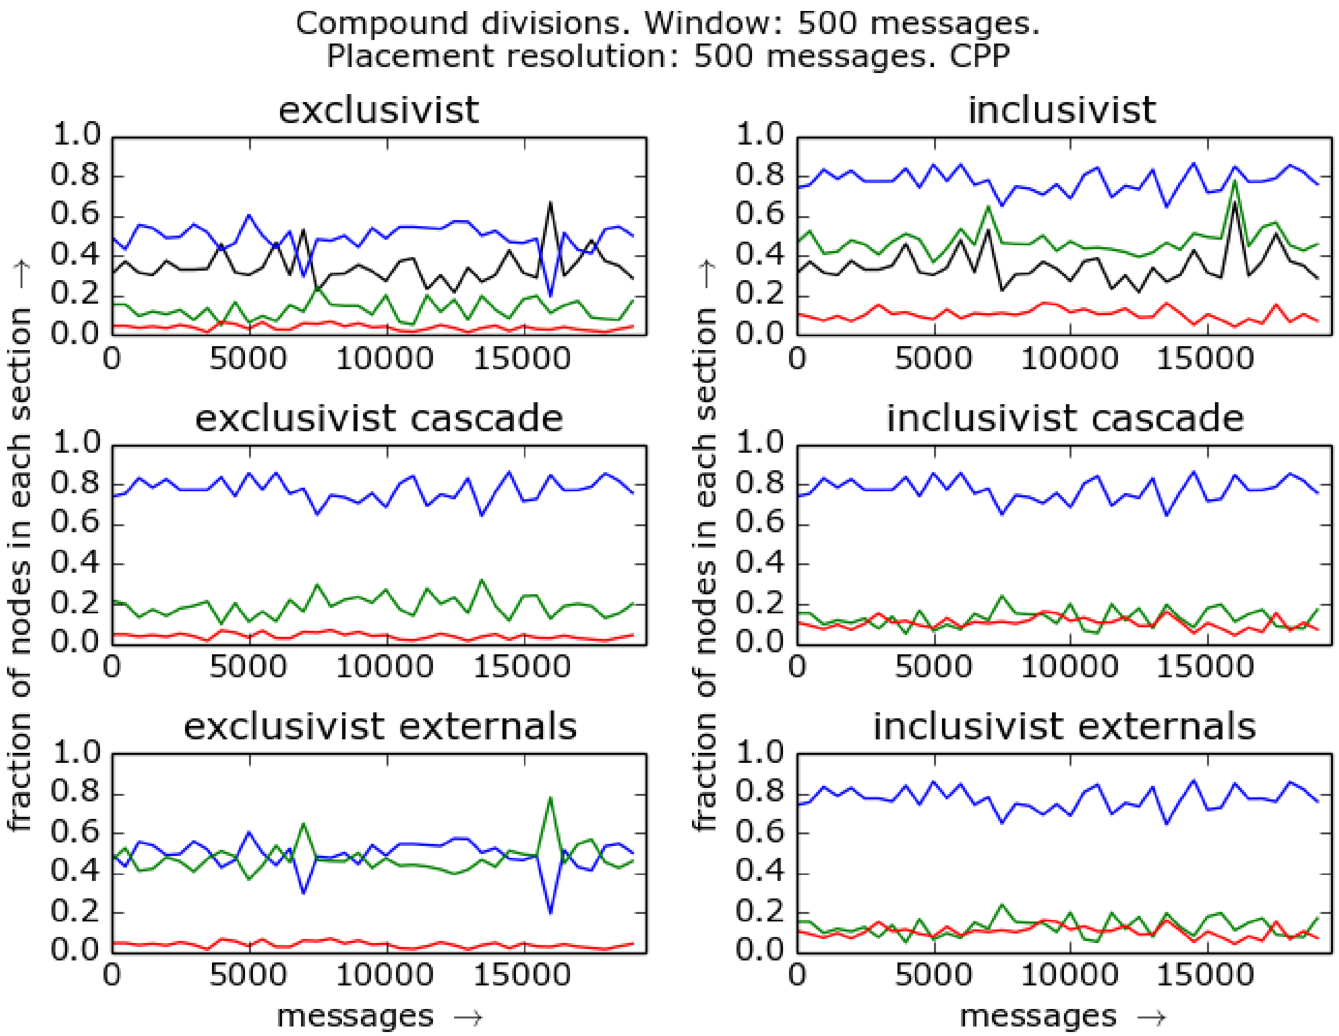
Compound divisions. Window: 500 messages.
Placement resolution: 500 messages. CPP
exclusivist
inclusivist
exclusivist cascade
inclusivist cascade
exclusivist externals
inclusivist externals
fraction of nodes in each section →
messages →
0
5000
10000
15000
0.0
0.2
0.4
0.6
0.8
1.0

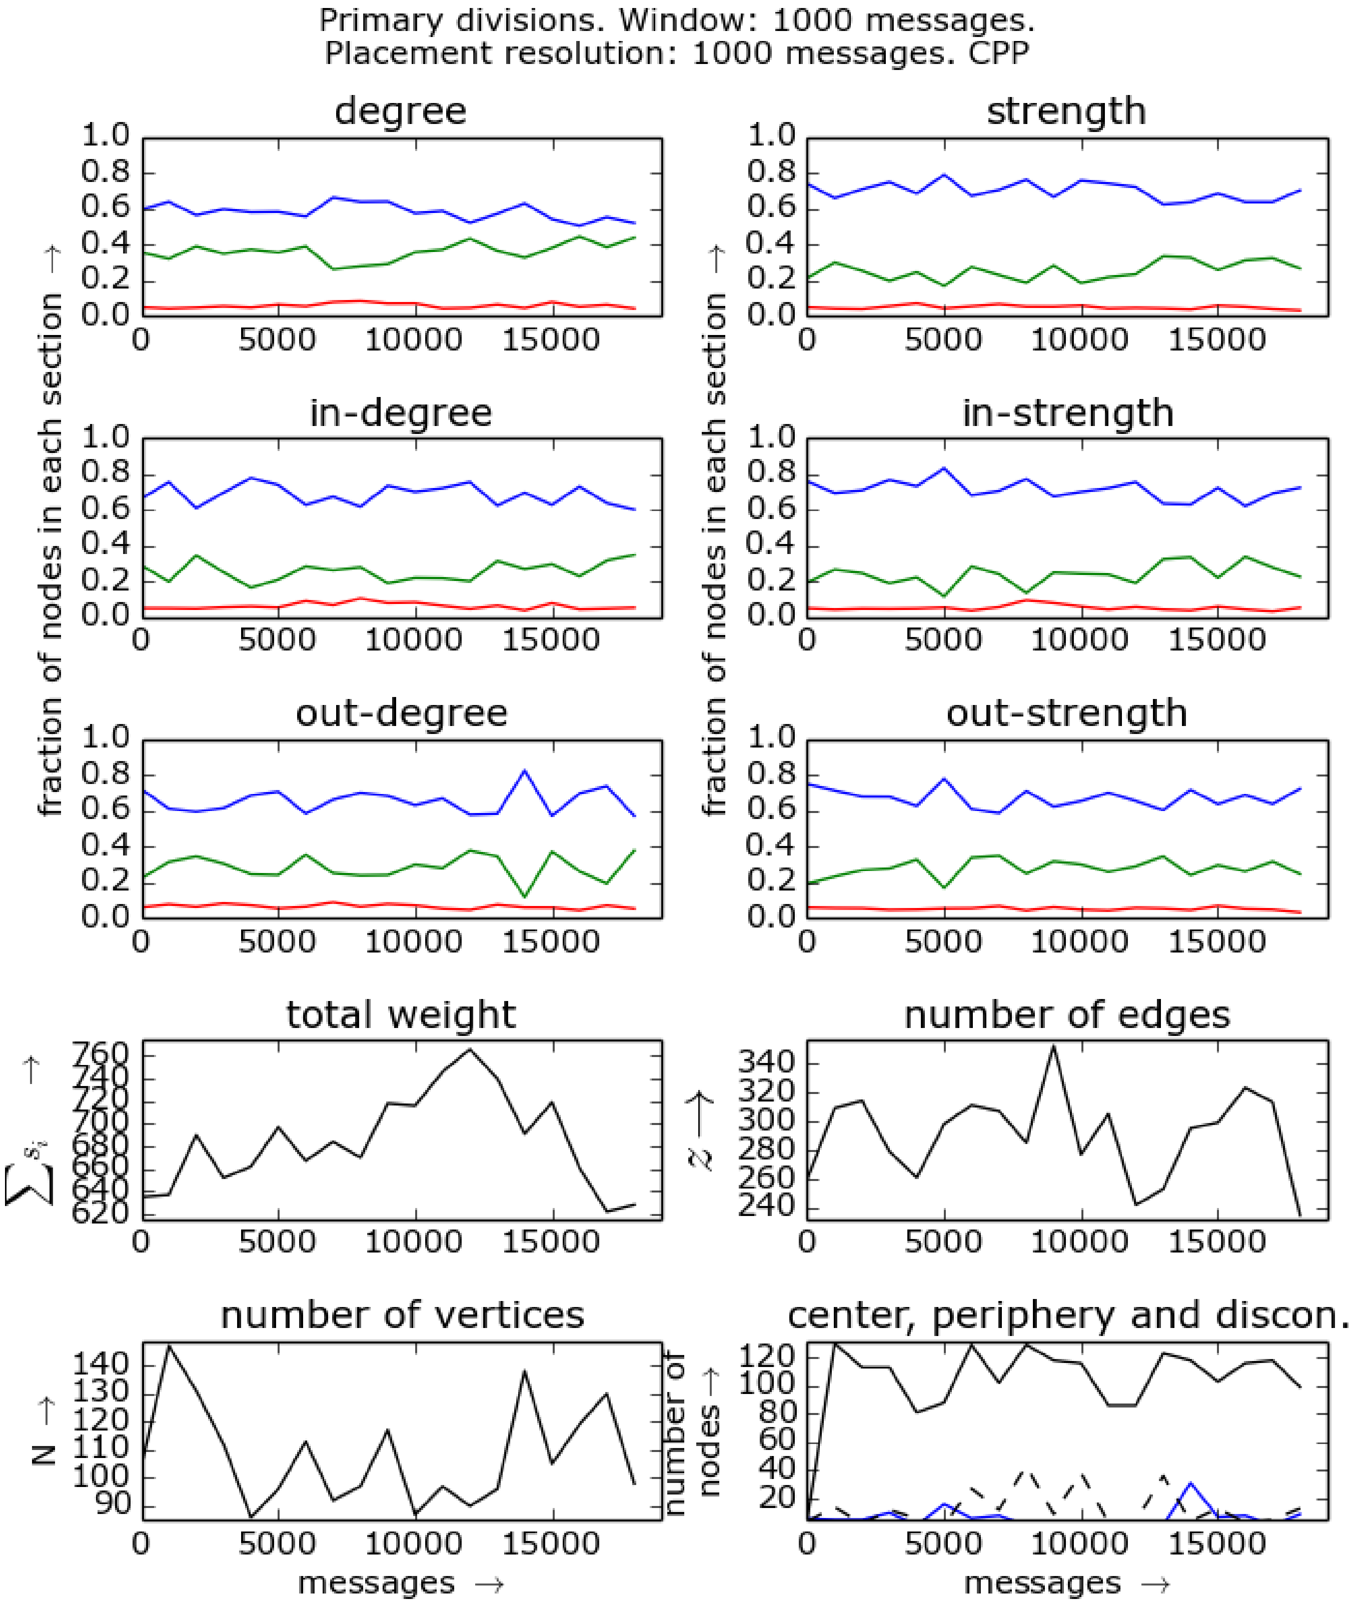
Primary divisions. Window: 1000 messages.
Placement resolution: 1000 messages. CPP
degree
strength
in-degree
in-strength
out-degree
out-strength
fraction of nodes in each section →
total weight
number of edges
number of vertices
center, periphery and discon.
messages →
number of nodes →
N →
z →
$\sum s_i$ →

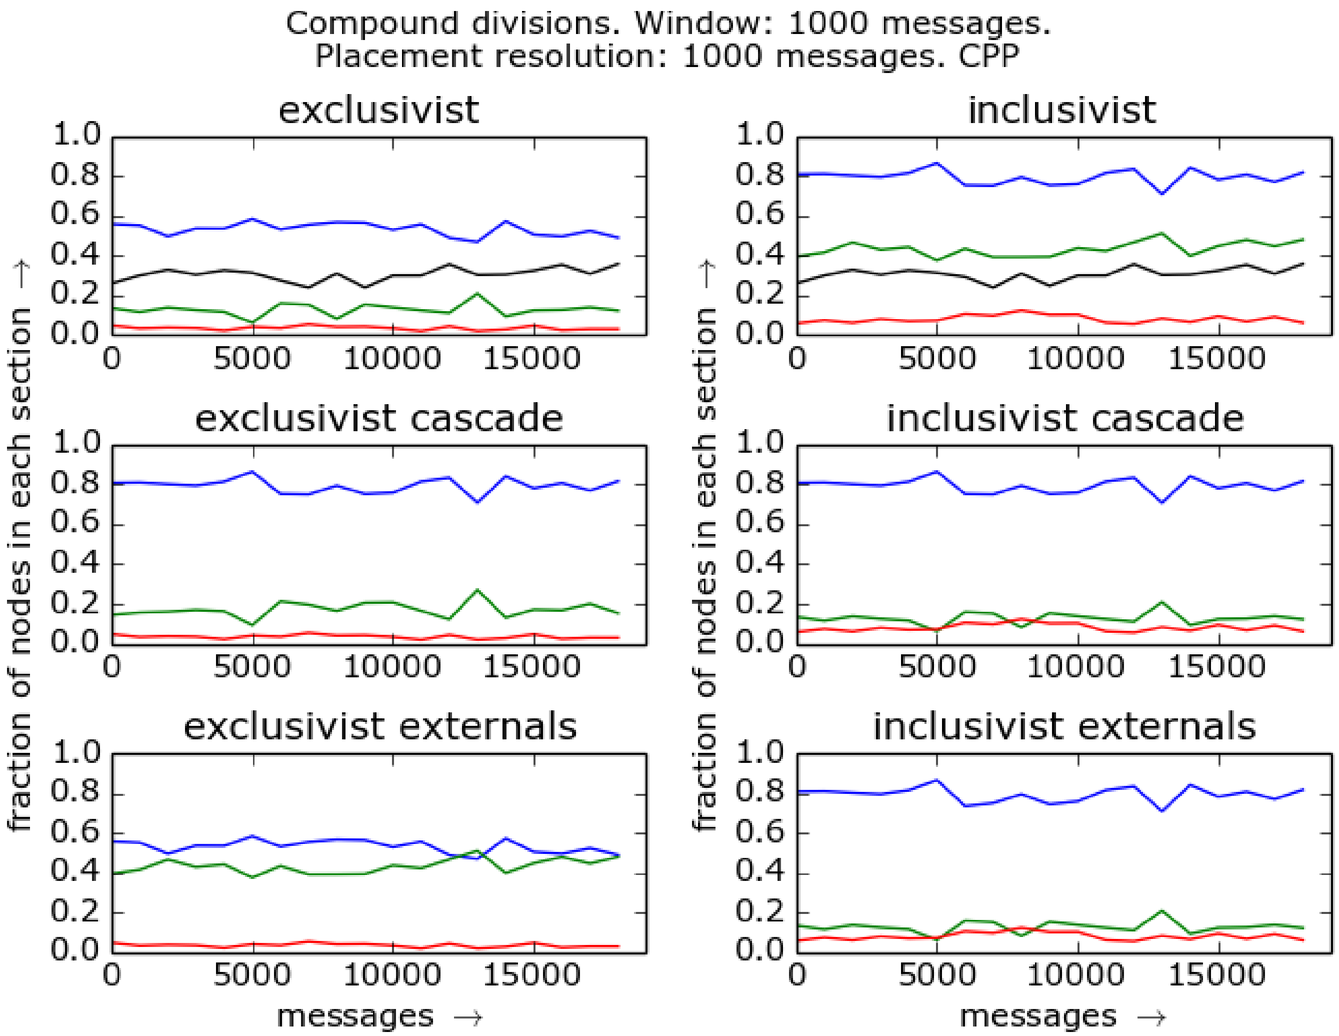
Compound divisions. Window: 1000 messages.
Placement resolution: 1000 messages. CPP
exclusivist
inclusivist
exclusivist cascade
inclusivist cascade
exclusivist externals
inclusivist externals
fraction of nodes in each section →
messages →
1.0
0.8
0.6
0.4
0.2
0.0
0
5000
10000
15000

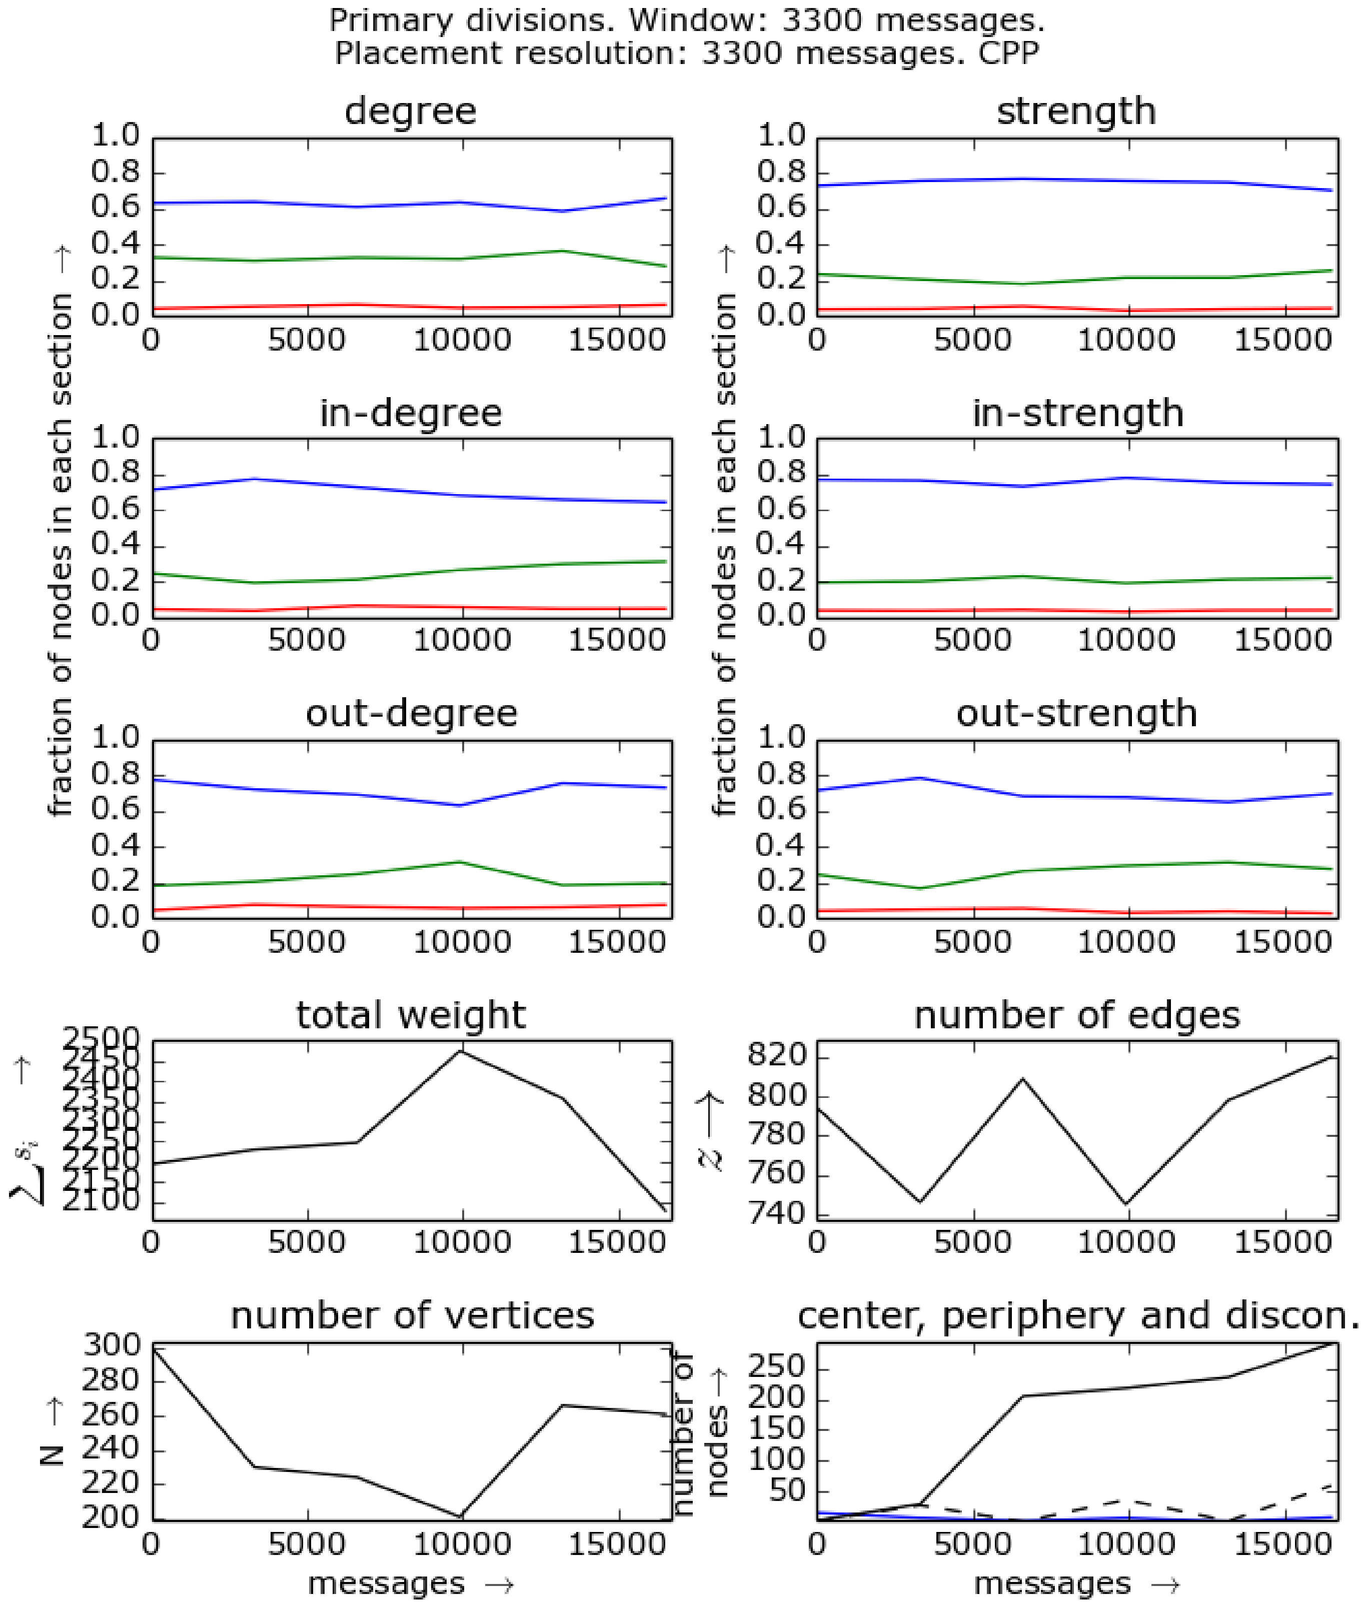
Primary divisions. Window: 3300 messages.
Placement resolution: 3300 messages. CPP
degree
strength
in-degree
in-strength
out-degree
out-strength
fraction of nodes in each section →
total weight
number of edges
number of vertices
center, periphery and discon.
N →
number of nodes →
messages →

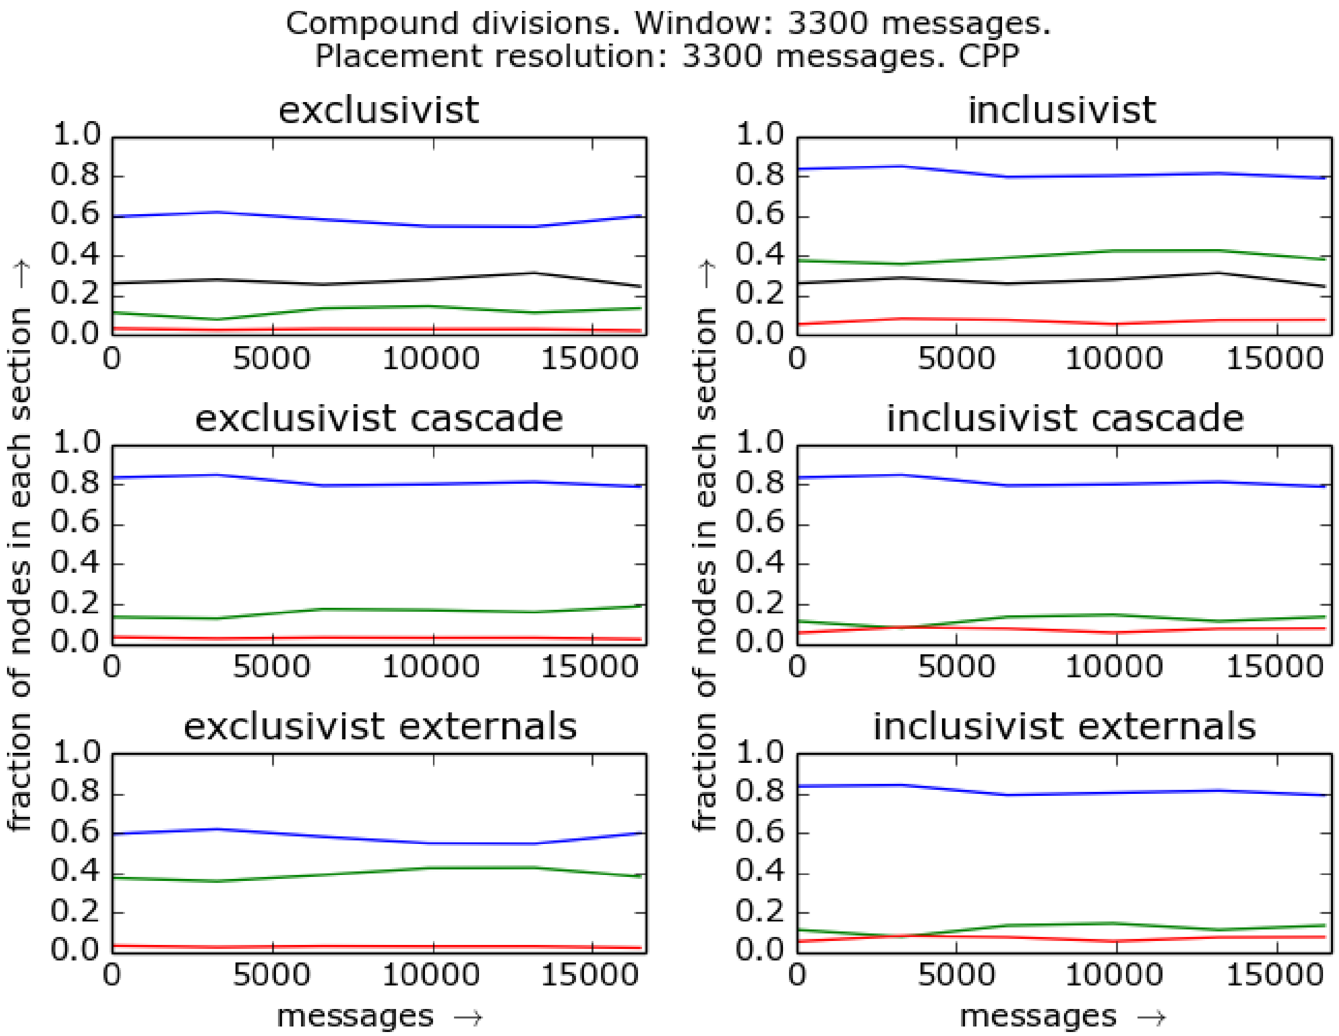
Compound divisions. Window: 3300 messages.
Placement resolution: 3300 messages. CPP
exclusivist
inclusivist
exclusivist cascade
inclusivist cascade
exclusivist externals
inclusivist externals
fraction of nodes in each section →
messages →
1.0
0.8
0.6
0.4
0.2
0.0
0
5000
10000
15000

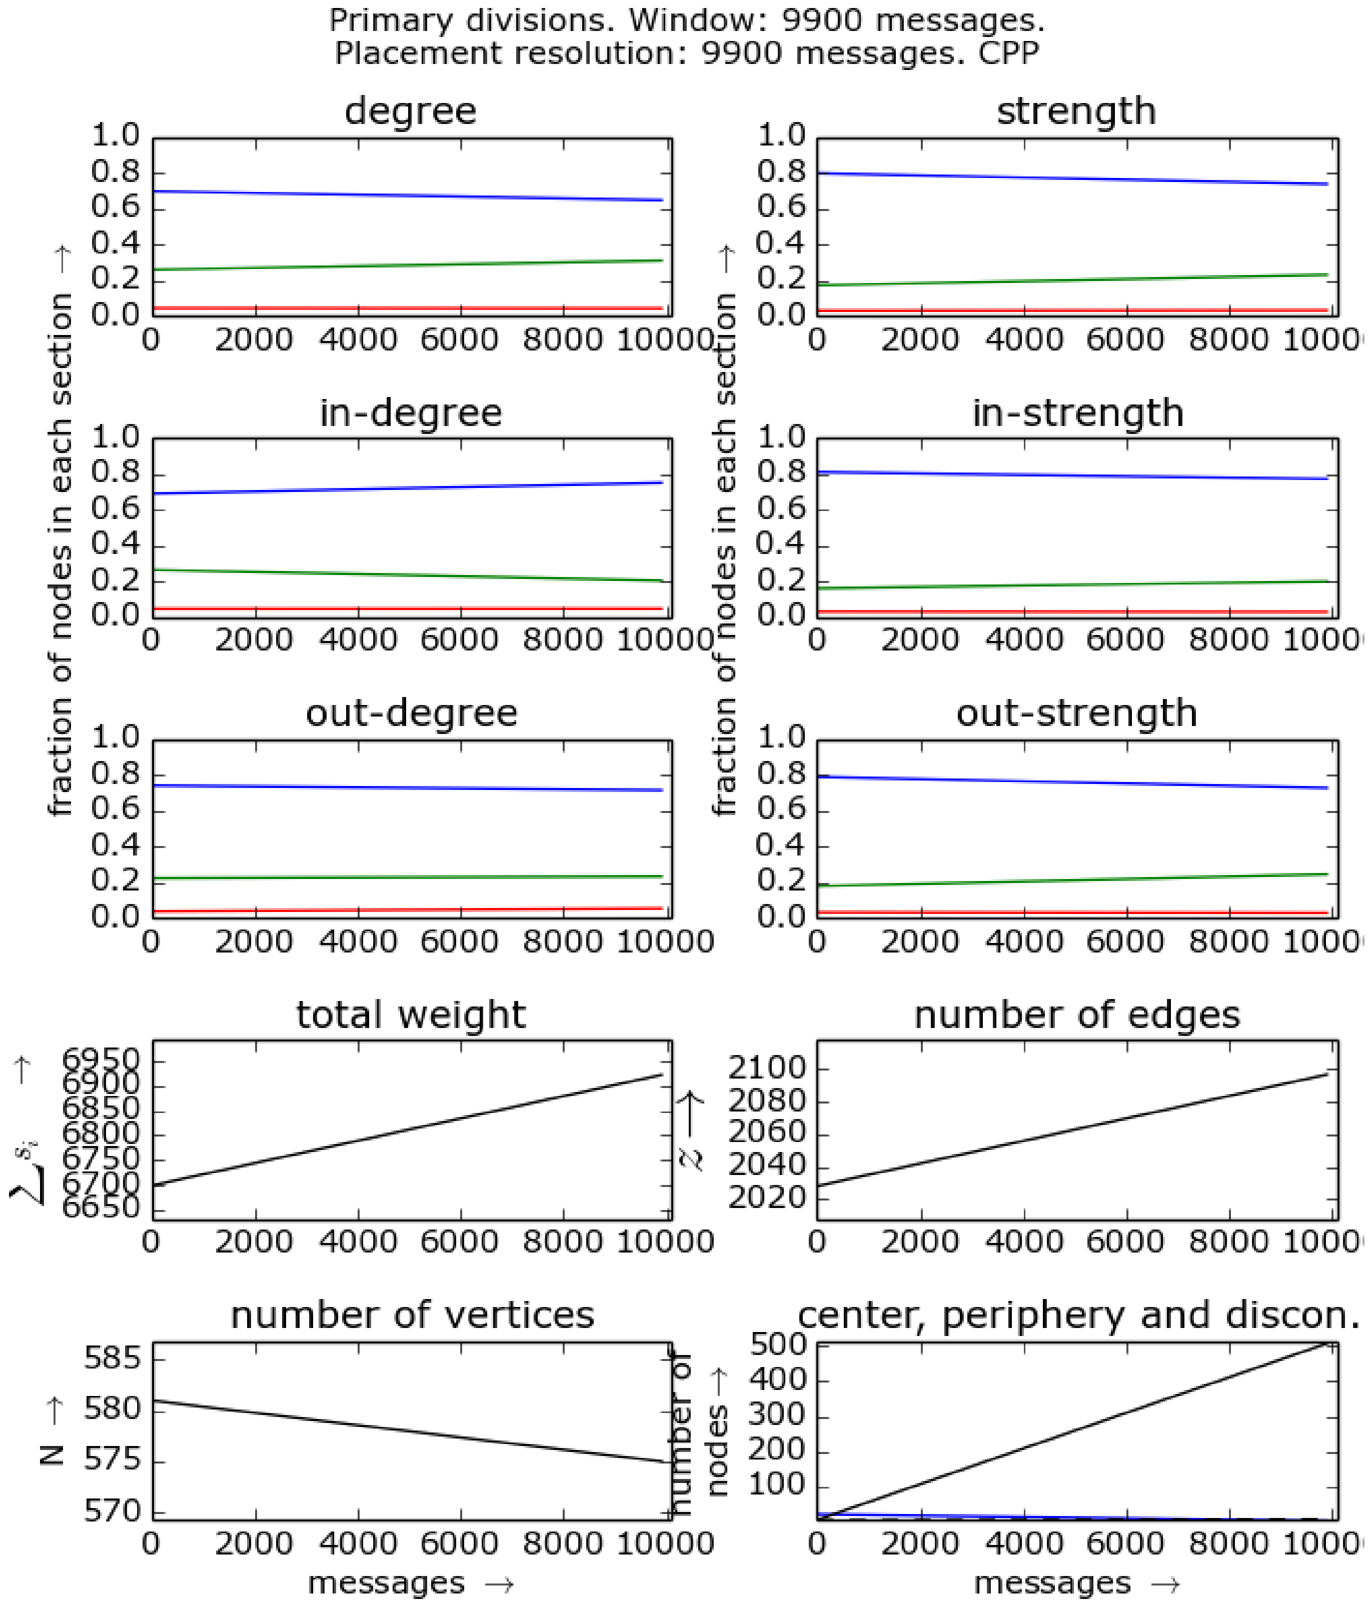

Primary divisions. Window: 9900 messages.
Placement resolution: 9900 messages. CPP
degree
strength
in-degree
in-strength
out-degree
out-strength
fraction of nodes in each section →
total weight
number of edges
number of vertices
center, periphery and discon.
N →
number of nodes →
messages →

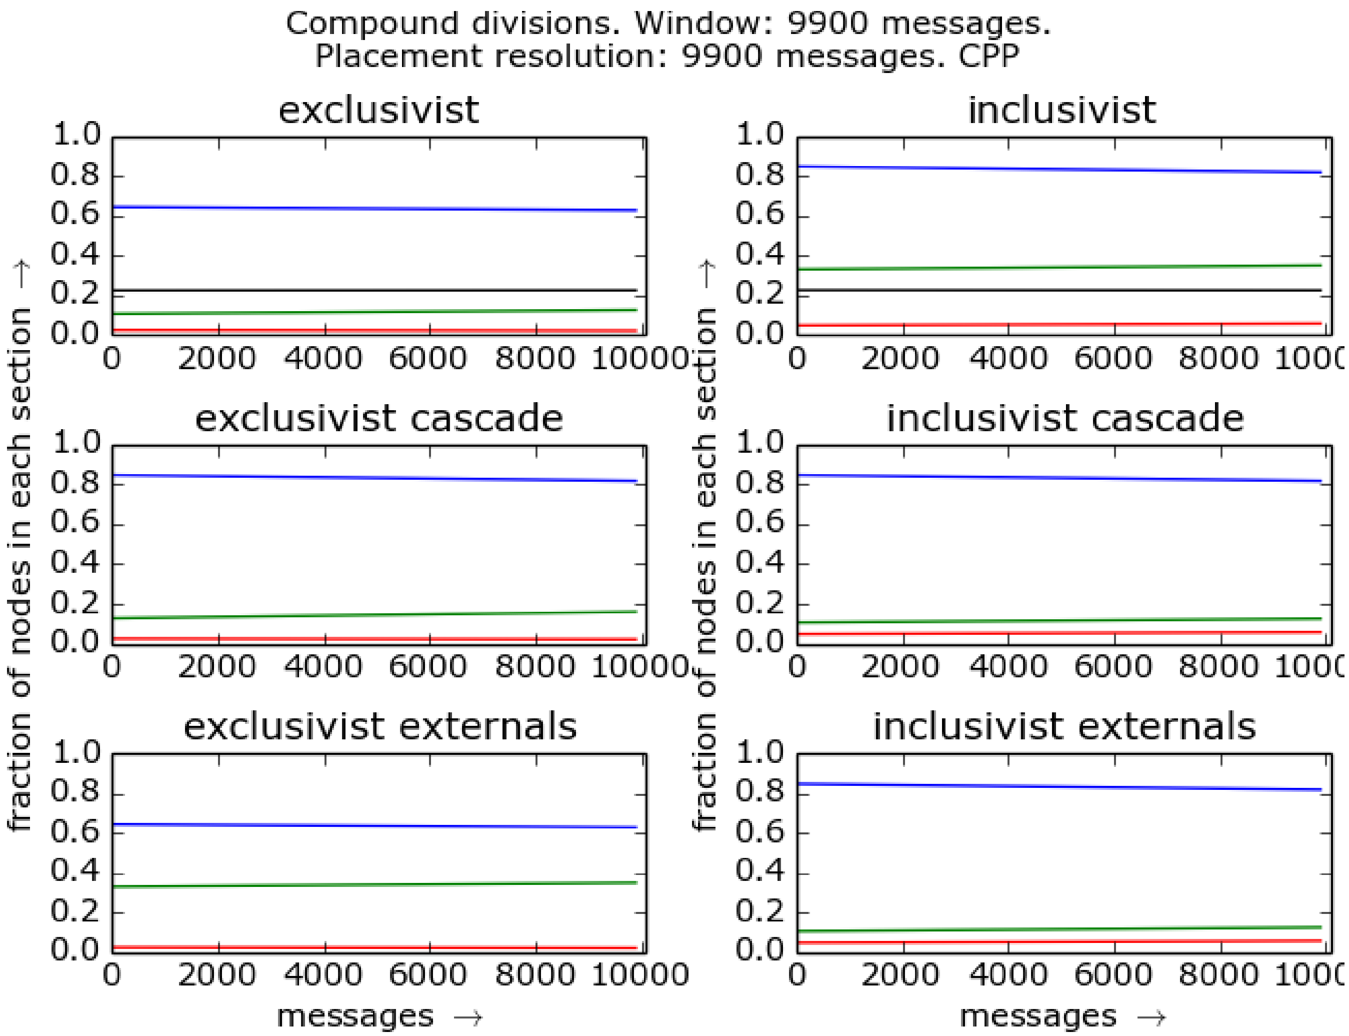
Compound divisions. Window: 9900 messages.
Placement resolution: 9900 messages. CPP
exclusivist
inclusivist
exclusivist cascade
inclusivist cascade
exclusivist externals
inclusivist externals
fraction of nodes in each section →
messages →
1.0
0.8
0.6
0.4
0.2
0.0
0
2000
4000
6000
8000
10000

### B. LAD list

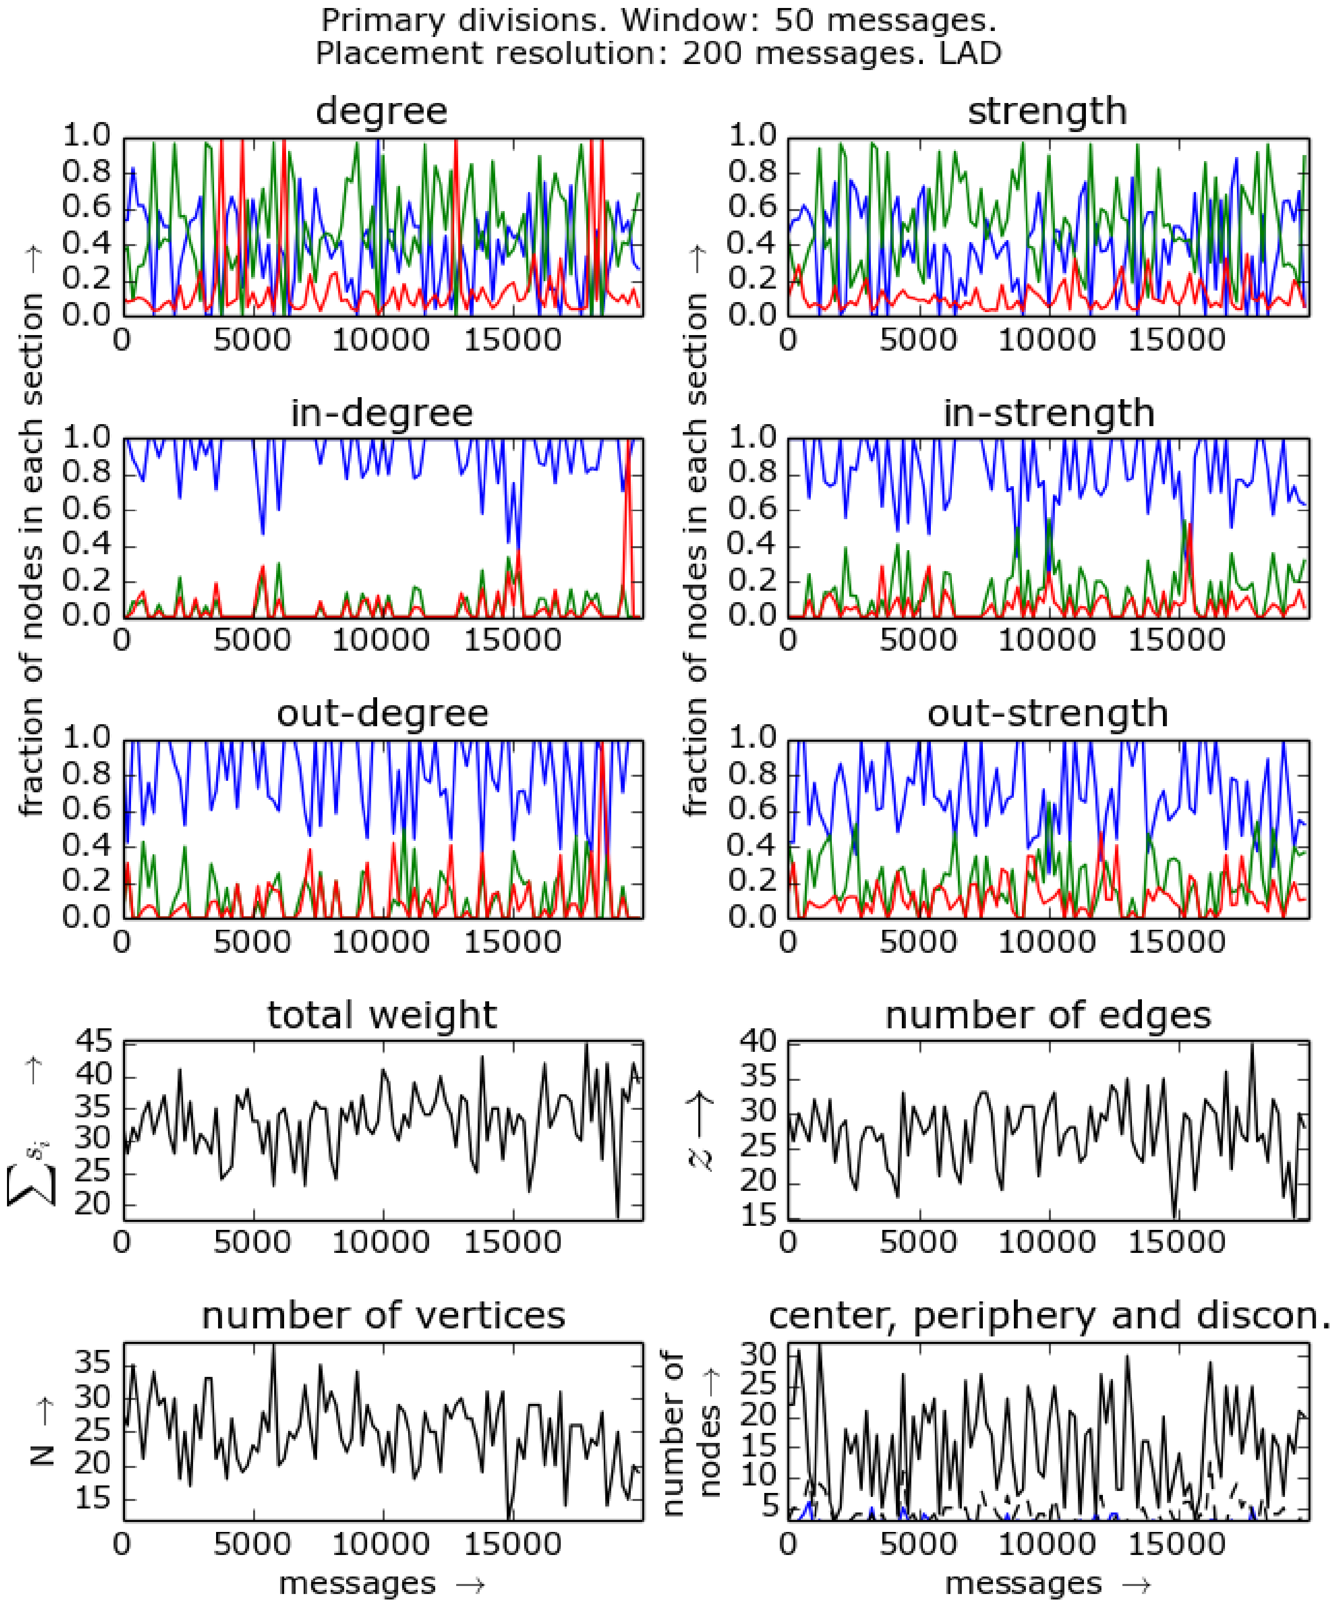
Primary divisions. Window: 50 messages.
Placement resolution: 200 messages. LAD
degree
strength
in-degree
in-strength
out-degree
out-strength
fraction of nodes in each section →
total weight
number of edges
number of vertices
center, periphery and discon.
messages →
N →
number of nodes →

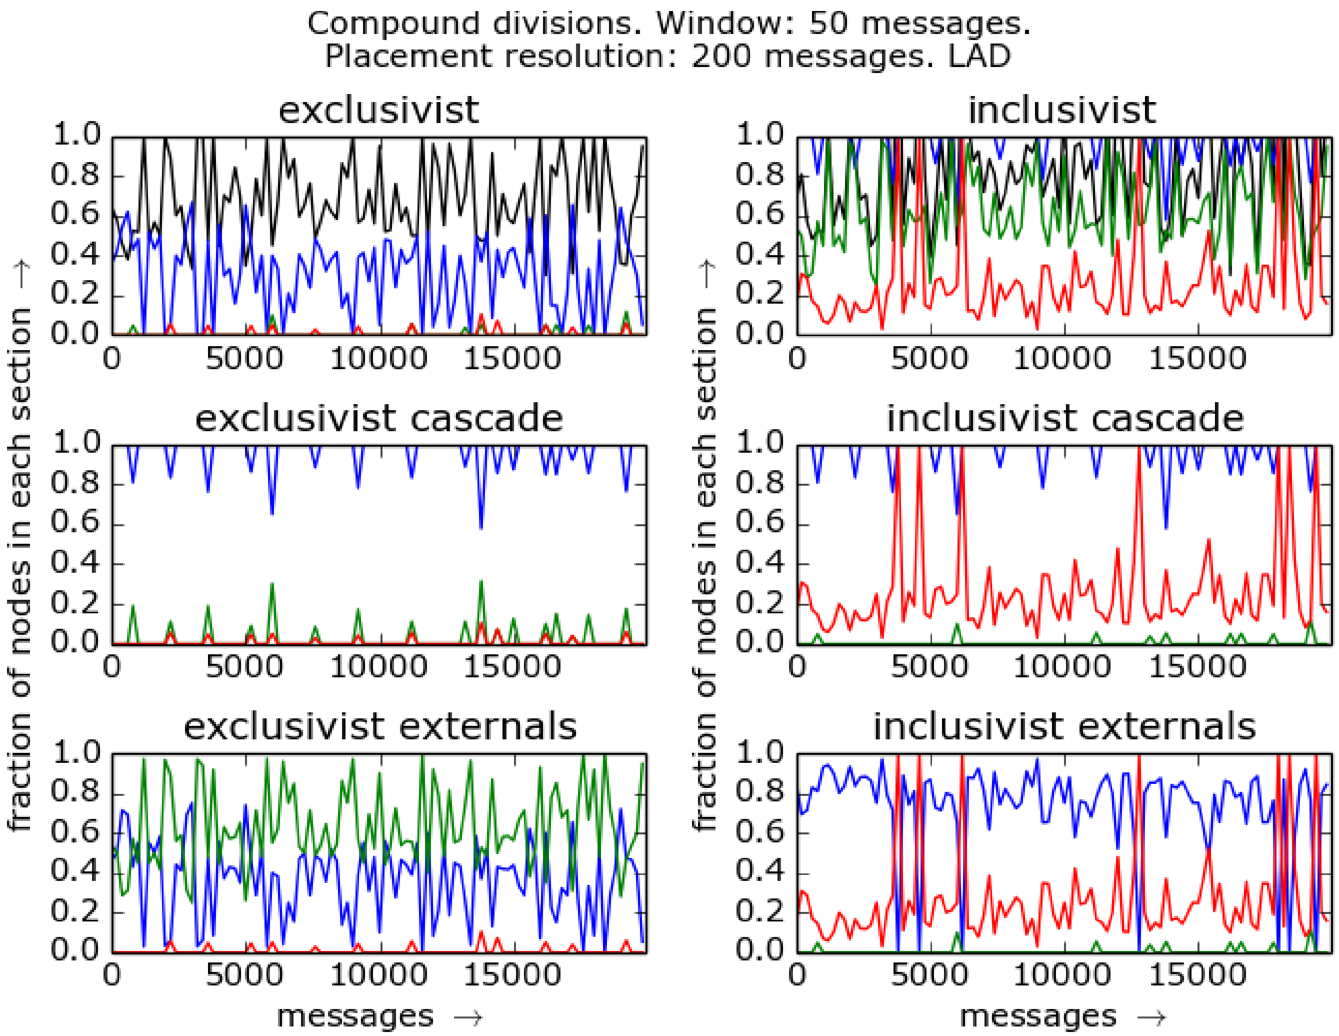
Compound divisions. Window: 50 messages.
Placement resolution: 200 messages. LAD
exclusivist
inclusivist
exclusivist cascade
inclusivist cascade
exclusivist externals
inclusivist externals
fraction of nodes in each section →
messages →
1.0
0.8
0.6
0.4
0.2
0.0
0
5000
10000
15000

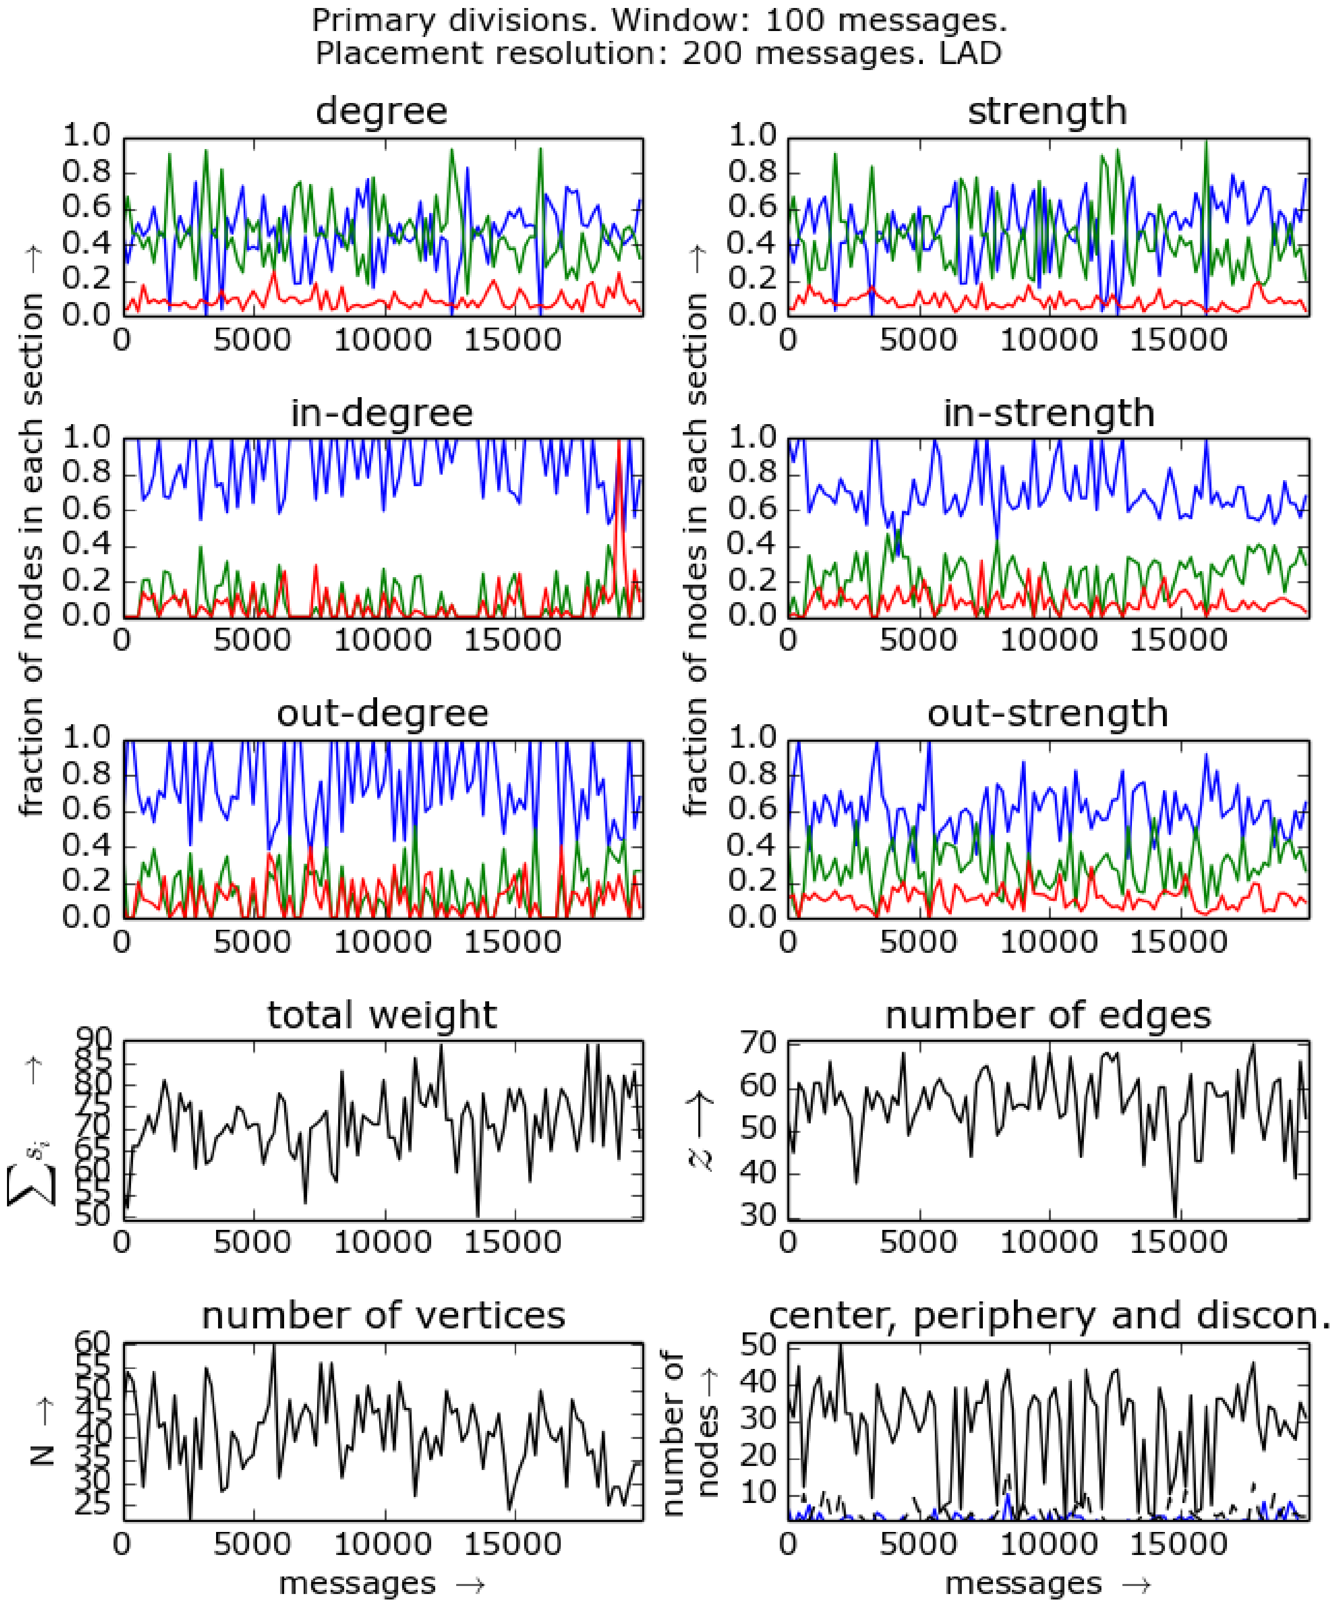
Primary divisions. Window: 100 messages.
Placement resolution: 200 messages. LAD
degree
strength
in-degree
in-strength
out-degree
out-strength
fraction of nodes in each section →
total weight
number of edges
number of vertices
center, periphery and discon.
number of nodes →
N →
messages →

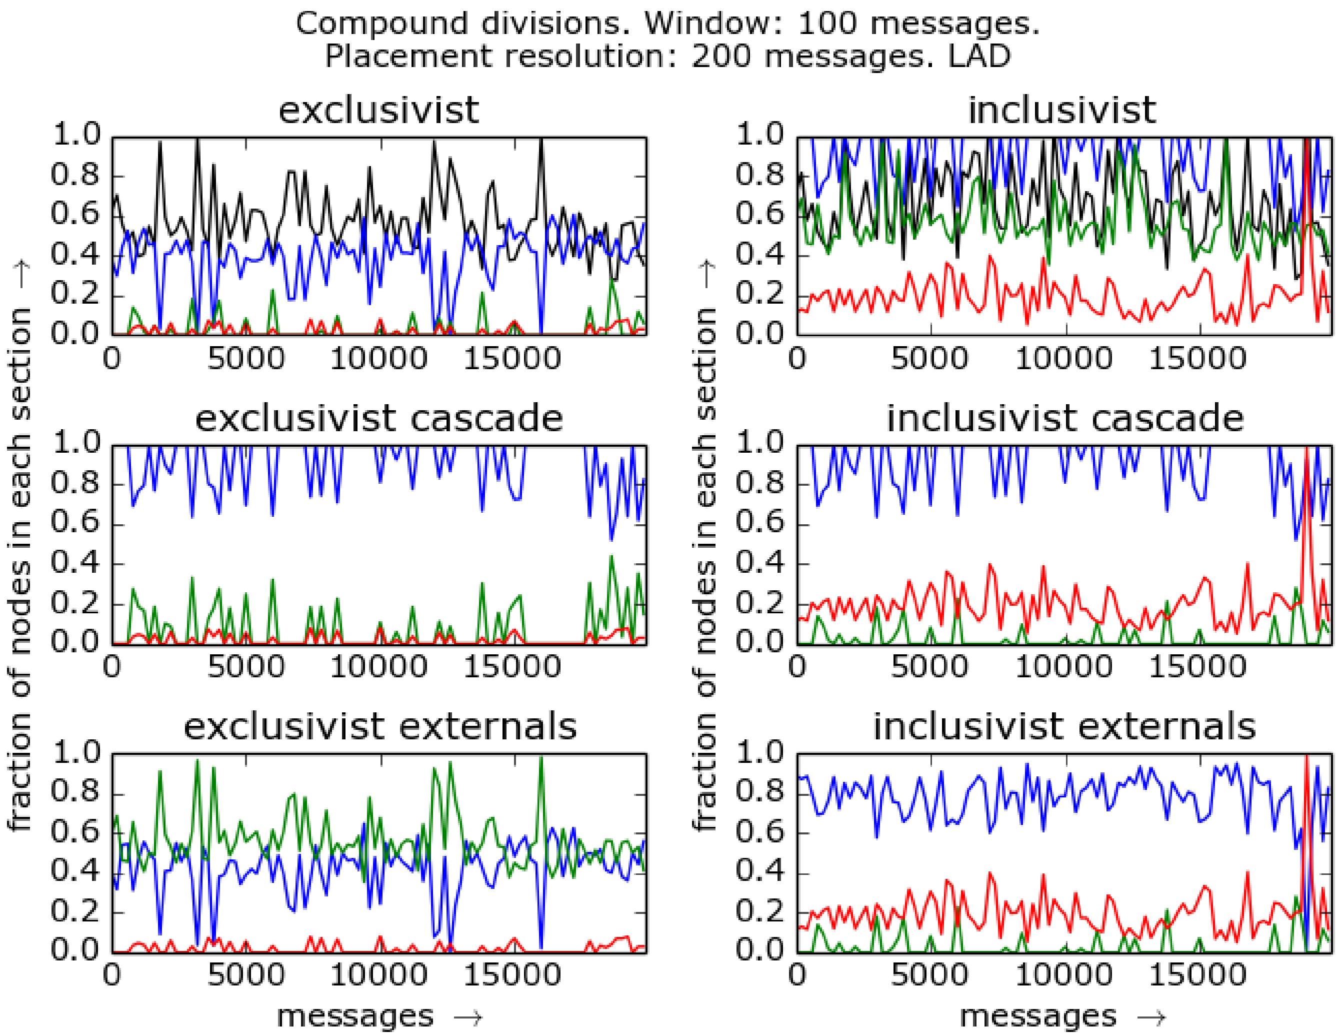
Compound divisions. Window: 100 messages.
Placement resolution: 200 messages. LAD
exclusivist
inclusivist
exclusivist cascade
inclusivist cascade
exclusivist externals
inclusivist externals
fraction of nodes in each section →
messages →
1.0
0.8
0.6
0.4
0.2
0.0
0
5000
10000
15000

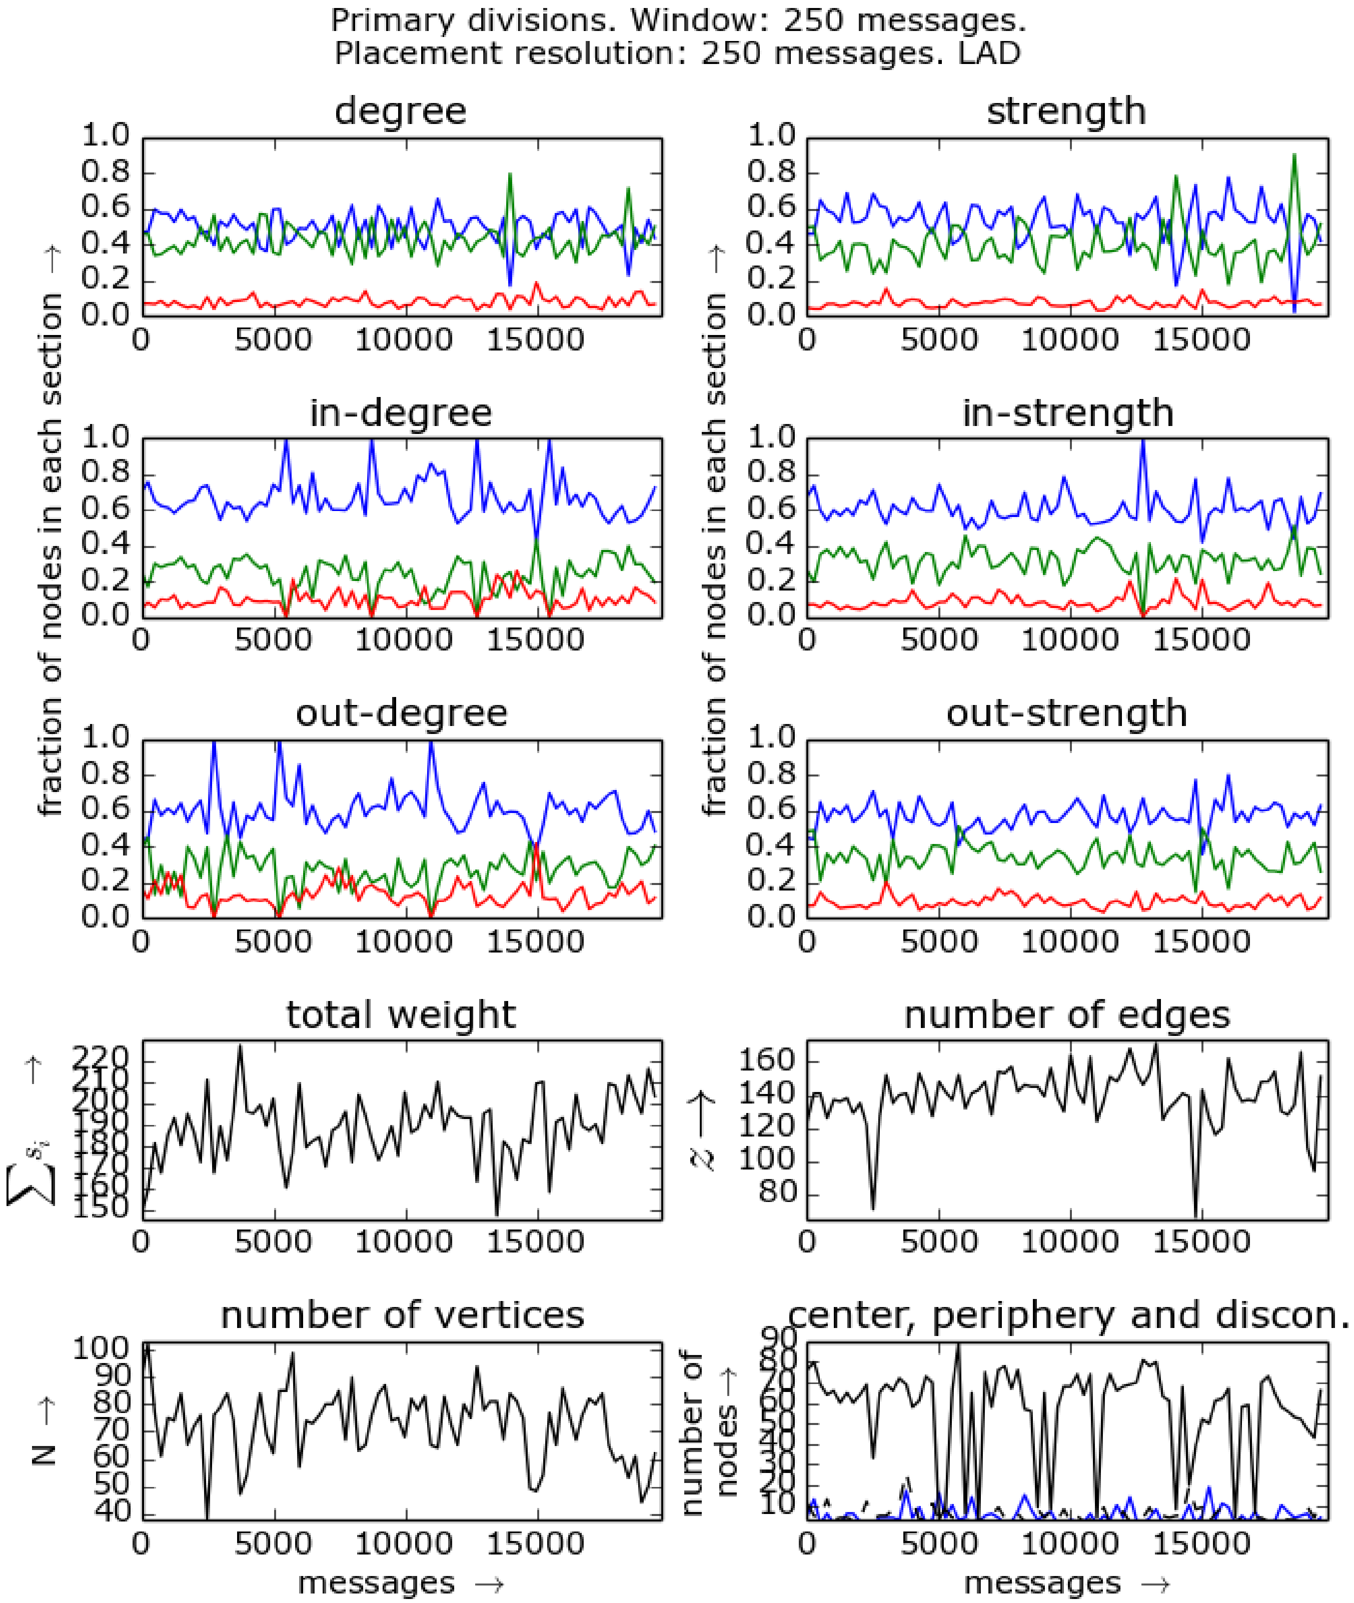
Primary divisions. Window: 250 messages.
Placement resolution: 250 messages. LAD
degree
strength
in-degree
in-strength
out-degree
out-strength
fraction of nodes in each section →
total weight
number of edges
number of vertices
center, periphery and discon.
messages →
N →
number of nodes →

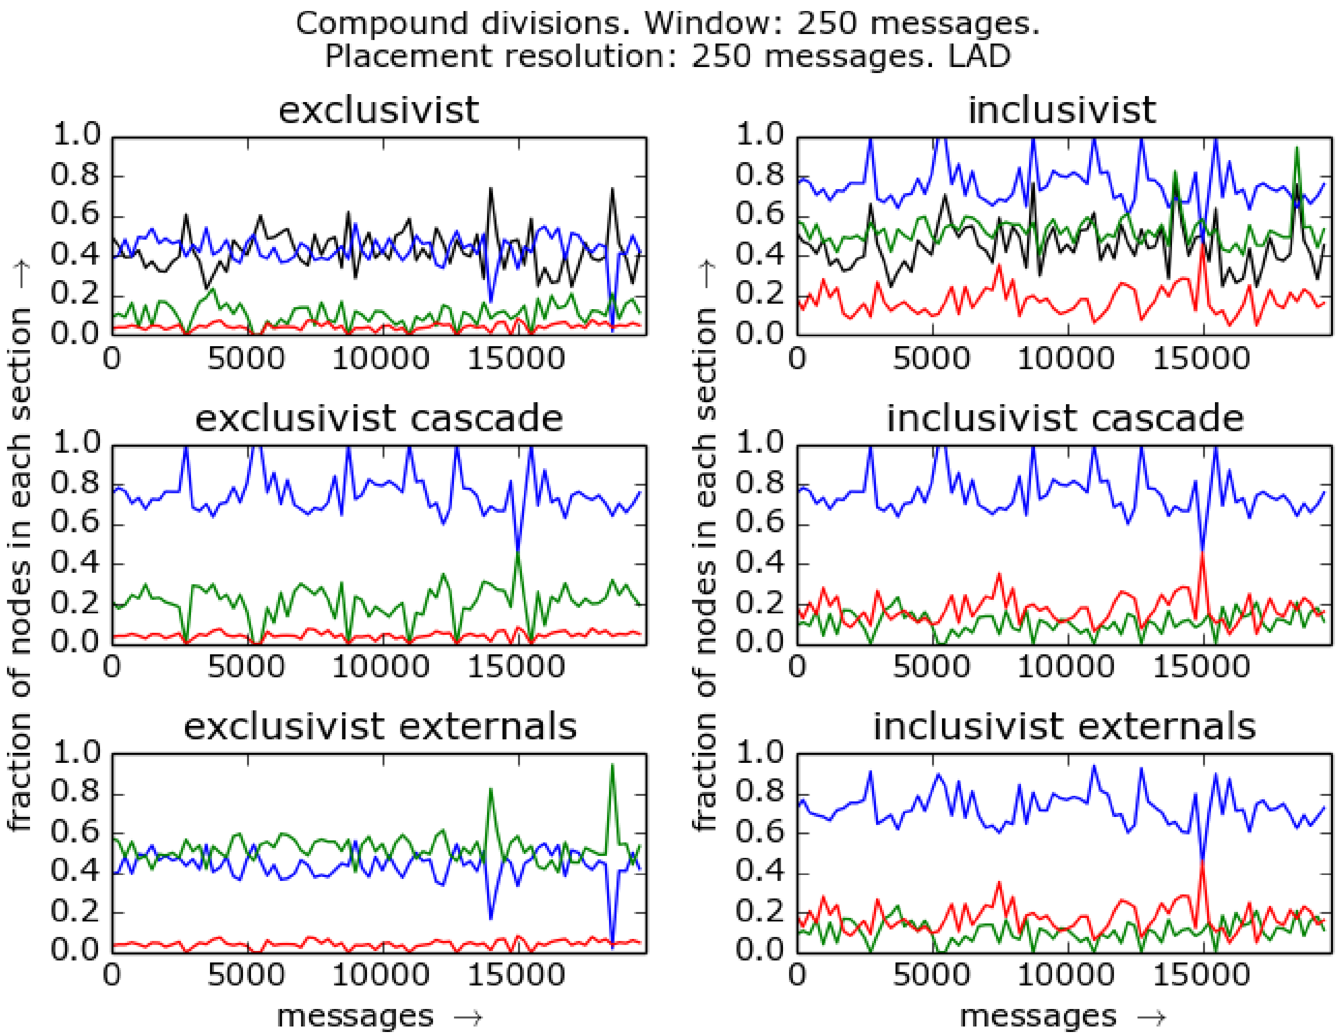
Compound divisions. Window: 250 messages.
Placement resolution: 250 messages. LAD
exclusivist
inclusivist
exclusivist cascade
inclusivist cascade
exclusivist externals
inclusivist externals
fraction of nodes in each section →
messages →
0.0
0.2
0.4
0.6
0.8
1.0
0
5000
10000
15000

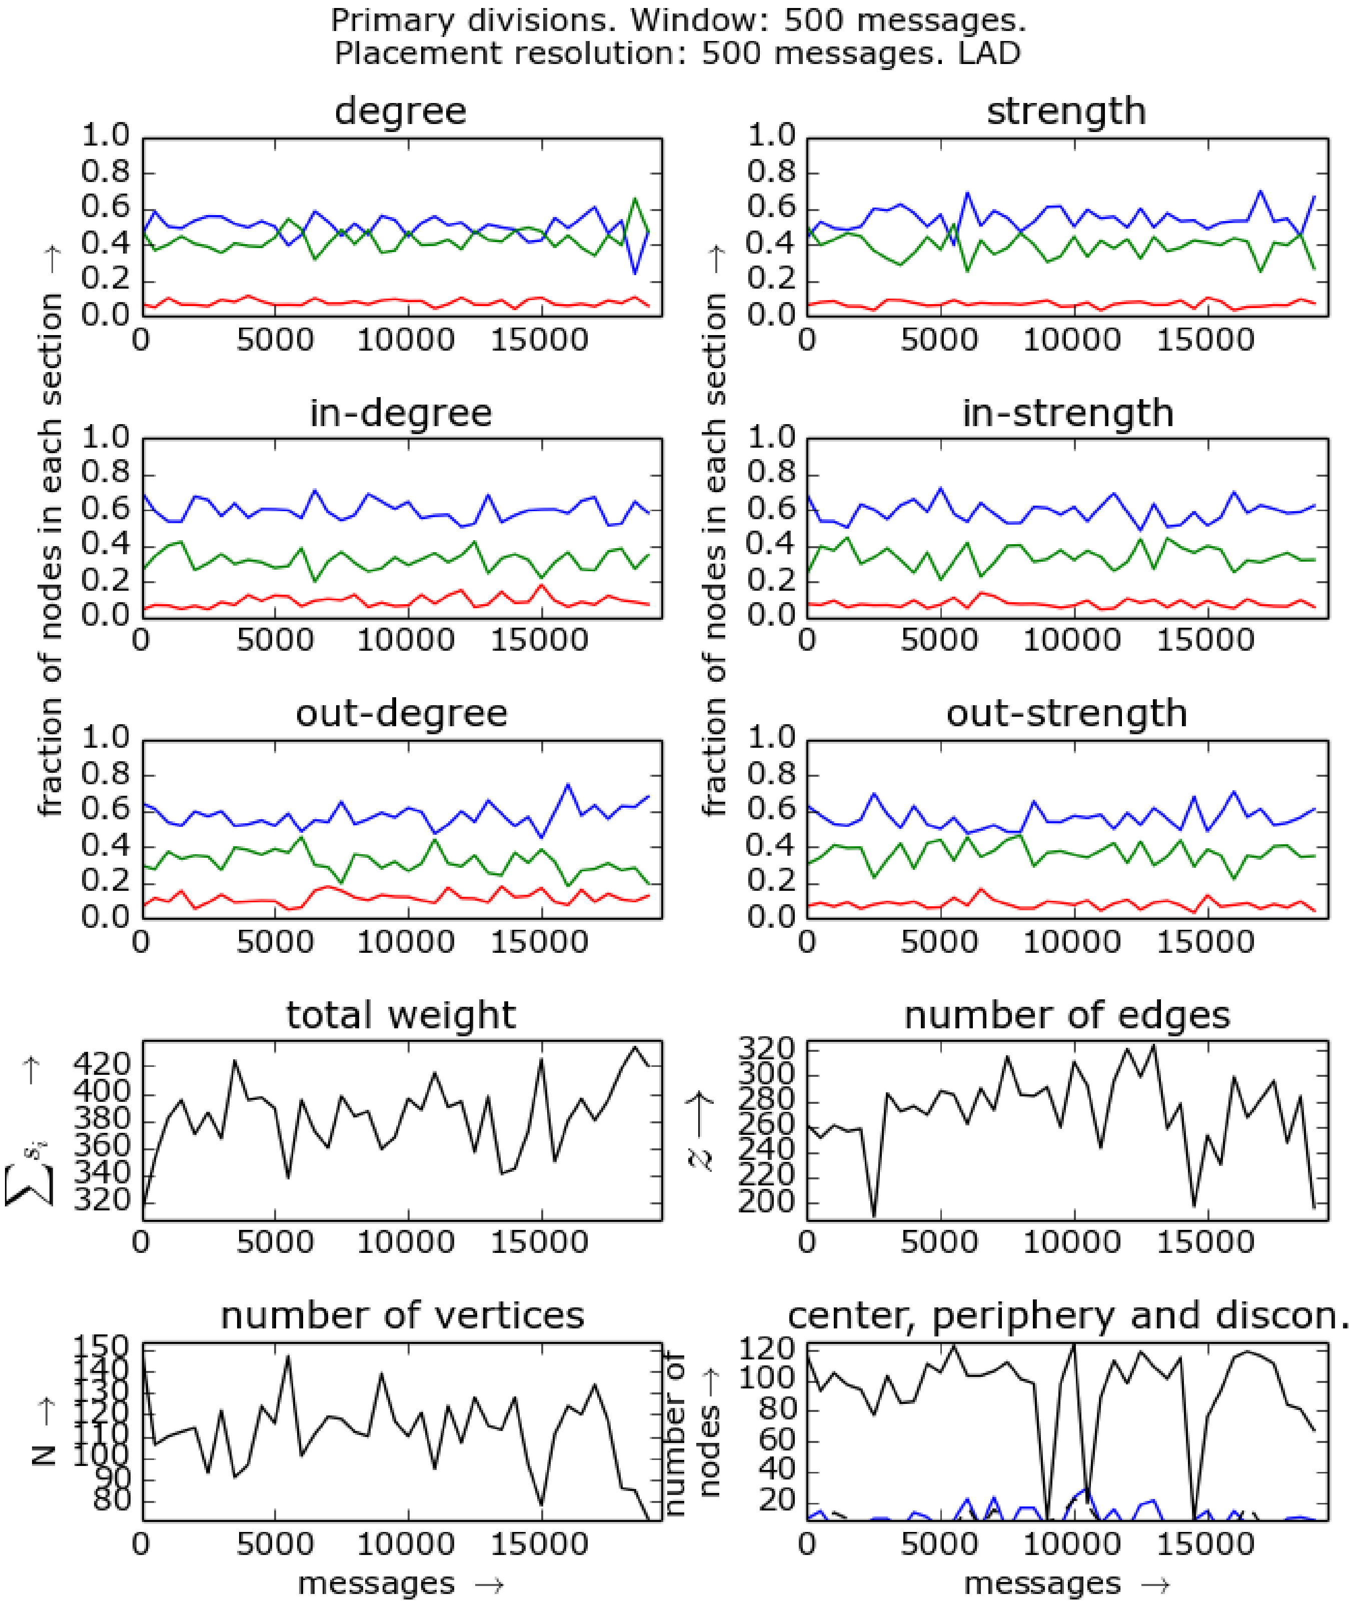
Primary divisions. Window: 500 messages.
Placement resolution: 500 messages. LAD
degree
strength
in-degree
in-strength
out-degree
out-strength
fraction of nodes in each section →
total weight
number of edges
number of vertices
center, periphery and discon.
number of nodes →
messages →

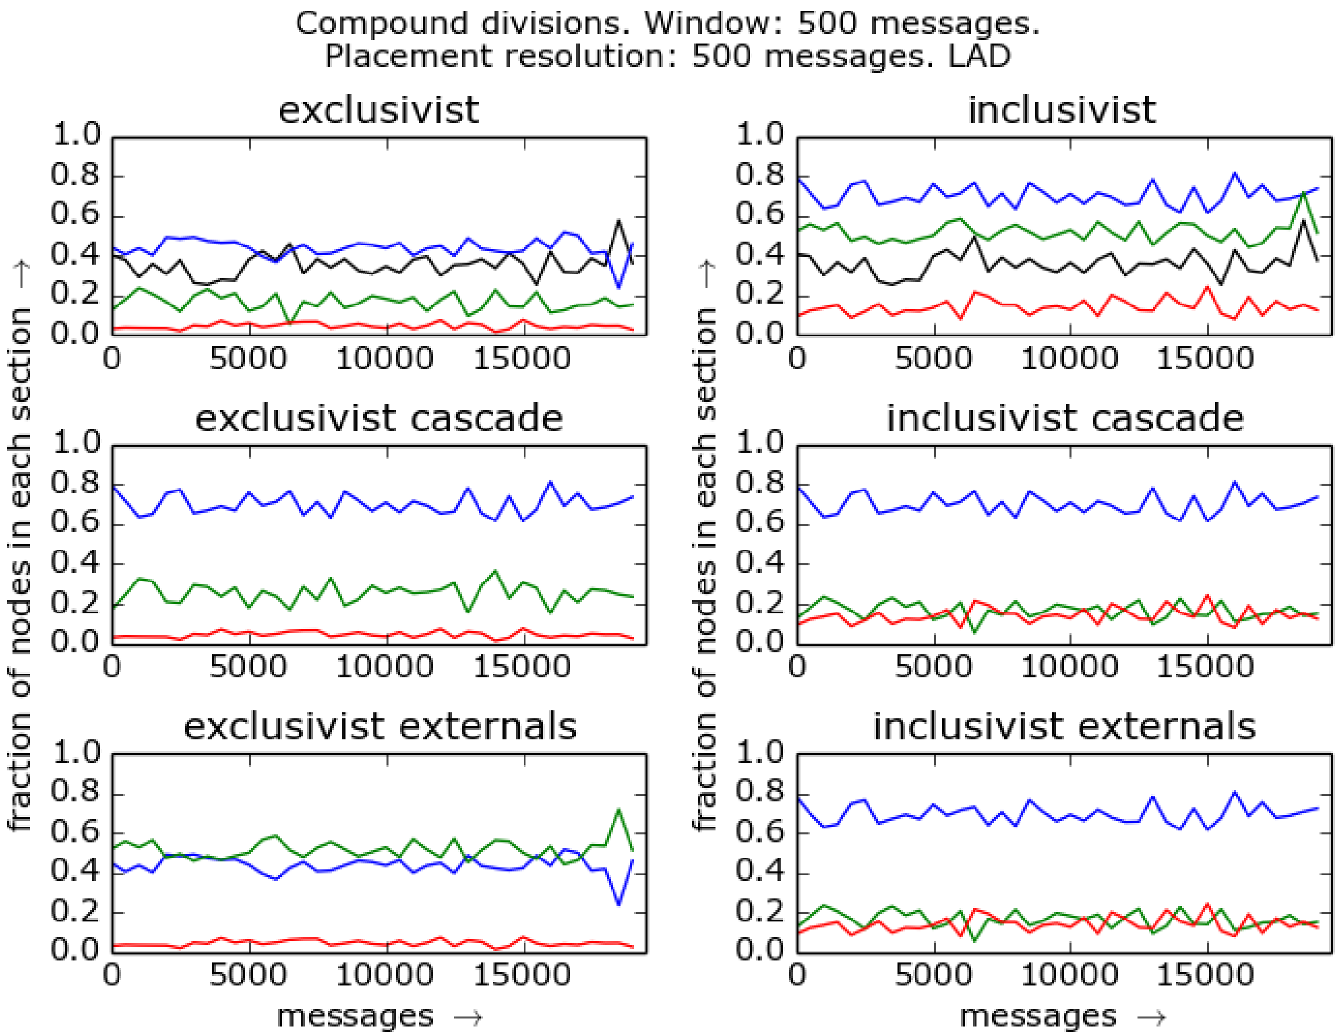
Compound divisions. Window: 500 messages.
Placement resolution: 500 messages. LAD
exclusivist
inclusivist
exclusivist cascade
inclusivist cascade
exclusivist externals
inclusivist externals
fraction of nodes in each section →
messages →
0.0
0.2
0.4
0.6
0.8
1.0
0
5000
10000
15000

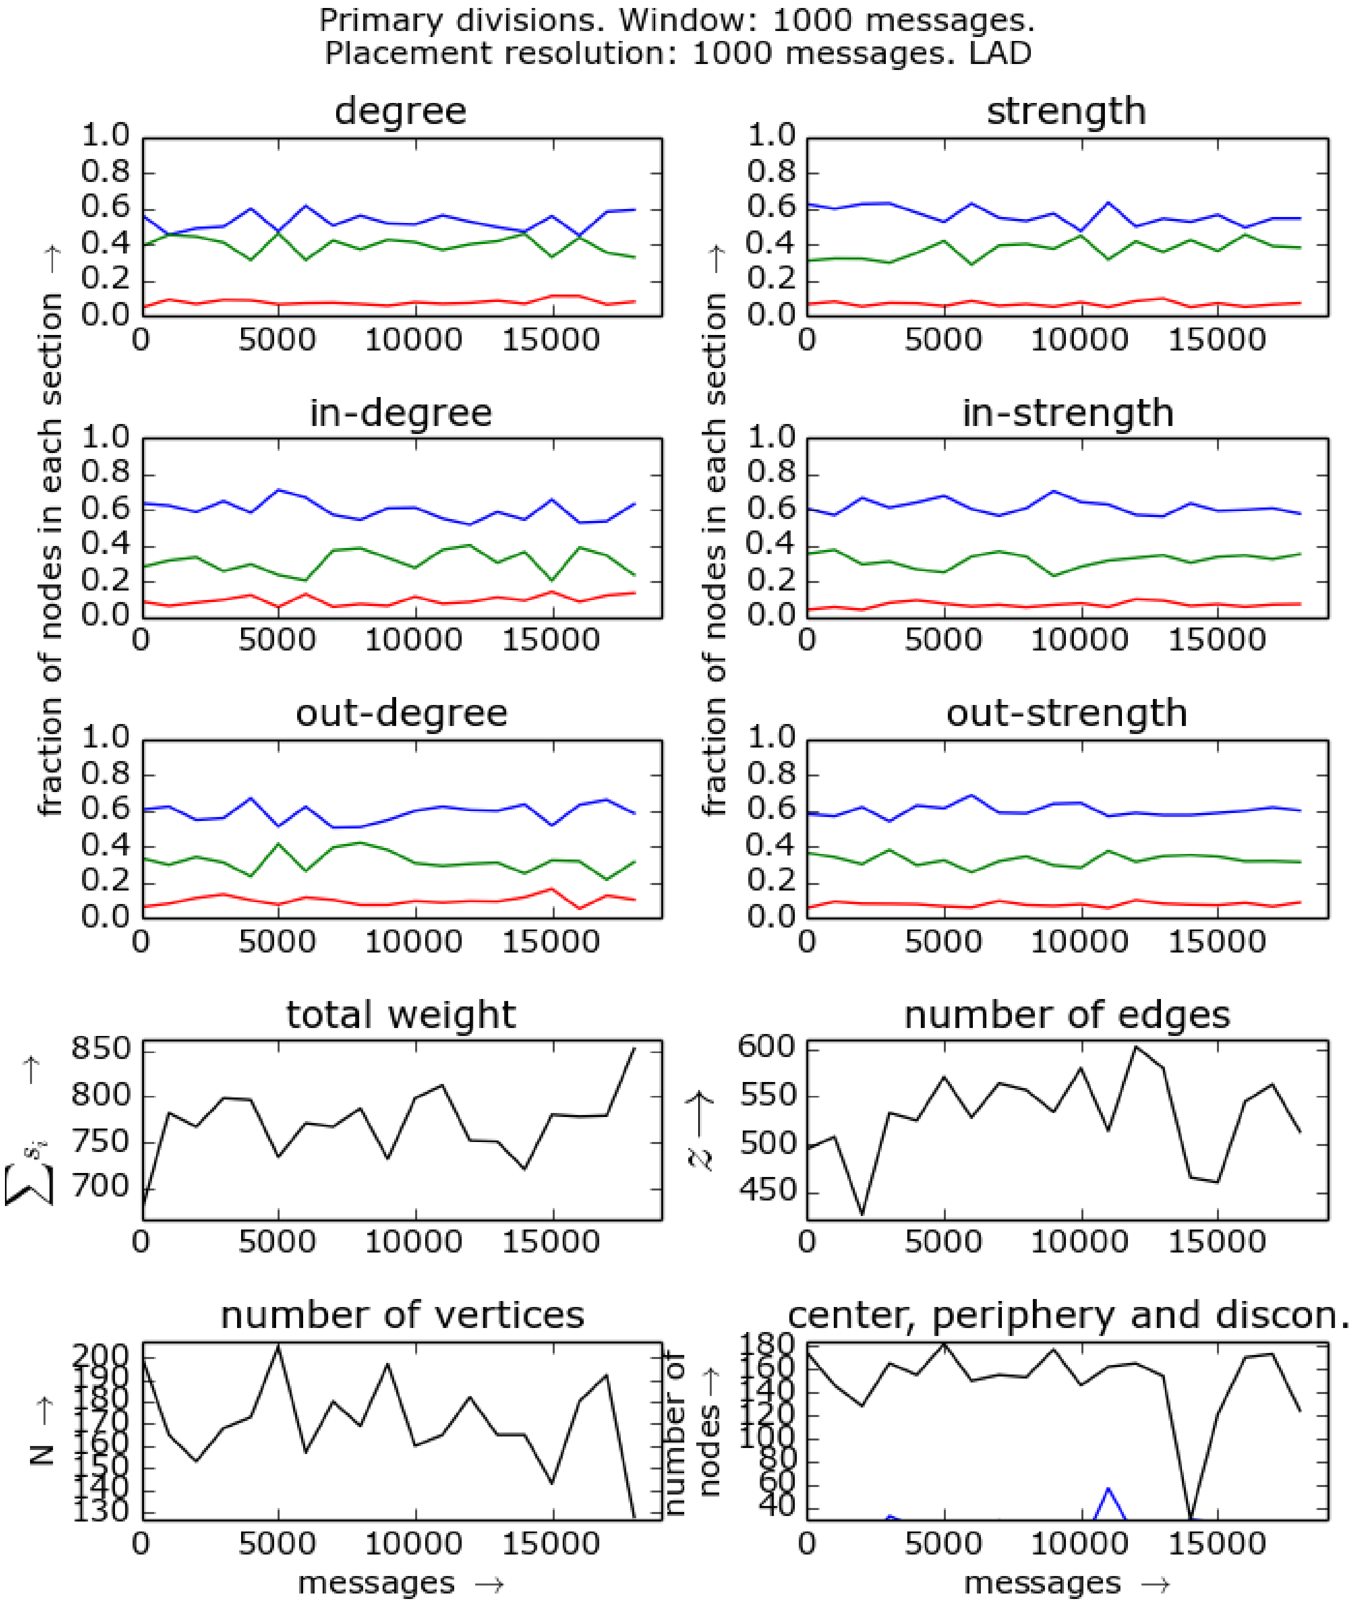
Primary divisions. Window: 1000 messages.
Placement resolution: 1000 messages. LAD
degree
strength
in-degree
in-strength
out-degree
out-strength
fraction of nodes in each section →
total weight
number of edges
number of vertices
center, periphery and discon.
messages →
number of nodes →
N →

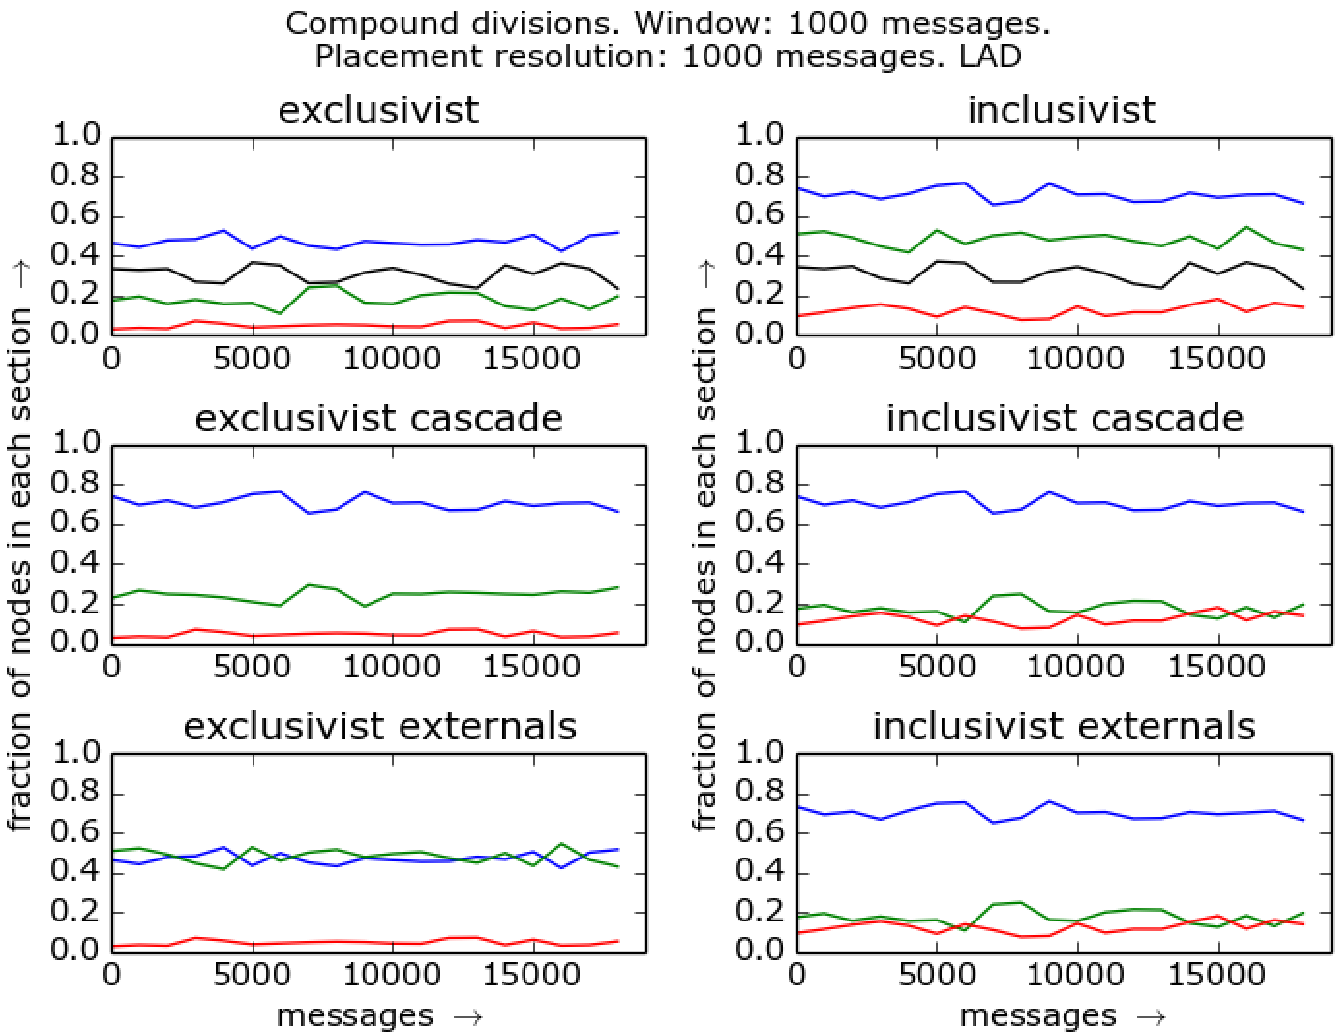
Compound divisions. Window: 1000 messages.
Placement resolution: 1000 messages. LAD
exclusivist
inclusivist
exclusivist cascade
inclusivist cascade
exclusivist externals
inclusivist externals
fraction of nodes in each section →
messages →
0.0
0.2
0.4
0.6
0.8
1.0
0
5000
10000
15000

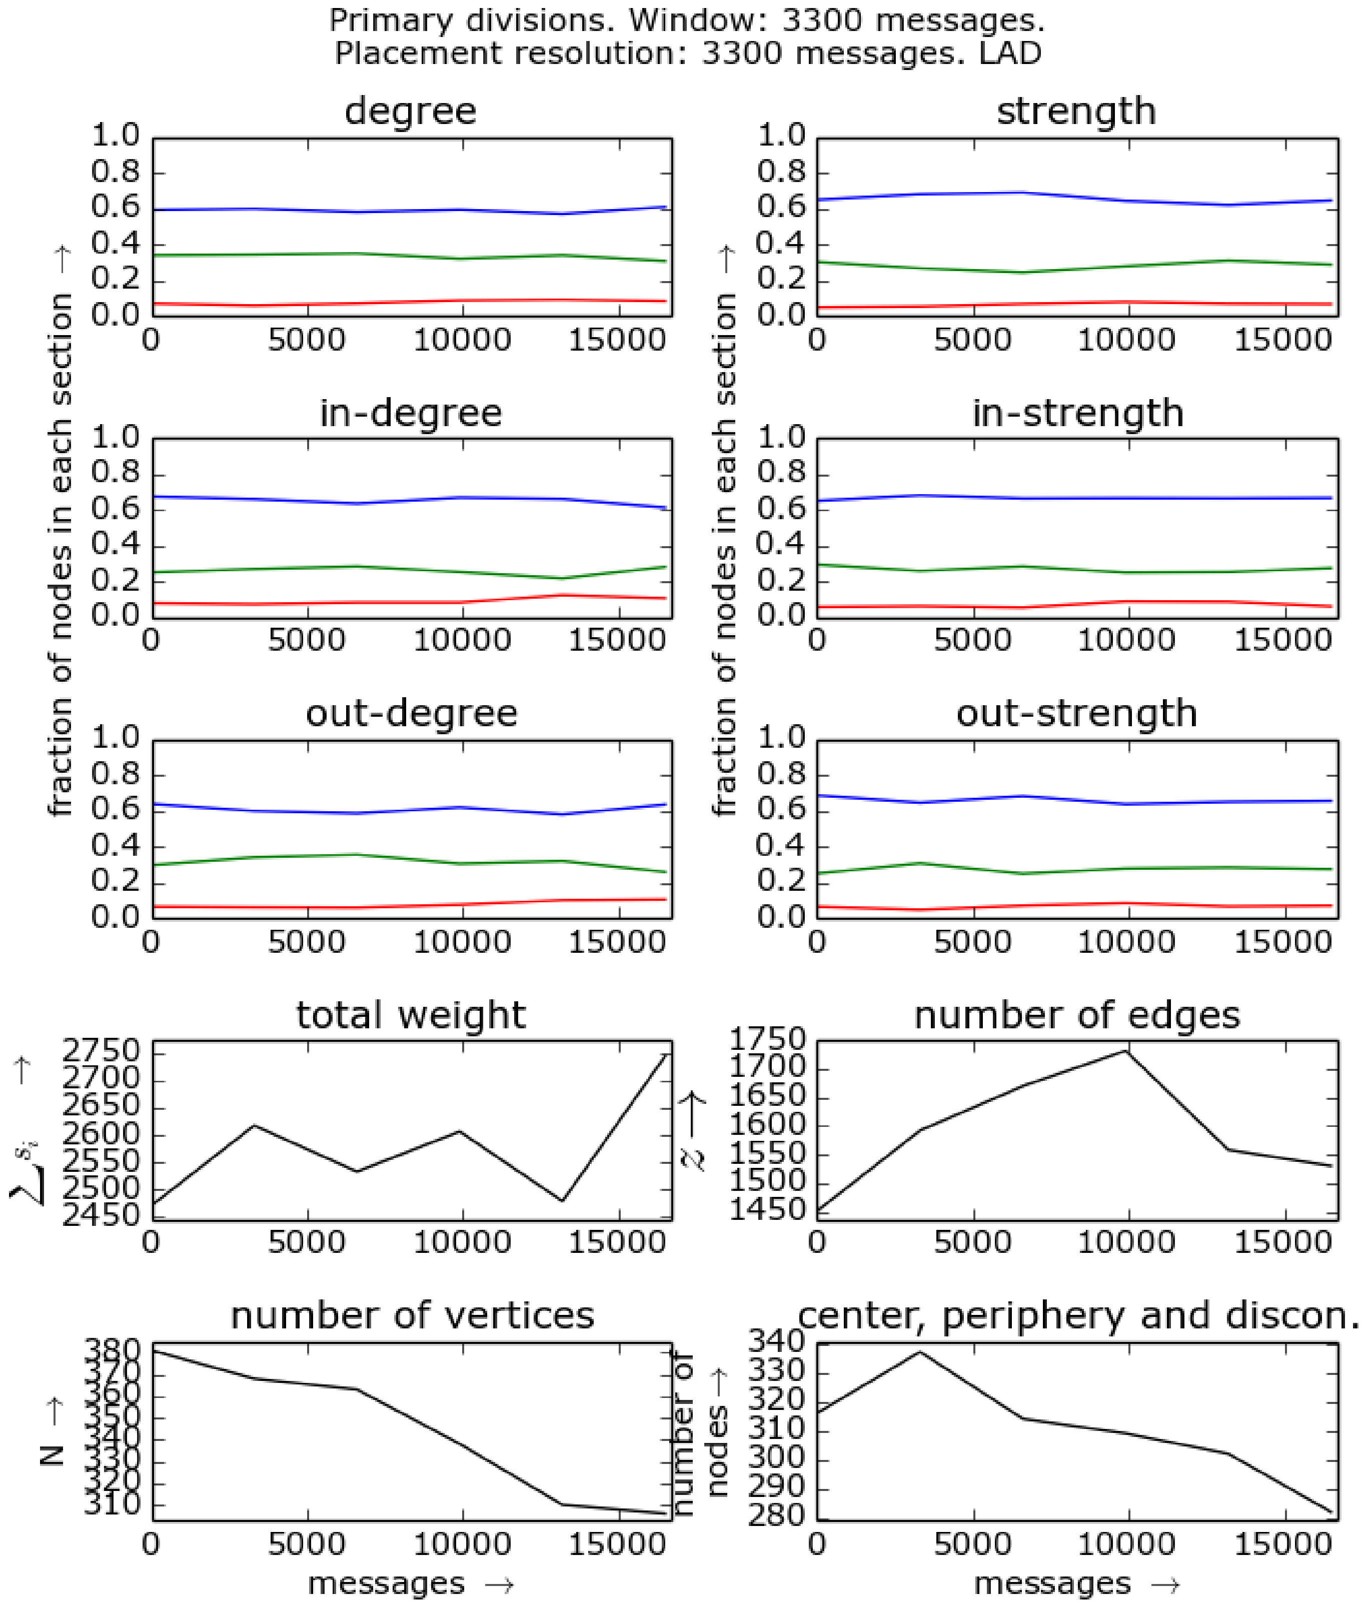
Primary divisions. Window: 3300 messages.
Placement resolution: 3300 messages. LAD
degree
strength
in-degree
in-strength
out-degree
out-strength
fraction of nodes in each section →
total weight
number of edges
number of vertices
center, periphery and discon.
N →
number of nodes →
messages →

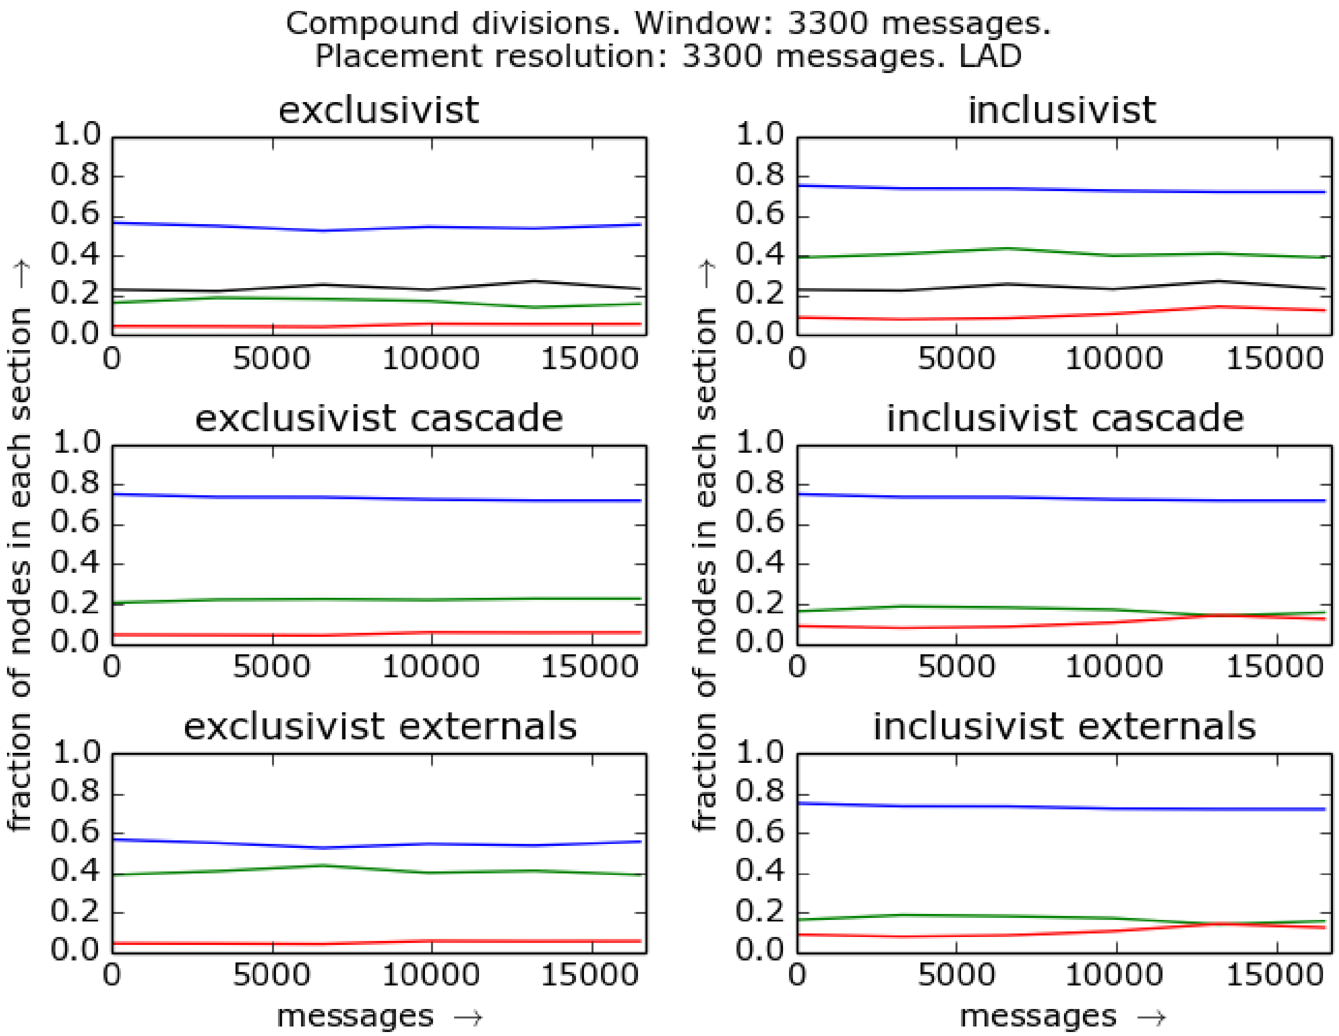
Compound divisions. Window: 3300 messages.
Placement resolution: 3300 messages. LAD
exclusivist
inclusivist
exclusivist cascade
inclusivist cascade
exclusivist externals
inclusivist externals
fraction of nodes in each section →
messages →
0.0
0.2
0.4
0.6
0.8
1.0
0
5000
10000
15000

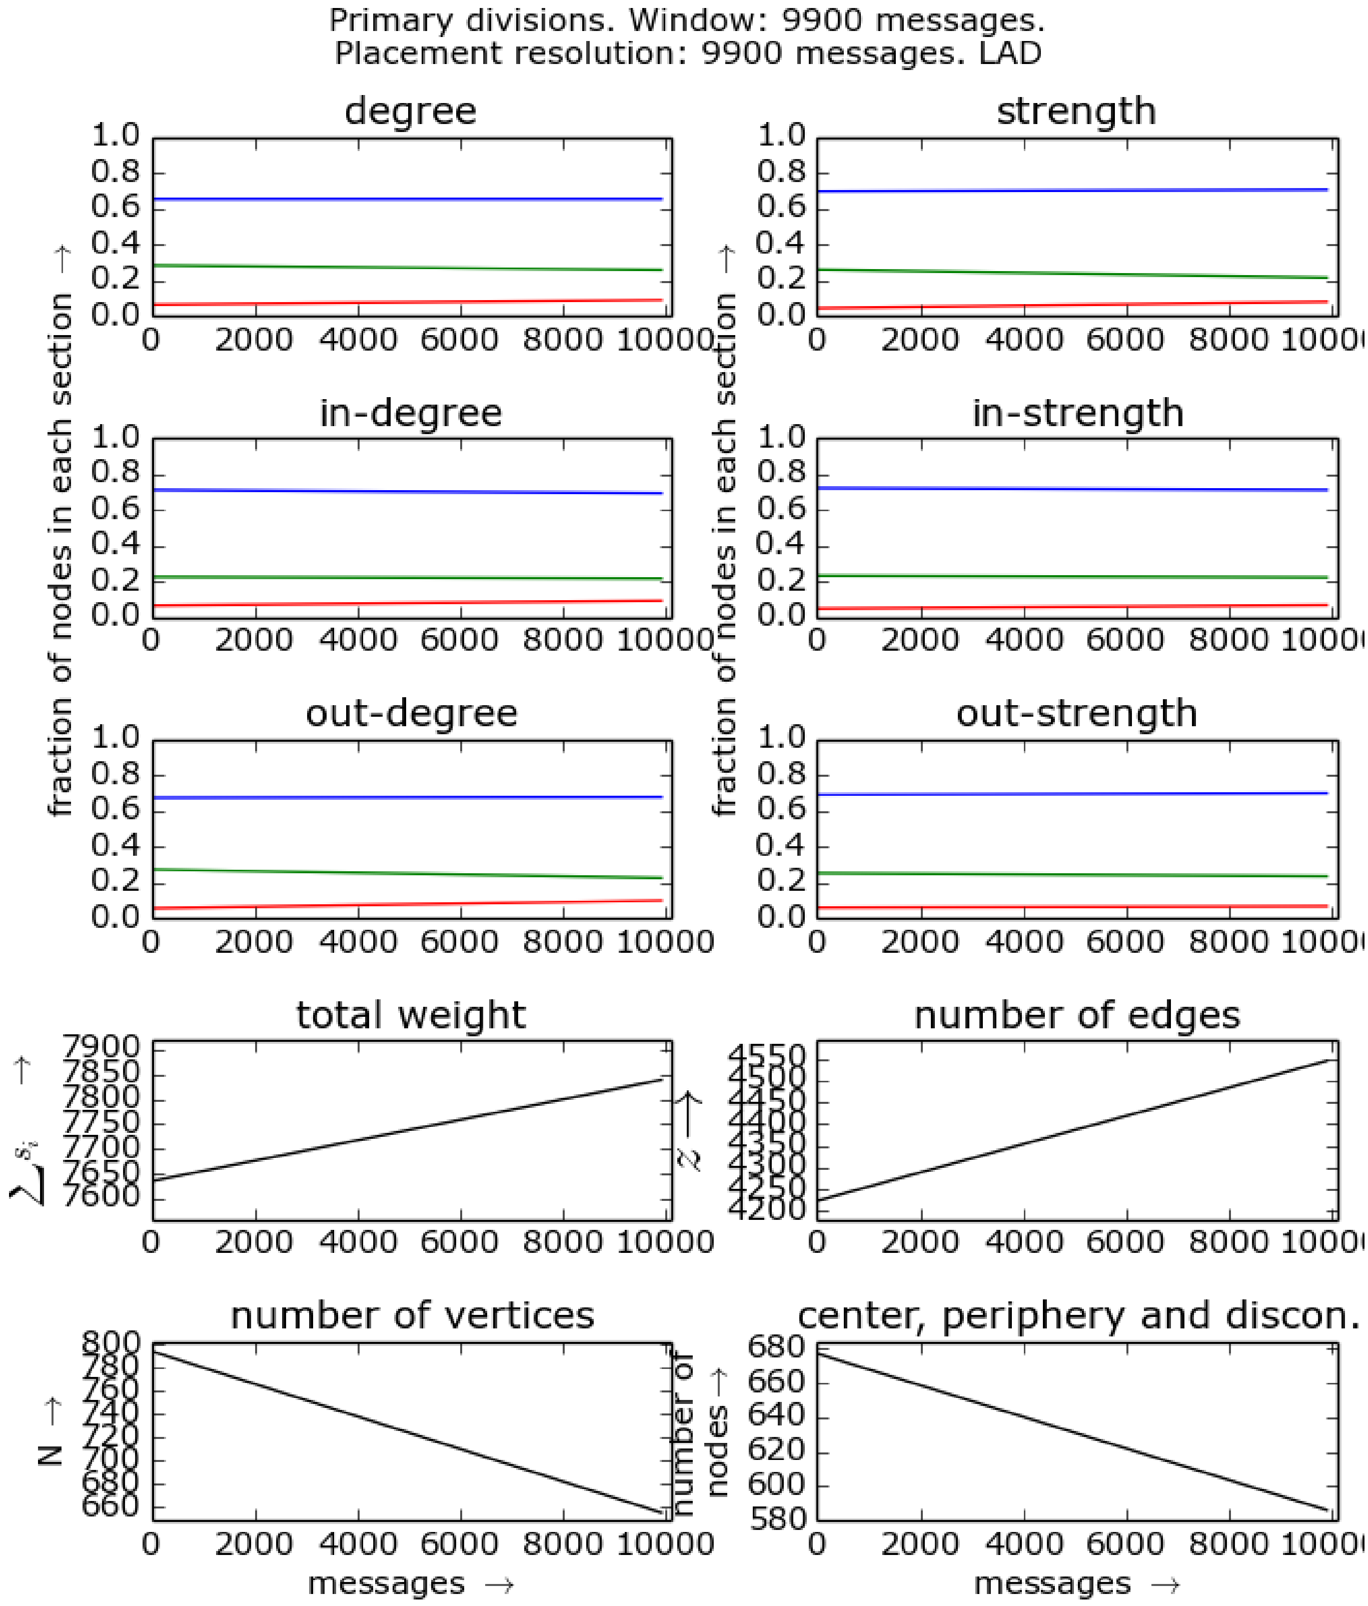

Primary divisions. Window: 9900 messages.
Placement resolution: 9900 messages. LAD
degree
strength
in-degree
in-strength
out-degree
out-strength
fraction of nodes in each section →
total weight
number of edges
number of vertices
center, periphery and discon.
$\sum s_i$ →
$z$ →
N →
number of nodes →
messages →

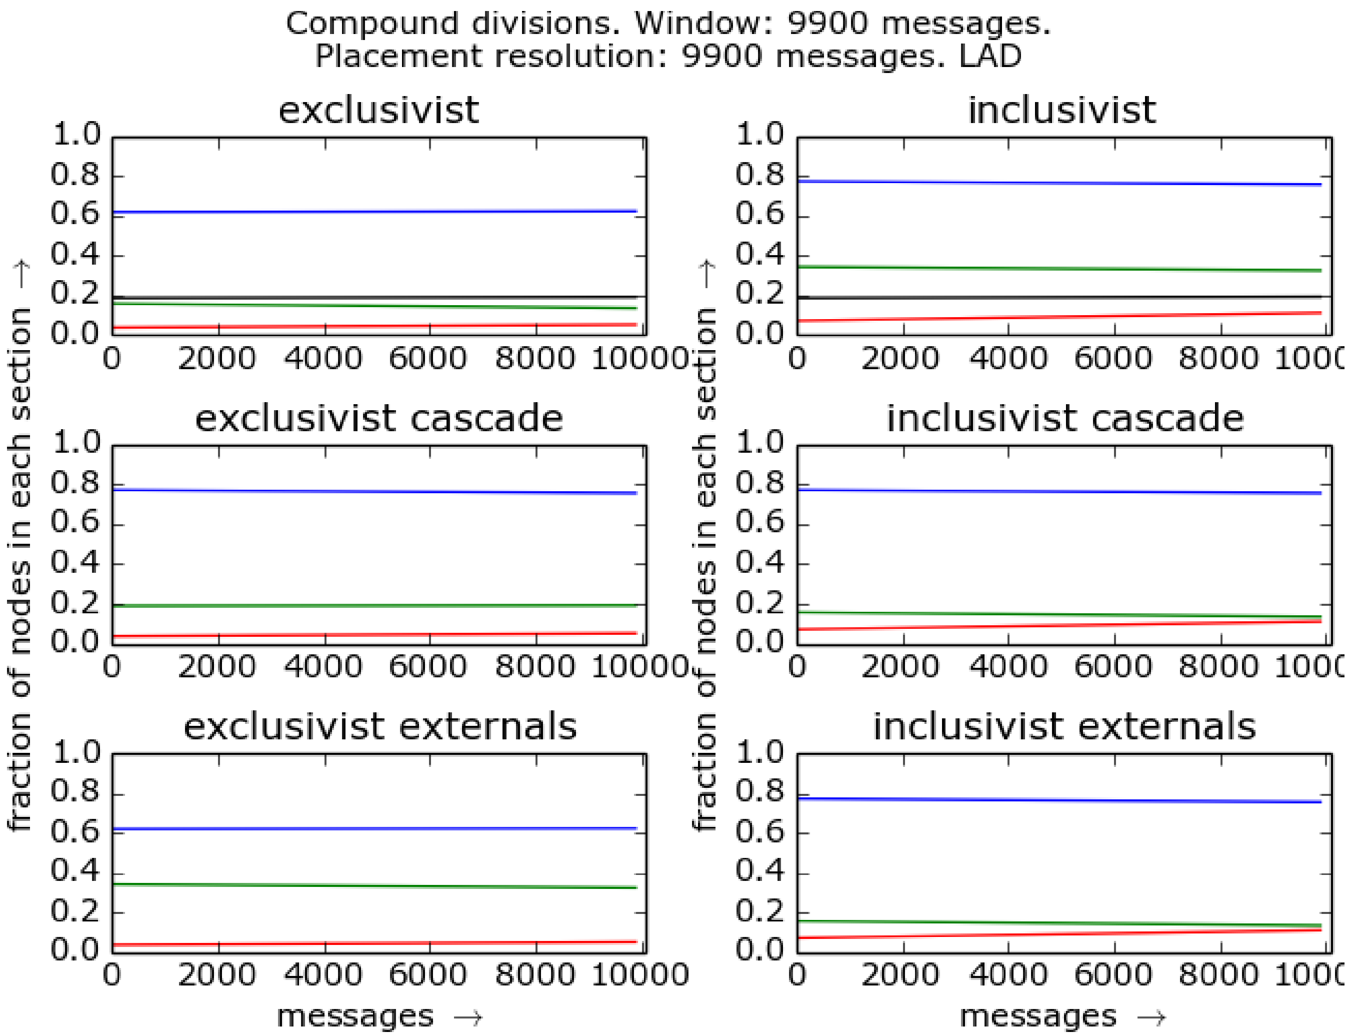
Compound divisions. Window: 9900 messages.
Placement resolution: 9900 messages. LAD
exclusivist
inclusivist
exclusivist cascade
inclusivist cascade
exclusivist externals
inclusivist externals
fraction of nodes in each section →
messages →
1.0
0.8
0.6
0.4
0.2
0.0
0
2000
4000
6000
8000
10000

## IV. STABILITY IN OTHER NETWORKS: TWITTER, FACEBOOK, PARTICIPA.BR

To further verify the hypothesis that such stability is a general property of human social networks, we analyzed networks from Twitter, Facebook and Participa.br. Selected networks are summarized in Table S29. Their Erdös sector relative sizes are given in Table S30. PCA formations are given in Tables S31, S32, S33 and S34. The friendship networks considered are undirected and unweighted, therefore all measurements of strength, in- and out- centralities, asymmetry and disequilibrium have little or no meaning, which is why F1, F2, F3, F4 and F5 are only present in Table S31. The most important results from this analysis are:

- a further indicative that the stability reported with a focus on email interaction networks is valid for a broader class of phenomena.
- The stability in email interaction networks is higher than for the other networks, considering the same number of participants. This is especially important for benchmarking and probing general properties.

TABLE S29. Overview of selected networks analyzed in addition to email interaction networks. Three social platforms were the sources of network structures: Facebook, Twitter and Participa.br. Both friendship and interaction networks were observed, yielding undirected and directed networks, respectively. The number of agents $N$ and the number of edges $z$ are given on the last columns. The acronyms, one for each network, are used throughout Tables S30, S32, S31, S33 and S34. All the data were collected in 2013 and 2014 within the anthropological physics framework[2].

| acronym | provenance | edge | directed | description | $N$ | $z$ |
|---|---|---|---|---|---|---|
| F1 | Facebook | friendship | no | the friendship network of Renato Fabbri (author) | 1367 | 28606 |
| F2 | Facebook | friendship | no | the friendship network of Massimo Canevacci (senior anthropologist) | 4764 | 59995 |
| F3 | Facebook | friendship | no | the friendship network of a brazilian direct democracy group | 3599 | 59471 |
| F4 | Facebook | friendship | no | the friendship network of the Silicon Valley Global Network group | 2026 | 15586 |
| F5 | Participa.br | friendship | no | the friendship network of a brazilian federal social participation portal | 443 | 910 |
| I1 | Facebook | interaction | yes | the interaction network of the Silicon Valley Global Network group | 104 | 154 |
| I2 | Facebook | interaction | yes | the interaction network of a Solidarity Economy group | 64 | 120 |
| I3 | Facebook | interaction | yes | the interaction network of a brazilian direct democracy group | 214 | 310 |
| I4 | Facebook | interaction | yes | the interaction network of the 'Cience with Frontiers' group | 530 | 1658 |
| I5 | Participa.br | interaction | yes | the interaction network of a brazilian federal social participation portal | 222 | 300 |
| TT1 | Twitter | retweet | yes | the retweet network of $\approx 22k$ tweets with the hashtag #arenaNETmundial | 2772 | 7222 |
| TT2 | Twitter | retweet | yes | same as TT1, but disconnected agents are not discarded | 2975 | 7222 |

TABLE S30. Percentage of agents in each Erdös sector in the friendship and interaction human networks of Table S29. The ratios found in email networks are preserved. I1 and I4 are outliers, probably because they should be better characterized as a superposition of networks, rather than one coherent network. The degree was used for establishing the sectors.

| | periphery | intermediary | hubs |
|---|---|---|---|
| F1 | 53.11 | 43.31 | 3.58 |
| F2 | 58.98 | 39.29 | 1.72 |
| F3 | 65.41 | 31.87 | 2.72 |
| F4 | 66.49 | 32.03 | 1.48 |
| F5 | 62.98 | 36.12 | 0.90 |
| I1 | 4.81 | 94.23 | 0.96 |
| I2 | 53.12 | 45.31 | 1.56 |
| I3 | 58.41 | 40.19 | 1.40 |
| I4 | 39.06 | 59.43 | 1.51 |
| I5 | 54.95 | 43.69 | 1.35 |
| TT1 | 74.86 | 24.49 | 0.65 |
| TT2 | 76.57 | 22.86 | 0.57 |

TABLE S31. First three principal components and variance concentration for each of the five friendship networks of Table S29 in the simplest case: dimensions correspond to degree, clustering coefficient and betweenness centrality. Participa.br yields the networks that most resemble the email networks. Overall, the general characteristic is preserved: first component is an average of degree and betweenness, while clustering is the most relevant for the second component. The friendship network of Renato Fabbri (F1) is the only network whose first component has more than 20% of clustering coefficient and second component has more than 40% of degree centrality.

| | PC1 | | | | | PC2 | | | | | PC3 | | | | |
|---|---|---|---|---|---|---|---|---|---|---|---|---|---|---|---|
| | F1 | F2 | F3 | F4 | F5 | F1 | F2 | F3 | F4 | F5 | F1 | F2 | F3 | F4 | F5 |
| $cc$ | 25.80 | 12.22 | 11.54 | 5.04 | 0.94 | 58.87 | 78.22 | 68.86 | 90.39 | 88.86 | 6.95 | 1.13 | 18.20 | 3.02 | 5.90 |
| $k$ | 36.43 | 43.96 | 45.61 | 47.40 | 49.50 | 25.66 | 9.98 | 6.10 | 7.63 | 6.42 | 44.94 | 49.52 | 42.00 | 48.41 | 47.02 |
| $bt$ | 37.77 | 43.82 | 42.85 | 47.56 | 49.56 | 15.46 | 11.80 | 25.04 | 1.98 | 4.72 | 48.11 | 49.35 | 39.80 | 48.57 | 47.08 |
| $\lambda$ | 53.15 | 53.06 | 46.26 | 55.36 | 63.80 | 28.69 | 32.57 | 34.27 | 33.25 | 33.57 | 18.16 | 14.37 | 19.47 | 11.38 | 2.63 |

TABLE S32. First three principal components and variance concentration for each of the seven interaction networks of Table S29 in the simplest case: dimensions correspond to degree, clustering coefficient and betweenness centrality. Twitter yields the networks that most resemble the email networks. Overall, the general characteristic is preserved: first component is an average of degree and betweenness, while clustering is the most relevant for the second component.

| | PC1 | | | | | | | PC2 | | | | | | | PC3 | | | | | | |
|---|---|---|---|---|---|---|---|---|---|---|---|---|---|---|---|---|---|---|---|---|---|
| | I1 | I2 | I3 | I4 | I5 | TT1 | TT2 | I1 | I2 | I3 | I4 | I5 | TT1 | TT2 | I1 | I2 | I3 | I4 | I5 | TT1 | TT2 |
| $cc$ | 14.43 | 17.12 | 11.54 | 0.69 | 13.26 | 2.17 | 2.72 | 74.78 | 70.72 | 79.30 | 96.63 | 76.59 | 95.75 | 94.69 | 1.58 | 4.09 | 2.46 | 1.71 | 0.57 | 2.03 | 2.20 |
| $k$ | 42.68 | 41.77 | 44.37 | 49.65 | 43.41 | 48.94 | 48.67 | 13.85 | 11.48 | 8.31 | 2.35 | 11.26 | 0.14 | 0.52 | 49.07 | 48.42 | 48.94 | 49.14 | 49.76 | 49.01 | 48.93 |
| $bt$ | 42.89 | 41.11 | 44.09 | 49.66 | 43.34 | 48.89 | 48.61 | 11.37 | 17.80 | 12.39 | 1.02 | 12.15 | 4.12 | 4.79 | 49.35 | 47.49 | 48.60 | 49.15 | 49.67 | 48.96 | 48.87 |
| $\lambda$ | 64.58 | 61.97 | 56.95 | 62.01 | 50.92 | 64.82 | 64.83 | 31.57 | 30.98 | 32.56 | 33.35 | 32.51 | 33.33 | 33.32 | 3.85 | 7.05 | 10.50 | 4.64 | 16.57 | 1.85 | 1.86 |

TABLE S33. First three principal components and variance concentration for each of the seven interaction networks of Table S29 considering dimensions of in- and out- degrees and strengths, clustering coefficient and betweenness centrality. Twitter yields the networks that most resemble email networks. The general characteristic is preserved: first component is an average of degree and betweenness, while clustering is the most relevant for the second component. Important differences are: - the clustering coefficient was only important to the third component for two of the networks ($I2$, $I3$) and does not contribute significantly to any of the first three principal components in $I5$; - in the first component, I5 exhibited less contribution from in-strength, in-degree and betweenness, I4 exhibited less contribution from out-degree.

| | PC1 | | | | | | | PC2 | | | | | | | PC3 | | | | | | |
|---|---|---|---|---|---|---|---|---|---|---|---|---|---|---|---|---|---|---|---|---|---|
| | I1 | I2 | I3 | I4 | I5 | TT1 | TT2 | I1 | I2 | I3 | I4 | I5 | TT1 | TT2 | I1 | I2 | I3 | I4 | I5 | TT1 | TT2 |
| $cc$ | 2.79 | 4.34 | 2.57 | 0.82 | 1.29 | 0.66 | 0.76 | 28.44 | 9.46 | 3.29 | 21.95 | 6.95 | 29.82 | 30.04 | 32.24 | 60.89 | 80.24 | 43.85 | 3.81 | 33.84 | 33.54 |
| $s$ | 15.28 | 15.84 | 16.46 | 16.01 | 16.70 | 15.49 | 15.47 | 3.78 | 4.95 | 2.90 | 3.26 | 17.78 | 1.95 | 2.05 | 1.95 | 0.34 | 0.87 | 4.84 | 11.15 | 0.52 | 0.43 |
| $s^{in}$ | 14.48 | 12.81 | 13.62 | 14.63 | 4.50 | 11.85 | 11.84 | 11.77 | 18.29 | 17.41 | 12.44 | 16.19 | 19.03 | 18.81 | 5.38 | 5.03 | 0.93 | 11.16 | 30.41 | 21.48 | 21.71 |
| $s^{out}$ | 12.13 | 12.12 | 12.59 | 12.91 | 19.02 | 13.87 | 13.85 | 17.19 | 16.79 | 20.12 | 18.81 | 8.90 | 13.42 | 13.43 | 19.35 | 7.90 | 3.11 | 11.38 | 14.58 | 12.91 | 12.92 |
| $k$ | 15.32 | 16.22 | 16.12 | 16.20 | 21.12 | 15.48 | 15.46 | 3.13 | 4.18 | 6.25 | 2.88 | 9.26 | 3.32 | 3.24 | 1.84 | 0.09 | 1.16 | 0.11 | 2.22 | 4.26 | 4.30 |
| $k^{in}$ | 14.49 | 13.56 | 12.90 | 15.34 | 7.29 | 12.99 | 12.98 | 10.45 | 16.50 | 19.68 | 11.13 | 20.75 | 17.89 | 17.86 | 8.78 | 4.07 | 1.26 | 6.07 | 15.41 | 14.67 | 14.65 |
| $k^{out}$ | 11.70 | 11.25 | 11.80 | 9.24 | 21.09 | 14.20 | 14.19 | 19.14 | 20.50 | 21.19 | 26.13 | 0.19 | 12.36 | 12.28 | 18.80 | 7.50 | 4.68 | 20.44 | 10.57 | 12.14 | 12.20 |
| $bt$ | 13.82 | 13.86 | 13.93 | 14.86 | 8.99 | 15.47 | 15.45 | 6.10 | 9.32 | 9.16 | 3.41 | 19.99 | 2.20 | 2.29 | 11.66 | 14.20 | 7.75 | 2.17 | 11.86 | 0.18 | 0.25 |
| $\lambda$ | 71.73 | 60.58 | 60.35 | 64.53 | 41.28 | 70.06 | 70.08 | 15.23 | 21.53 | 20.13 | 16.42 | 22.83 | 13.83 | 13.86 | 9.95 | 11.37 | 12.25 | 11.19 | 15.71 | 11.43 | 11.38 |

TABLE S34. First three principal components and variance concentration for each of the seven interaction networks of Table S29 considering dimensions of in- and out- degrees and strengths, clustering coefficient, betweenness centrality and symmetry related metrics (see Section III C 1). The characteristics found in email interaction networks are preserved: the first component is an average of degree and betweenness, the second component is mostly governed by symmetry related metrics, and clustering coefficient is mostly relevant for the third component. Standard deviation of asymmetry and disequilibrium metrics are again coupled to clustering coefficient in the third component. Important differences are: - the first component is a less regular average of centrality measures and has a greater contribution of symmetry metrics; - The first component of I5 is formed mostly from symmetry, not centrality, metrics.

| | PC1 | | | | | | | PC2 | | | | | | | PC3 | | | | | | |
|---|---|---|---|---|---|---|---|---|---|---|---|---|---|---|---|---|---|---|---|---|---|
| | I1 | I2 | I3 | I4 | I5 | TT1 | TT2 | I1 | I2 | I3 | I4 | I5 | TT1 | TT2 | I1 | I2 | I3 | I4 | I5 | TT1 | TT2 |
| $cc$ | 3.46 | 4.19 | 2.44 | 0.36 | 2.18 | 1.28 | 1.17 | 3.06 | 1.61 | 1.23 | 1.19 | 2.57 | 3.03 | 2.17 | 17.36 | 16.88 | 21.68 | 17.00 | 10.00 | 18.65 | 19.13 |
| $s$ | 10.05 | 9.21 | 9.60 | 9.31 | 3.54 | 10.27 | 10.59 | 5.81 | 5.74 | 7.33 | 8.47 | 9.24 | 6.26 | 5.96 | 4.58 | 8.02 | 4.91 | 2.21 | 13.10 | 0.92 | 1.53 |
| $s^{in}$ | 9.57 | 8.03 | 9.21 | 8.74 | 0.78 | 7.75 | 7.99 | 4.63 | 0.59 | 1.27 | 6.69 | 2.77 | 5.38 | 5.29 | 8.22 | 12.82 | 9.18 | 6.53 | 7.63 | 5.90 | 4.77 |
| $s^{out}$ | 7.88 | 6.21 | 5.45 | 6.97 | 5.76 | 9.25 | 9.54 | 6.78 | 10.23 | 12.76 | 9.20 | 10.26 | 5.27 | 4.92 | 5.90 | 2.99 | 3.86 | 8.43 | 10.84 | 4.58 | 4.76 |
| $k$ | 10.44 | 10.02 | 9.88 | 10.39 | 5.80 | 10.80 | 11.05 | 4.62 | 5.13 | 5.66 | 5.54 | 14.08 | 4.48 | 4.29 | 3.63 | 6.02 | 6.18 | 1.86 | 1.21 | 1.33 | 1.30 |
| $k^{in}$ | 10.12 | 9.30 | 9.50 | 9.98 | 4.43 | 8.64 | 8.86 | 2.69 | 0.70 | 0.88 | 4.49 | 9.61 | 5.40 | 5.50 | 7.12 | 10.55 | 8.70 | 6.17 | 8.24 | 7.27 | 6.54 |
| $k^{out}$ | 7.27 | 5.29 | 4.43 | 5.43 | 9.11 | 10.10 | 10.33 | 8.36 | 12.52 | 13.63 | 5.65 | 11.61 | 3.38 | 3.08 | 7.82 | 5.77 | 2.07 | 13.52 | 5.68 | 5.00 | 4.65 |
| $bt$ | 9.62 | 7.97 | 7.53 | 8.93 | 2.25 | 10.47 | 10.78 | 3.77 | 8.42 | 9.14 | 6.95 | 8.12 | 5.60 | 5.29 | 2.72 | 0.42 | 1.99 | 2.74 | 8.66 | 1.16 | 1.60 |
| $asy$ | 5.42 | 7.05 | 7.97 | 8.48 | 15.47 | 6.16 | 5.79 | 14.17 | 12.88 | 11.78 | 11.02 | 4.67 | 12.48 | 13.39 | 2.95 | 1.03 | 0.58 | 2.71 | 0.87 | 6.54 | 5.80 |
| $\mu_{asy}$ | 5.48 | 6.99 | 7.99 | 8.47 | 15.44 | 6.18 | 5.80 | 14.12 | 13.04 | 11.78 | 11.01 | 4.72 | 12.46 | 13.37 | 2.92 | 0.76 | 0.75 | 2.77 | 0.76 | 6.58 | 5.83 |
| $\sigma_{asy}$ | 6.53 | 7.39 | 7.63 | 7.15 | 2.37 | 5.59 | 5.48 | 1.69 | 3.80 | 1.75 | 8.46 | 7.49 | 5.94 | 5.45 | 11.32 | 8.91 | 11.14 | 3.04 | 15.54 | 13.70 | 15.31 |
| $dis$ | 5.02 | 6.67 | 7.78 | 8.08 | 15.41 | 5.98 | 5.59 | 14.12 | 13.41 | 11.92 | 11.53 | 4.80 | 12.45 | 13.38 | 4.99 | 1.40 | 0.67 | 3.02 | 0.83 | 7.44 | 6.69 |
| $\mu_{dis}$ | 5.33 | 7.01 | 7.24 | 6.92 | 14.34 | 5.49 | 5.14 | 13.33 | 10.15 | 9.47 | 8.02 | 5.05 | 11.86 | 12.65 | 1.66 | 7.08 | 5.72 | 11.38 | 2.68 | 0.77 | 0.66 |
| $\sigma_{dis}$ | 3.82 | 4.68 | 3.34 | 0.81 | 3.12 | 2.03 | 1.88 | 2.85 | 1.77 | 1.39 | 1.77 | 5.00 | 6.01 | 5.24 | 18.82 | 17.36 | 22.58 | 18.61 | 13.97 | 20.16 | 21.42 |
| $\lambda$ | 46.11 | 43.48 | 44.29 | 46.95 | 30.34 | 44.12 | 43.52 | 26.42 | 24.97 | 24.76 | 19.99 | 23.91 | 25.98 | 26.13 | 14.90 | 14.72 | 11.82 | 13.16 | 17.32 | 11.62 | 12.15 |

[1] R. Fabbri, "Time stability in human interaction networks," preprint arXiv:1310.7769. http://arxiv.org/abs/1310.7769.

[2] R. Fabbri, "What are you and i? [anthropological physics fundamentals]," (2015), https://www.academia.edu/10356773/What_are_you_and_I_anthropological_physics_fundamentals_.
